# Supplementary material for: Wavelet Integrated CNNs for Noise-Robust Image Classification
Source: arXiv:2005.03337 source file (2020-07-14)
Supplement: Supplementary file 1 [file supplementary_material_-_compete_version.tex]

\section*{Supplementary materials for ``Wavelet Integrated CNNs for Noise-Robust Image Classification''}\label{APP_wavelet}
\subsection*{A. Wavelets}
\begin{table*}
	\scriptsize
	\caption{Low-pass filters of the Daubechies wavelets.}
	\label{Tab_Daubechies_banks}
	\begin{center}
	\setlength{\tabcolsep}{1mm}{
	\begin{tabular}{c|cccccc}
		\hline
		          $p$           &     $1$      &       $2$       &         $3$         &         $4$         &         $5$         &         $6$         \\ \hline
		\multirow{12}{*}{$l_k$} &     $1$      &  $1+\sqrt{3}$   & $~~~0.332670552950$ & $~~~0.230377813309$ & $~~~0.160102397974$ & $~~~0.111540743350$ \\
		                        &     $1$      &  $3+\sqrt{3}$   & $~~~0.806891509311$ & $~~~0.714846570553$ & $~~~0.603829269797$ & $~~~0.494623890398$ \\
		                        &              &  $3-\sqrt{3}$   & $~~~0.459877502118$ & $~~~0.630880767930$ & $~~~0.724308528438$ & $~~~0.751133908021$ \\
		                        &              &  $1-\sqrt{3}$   &  $-0.135011020010$  &  $-0.027983769417$  & $~~~0.138428145901$ & $~~~0.315250351709$ \\
		                        &              &                 &  $-0.085441273882$  &  $-0.187034811719$  &  $-0.242294887066$  &  $-0.226264693965$  \\
		                        &              &                 & $~~~0.035226291886$ & $~~~0.030841381836$ &  $-0.032244869585$  &  $-0.129766867567$  \\
		                        &              &                 &                     & $~~~0.032883011667$ & $~~~0.077571493840$ & $~~~0.097501605587$ \\
		                        &              &                 &                     &  $-0.010597401785$  &  $-0.006241490213$  & $~~~0.027522865530$ \\
		                        &              &                 &                     &                     &  $-0.012580751999$  &  $-0.031582039317$  \\
		                        &              &                 &                     &                     & $~~~0.003335725285$ & $~~~0.000553842201$ \\
		                        &              &                 &                     &                     &                     & $~~~0.004777257511$ \\
		                        &              &                 &                     &                     &                     &  $-0.001077301085$  \\ \hline
		       $\text{factor}$         & $1/\sqrt{2}$ & $1/(4\sqrt{2})$ &         $1$         &         $1$         &         $1$         &         $1$         \\ \hline
	\end{tabular}}
	\end{center}
\end{table*}
\begin{table*}
\scriptsize
\caption{Low-pass filters of the Cohen wavelets.}
\label{Tab_CDF_banks}
\begin{center}
	\setlength{\tabcolsep}{0.5mm}{
		\begin{tabular}{c|cc|cc|cc|cc}
			\hline
			$(p,\tilde{p})$     & \multicolumn{2}{|c|}{$(2,2)$}       & \multicolumn{2}{|c|}{$(3,3)$}       & \multicolumn{2}{|c|}{$(4,4)$}          & \multicolumn{2}{|c}{$(5,5)$}           \\ \hline
			banks          & $\textbf{l}$ & $\tilde{\textbf{l}}$ & $\textbf{l}$ & $\tilde{\textbf{l}}$ &  $\textbf{l}$   & $\tilde{\textbf{l}}$ &  $\textbf{l}$   & $\tilde{\textbf{l}}$ \\ \hline
			\multirow{12}{*}{$l_k$} &     $0$      &         $0$          &     $0$      &   $~~~0.06629126$    &       $0$       &         $0$          & $~~~0.01345671$ &         $0$          \\
			& $0.35355339$ &    $-0.17677670$     &     $0$      &    $-0.19887378$     &  $-0.06453888$  &   $~~~0.03782846$    &  $-0.00269497$  &         $0$          \\
			& $0.70710678$ &   $~~~0.35355339$    & $0.17677670$ &    $-0.15467961$     &  $-0.04068942$  &    $-0.02384947$     &  $-0.13670658$  &   $~~~0.03968709$    \\
			& $0.35355339$ &   $~~~1.06066017$    & $0.53033009$ &   $~~~0.99436891$    & $~~~0.41809227$ &    $-0.11062440$     &  $-0.09350470$  &   $~~~0.00794811$    \\
			&     $0$      &   $~~~0.35355339$    & $0.53033009$ &   $~~~0.99436891$    & $~~~0.78848562$ &   $~~~0.37740286$    & $~~~0.47680327$ &    $-0.05446379$     \\
			&     $0$      &    $-0.17677670$     & $0.17677670$ &    $-0.15467961$     & $~~~0.41809227$ &   $~~~0.85269868$    & $~~~0.89950611$ &   $~~~0.34560528$    \\
			&              &                      &     $0$      &    $-0.19887378$     &  $-0.04068942$  &   $~~~0.37740286$    & $~~~0.47680327$ &   $~~~0.73666018$    \\
			&              &                      &     $0$      &   $~~~0.06629126$    &  $-0.06453888$  &    $-0.11062440$     &  $-0.09350470$  &   $~~~0.34560528$    \\
			&              &                      &              &                      &       $0$       &    $-0.02384947$     &  $-0.13670658$  &    $-0.05446379$     \\
			&              &                      &              &                      &       $0$       &   $~~~0.03782846$    &  $-0.00269497$  &   $~~~0.00794811$    \\
			&              &                      &              &                      &                 &                      & $~~~0.01345671$ &   $~~~0.03968709$    \\
			&              &                      &              &                      &                 &                      &       $0$       &         $0$          \\ \hline
	\end{tabular}}
\end{center}
\end{table*}
Wavelet is associated with scaling function $\phi(x)$ and wavelet function $\psi(x)$
whose shifts and expansions compose stable basis for the signal space $L^2(x)$.
Using the basis, a signal can be decomposed and reconstructed.
Symmetric wavelet is with symmetric scaling function and symmetric/antisymmetric wavelet function,
i.e., $\exists~a_0, a_1$ for $\forall~x$ satisfies $\phi(x) = \phi(x+a_0)$ and $\psi(x) = \pm\psi(x+a_1)$.
The scaling function and wavelet function are closely related with the low-pass filter $\textbf{l}$ and high-pass filter $\textbf{h}$.
In practice, the filters are applied for the signal decomposition and reconstruction, as Eqs. (\ref{eq_DWT}) and (\ref{eq_IDWT}) show.
$\phi(x), \psi(x)$ are symmetric/antisymmetric if and only if $\textbf{l}, \textbf{h}$ are symmetric/antisymmetric.
It is not possible for any orthogonal wavelet with finite filters to be symmetric, except for the Haar wavelet.

\textbf{Orthogonal wavelets}\label{APP_ortho_wavelet}\quad
Daubechies wavelets are orthogonal.
Table \ref{Tab_Daubechies_banks} shows the low-pass filter $\textbf{l} = \{l_k\}$ of the wavelets with order $p, 1\leq p\leq6$.
The length of the filter is $2p$.
The high-pass filter $\textbf{h} = \{h_k\}$ can be deduced from
\begin{equation}\label{eq_high_pass_bank}
h_k = (-1)^k l_{N-k},
\end{equation}
where $N$ is an odd number.
Daubechies(1) is Haar wavelet.

\textbf{Biorthogonal wavelets}\label{APP_bior_wavelet}\quad
Cohen wavelets are symmetric biorthogonal wavelets,
and each of them is with scaling function $\phi$, wavelet function $\psi$, and their dual functions $\tilde{\phi}, \tilde{\psi}$.
Correspondingly, it has four filters $\textbf{l}$, $\textbf{h}$, $\tilde{\textbf{l}}$, and $\tilde{\textbf{h}}$.
While a signal is decomposed using filters $\textbf{l}$ and $\textbf{h}$,
it can be reconstructed using the dual filters $\tilde{\textbf{l}}$ and $\tilde{\textbf{h}}$.
Cohen wavelet is with two order parameters $p$ and $\tilde{p}$.
Table \ref{Tab_CDF_banks} shows the low-pass filters with orders $2\leq p = \tilde{p}\leq5$.
Their high-pass filters can be deduced from
\begin{eqnarray}\label{eq_high_pass_bank_bior}
&h_k = (-1)^k \tilde{l}_{N-k},&\\
&\tilde{h}_k = (-1)^k l_{N-k},&
\end{eqnarray}
where $N$ is an odd number.
Cohen$(1,1)$ is Haar wavelet.

Wavelet theory is valid for finite or infinite filters,
but the infinite case is rarely covered in practical interest.
Discrete Wavelet Transform (DWT) decomposes an image into its low-frequency and high-frequency components.
In theory, Inverse DWT (IDWT) could precisely reconstructs the image using the DWT output.
In practice, in our DWT and IDWT layers, we truncate \textbf{L}, \textbf{H} to fit the image with finite size.
As a result, IDWT with asymmetric wavelet can not fully restore the image in the region near the image boundary,
and the region width increases as the wavelet filter length increases.
With symmetric wavelet, however, one can fully restore the image based on symmetric extension of the DWT output.
In other words, the DWT output of symmetric wavelets save the fully information of the input image,
but that of asymmetric wavelets do not.
We believe that is the reason why asymmetric Daubechies wavelets perform worse
than symmetric Cohen and Haar wavelets in image classification of WaveCNets.

Our DWT and IDWT layers are applicable to any discrete orthogonal or biorthogonal wavelets.
Besides the othogonal and biorthogonal wavelets,
various wavelets and beyond-wavelets, including multi-wavelets, ridgelet, curvelet, bandelet, contourlet, dual-tree complex wavelet, etc.,
have been designed and studied, which have found many applications in signal processing, numerical analysis,
pattern recognition, computer vision, quantum mechanics, etc.
The DWT/IDWT layer could be applicable to these mathematical tools with slight modifications.

\subsection*{B. The application of DWT in suppressing aliasing effects in deep networks}
In deep networks, the down-sampling operations ignoring the classic sampling theorem introduce at least two drawbacks:
breaking basic object structures and accumulating noises in the feature maps.
These drawbacks are related with the aliasing introduced by the down-sampling,
and we call them \textbf{aliasing effects} in deep networks.

In WaveCNets, DWT is applied to maintain the basic object structures and resist the noise propagation,
for better accuracy and noise-robustness.
We have shown four example feature maps of well trained CNNs and WaveCNets in Fig. \ref{fig_feature_maps}.
To illustrate more persuasively the application of DWT in suppressing aliasing effects in deep networks,
Fig. \ref{fig_feature_maps_more_0} and Fig. \ref{fig_feature_maps_more_1} present more examples.
In each subfigure, the top row shows the input image with size of $224 \times 224$ from ImageNet validation set
and the two feature maps produced by original CNN,
while the bottom row shows the related information (image, CNN and WaveCNet names) and feature maps produced by the WaveCNet.
The two feature maps are captured from the 16th output channel of the final layer
in the network blocks with tensor size of $56 \times 56$ (middle) and $28 \times 28$ (right), respectively.
The feature maps have been enlarged for better illustration.

\begin{figure*}[!bpt]
	\centering
	\subfigure[]
	{\includegraphics*[scale=0.25, viewport=175 65 1025 575]{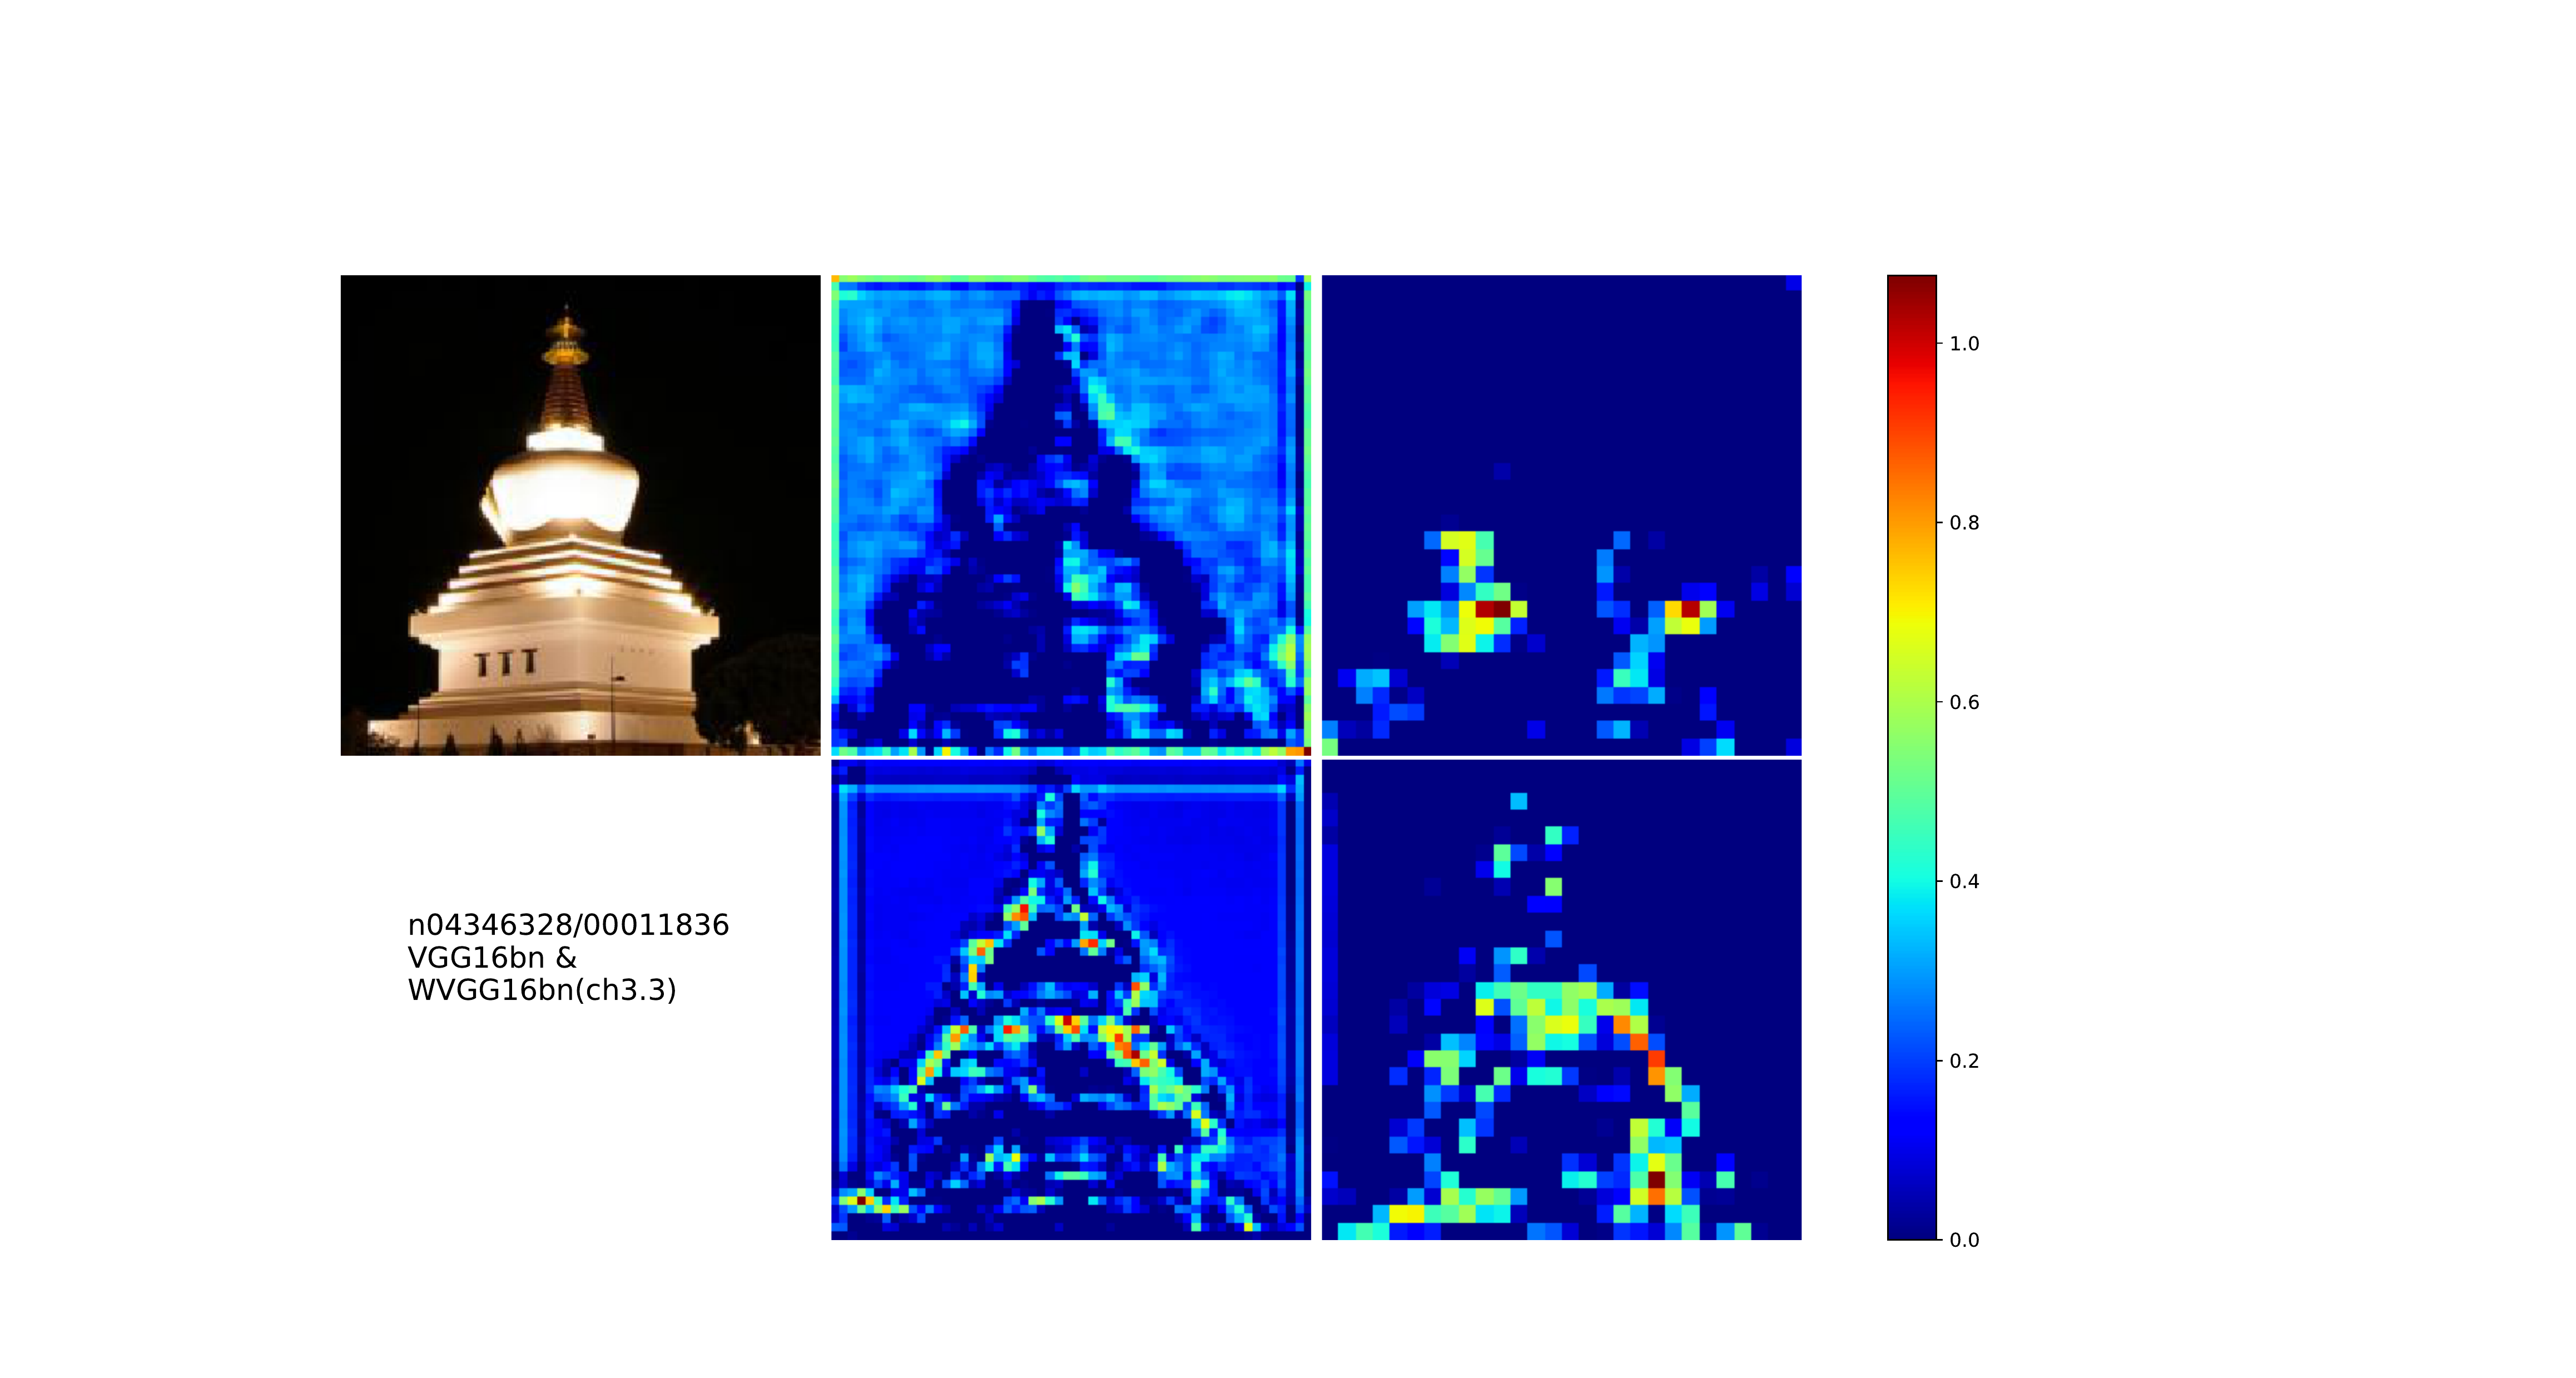}}\hspace{30pt}
	\subfigure[]
	{\includegraphics*[scale=0.25, viewport=175 65 1025 575]{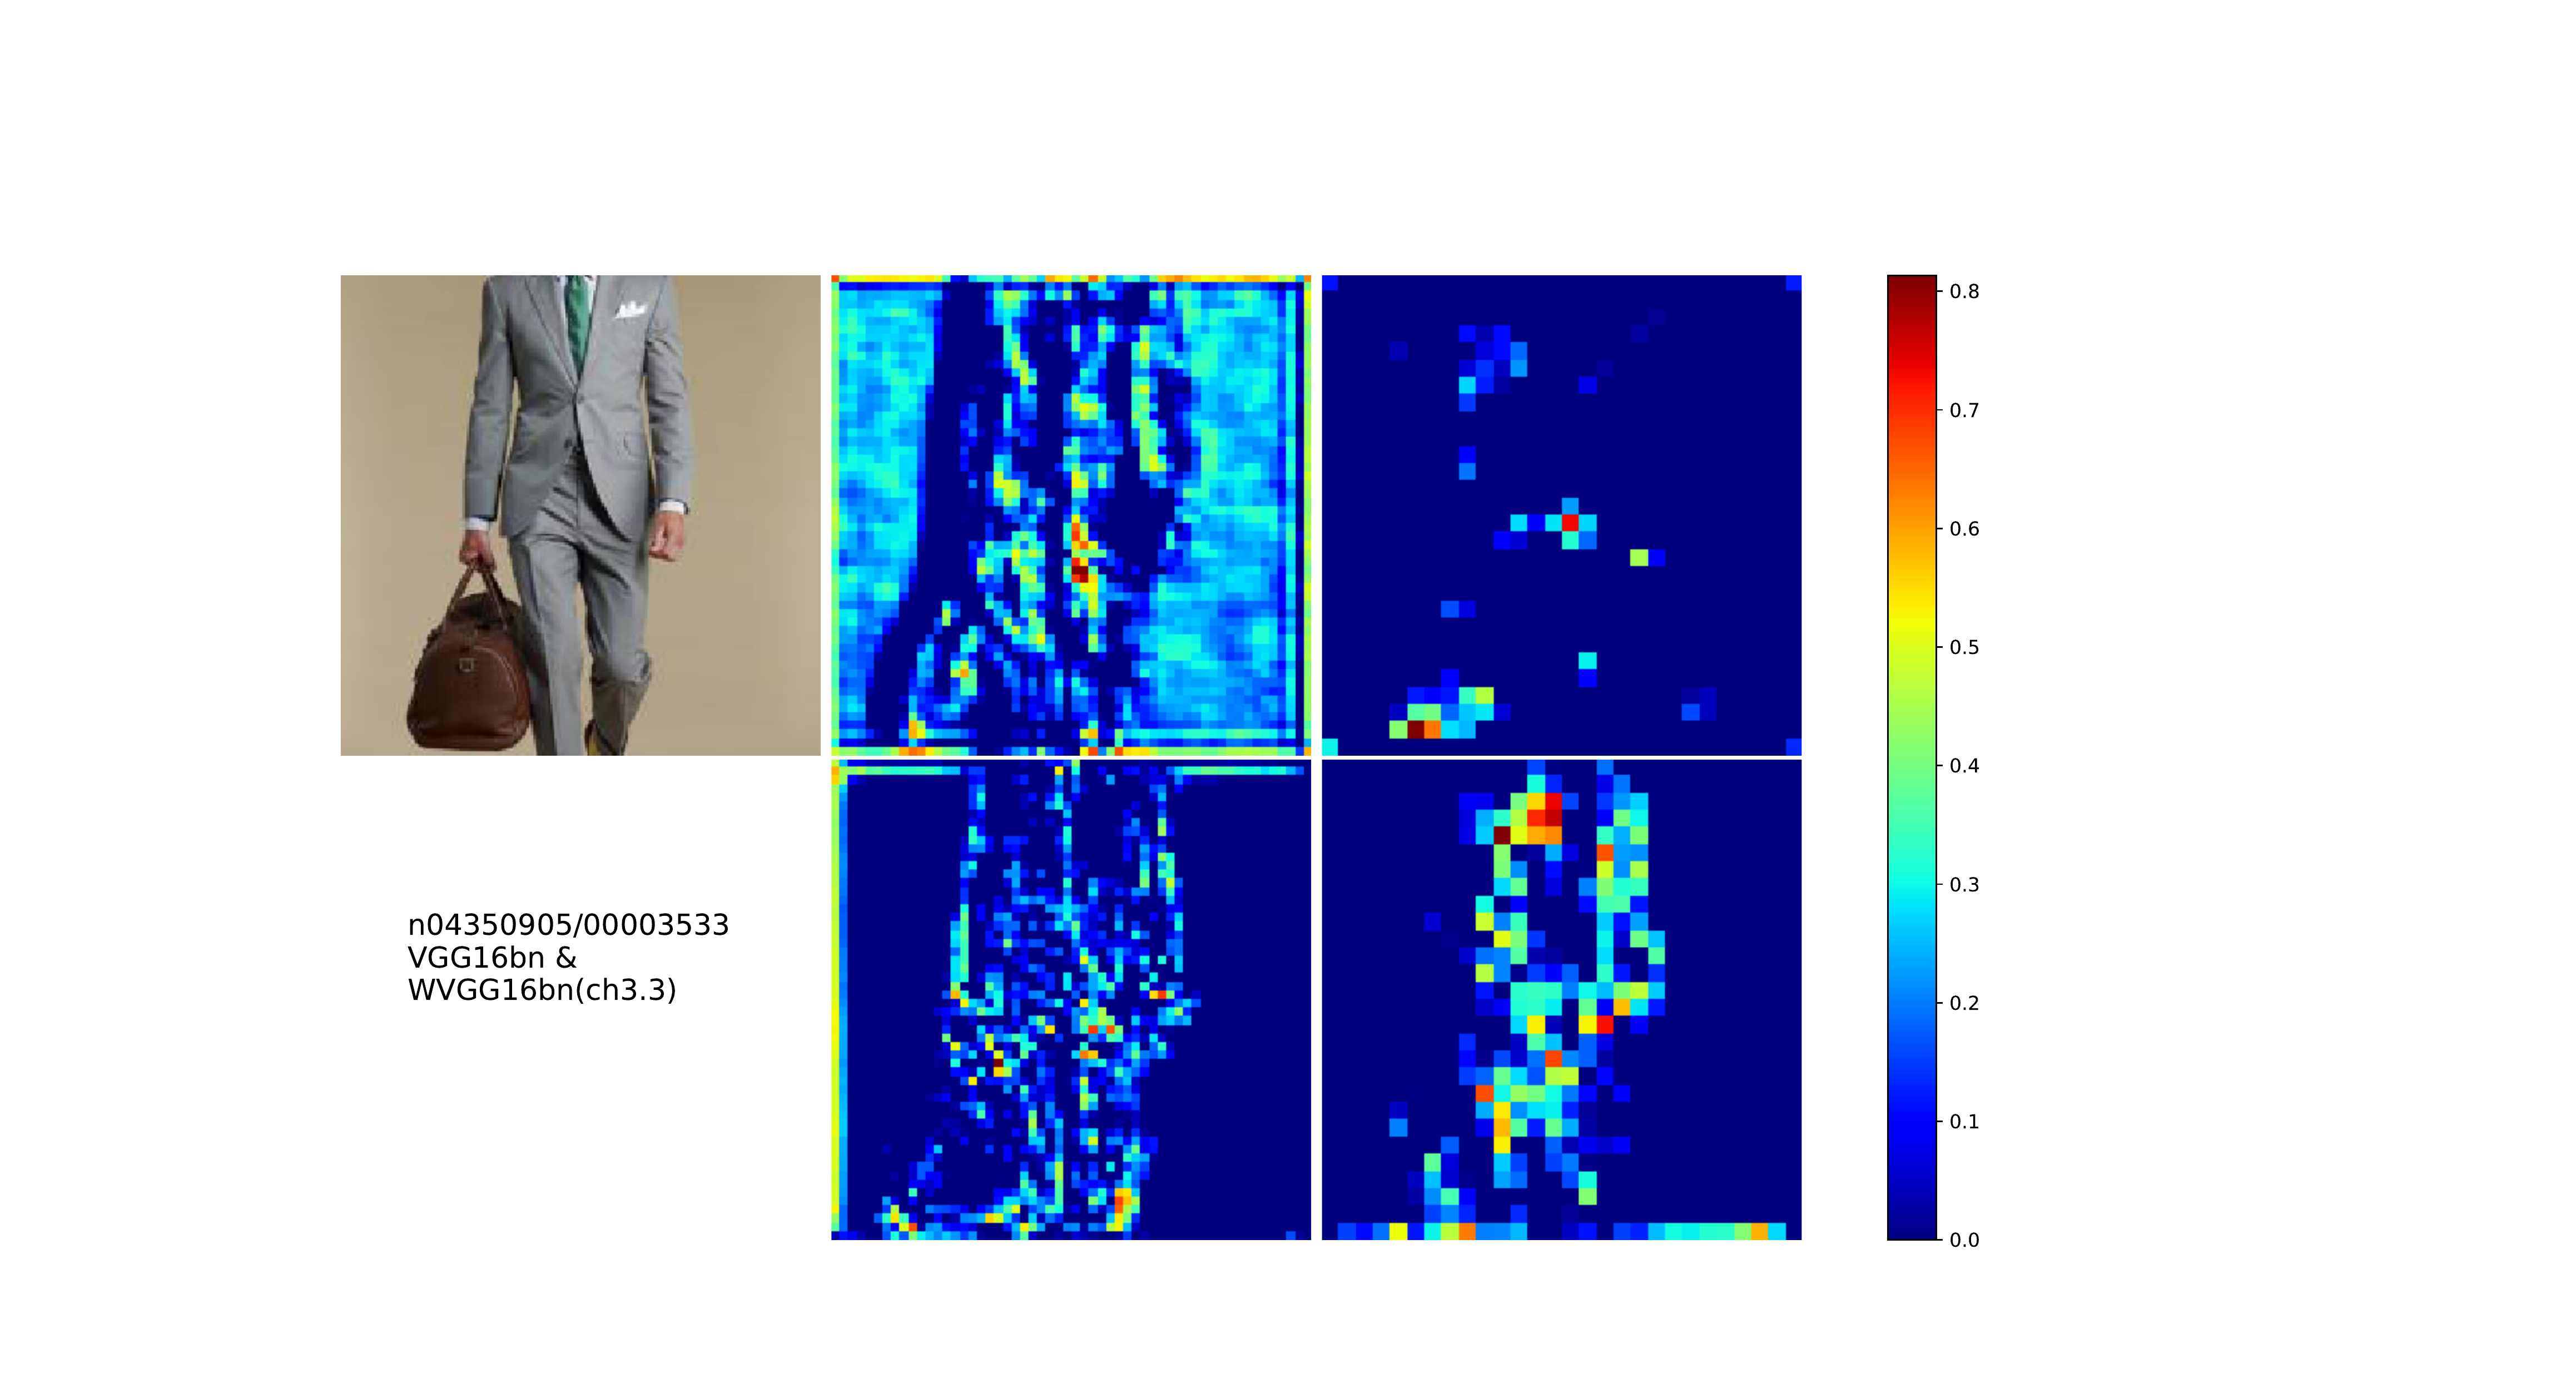}}\\
	\subfigure[]
	{\includegraphics*[scale=0.25, viewport=175 65 1025 575]{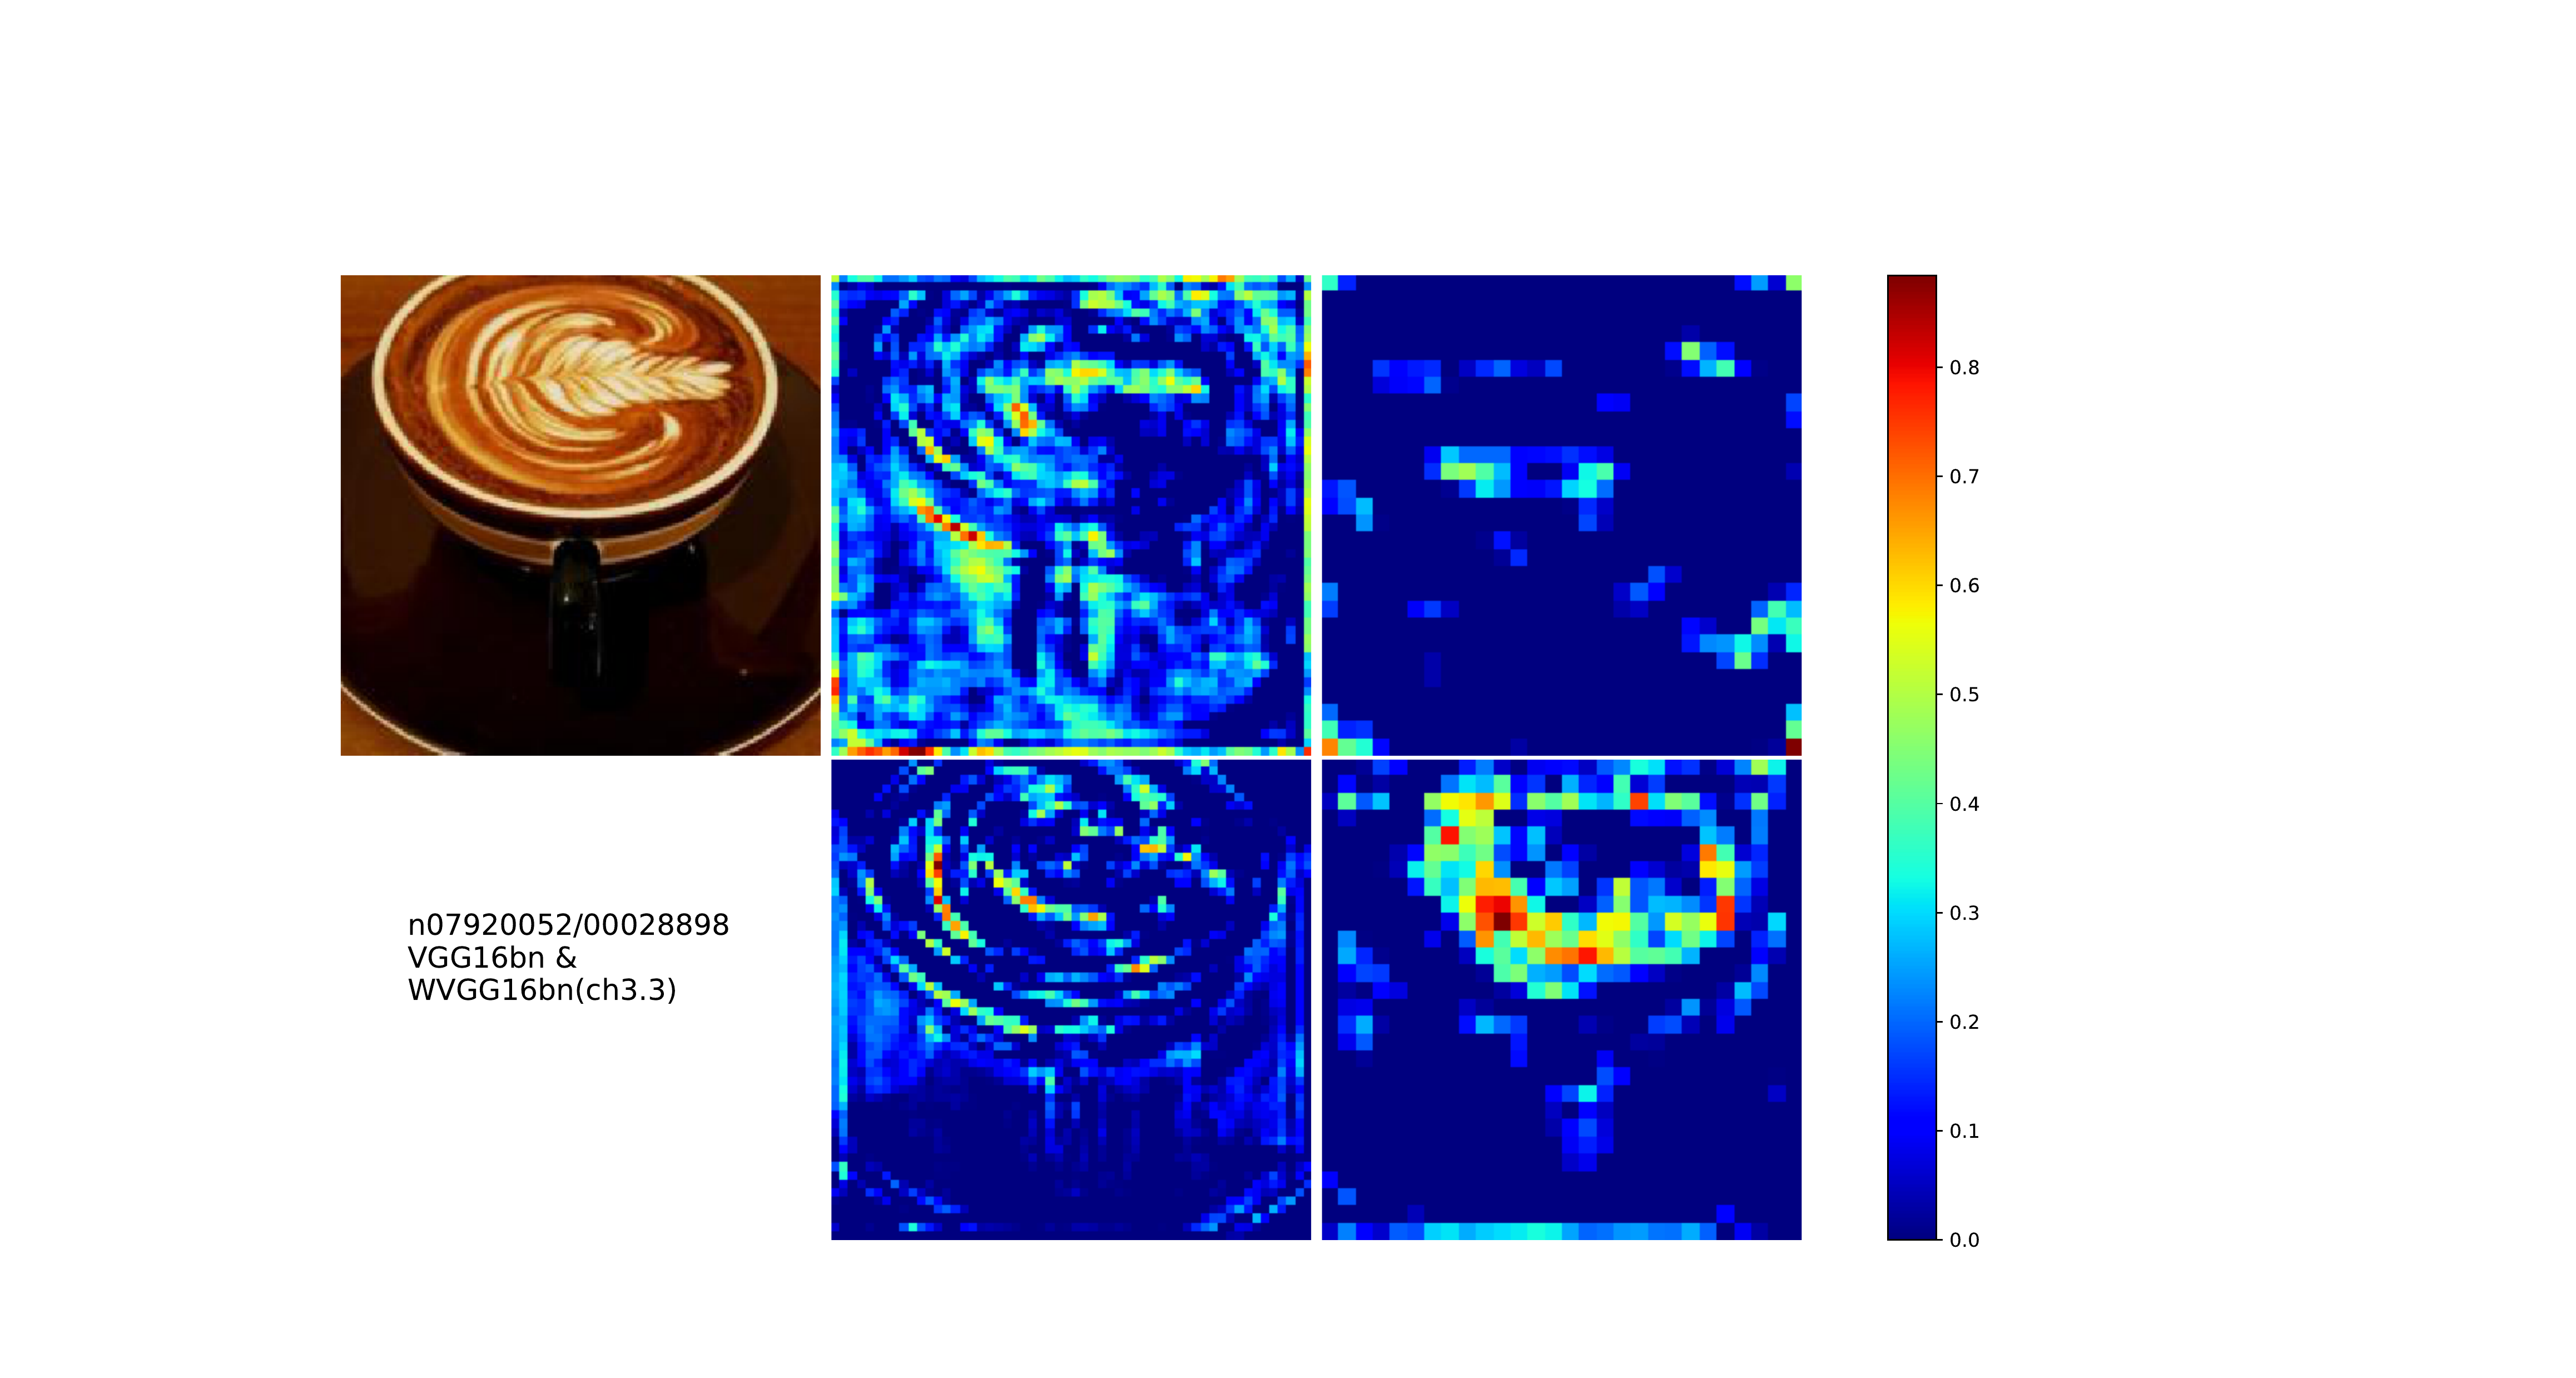}}\hspace{30pt}
	\subfigure[]
	{\includegraphics*[scale=0.25, viewport=175 65 1025 575]{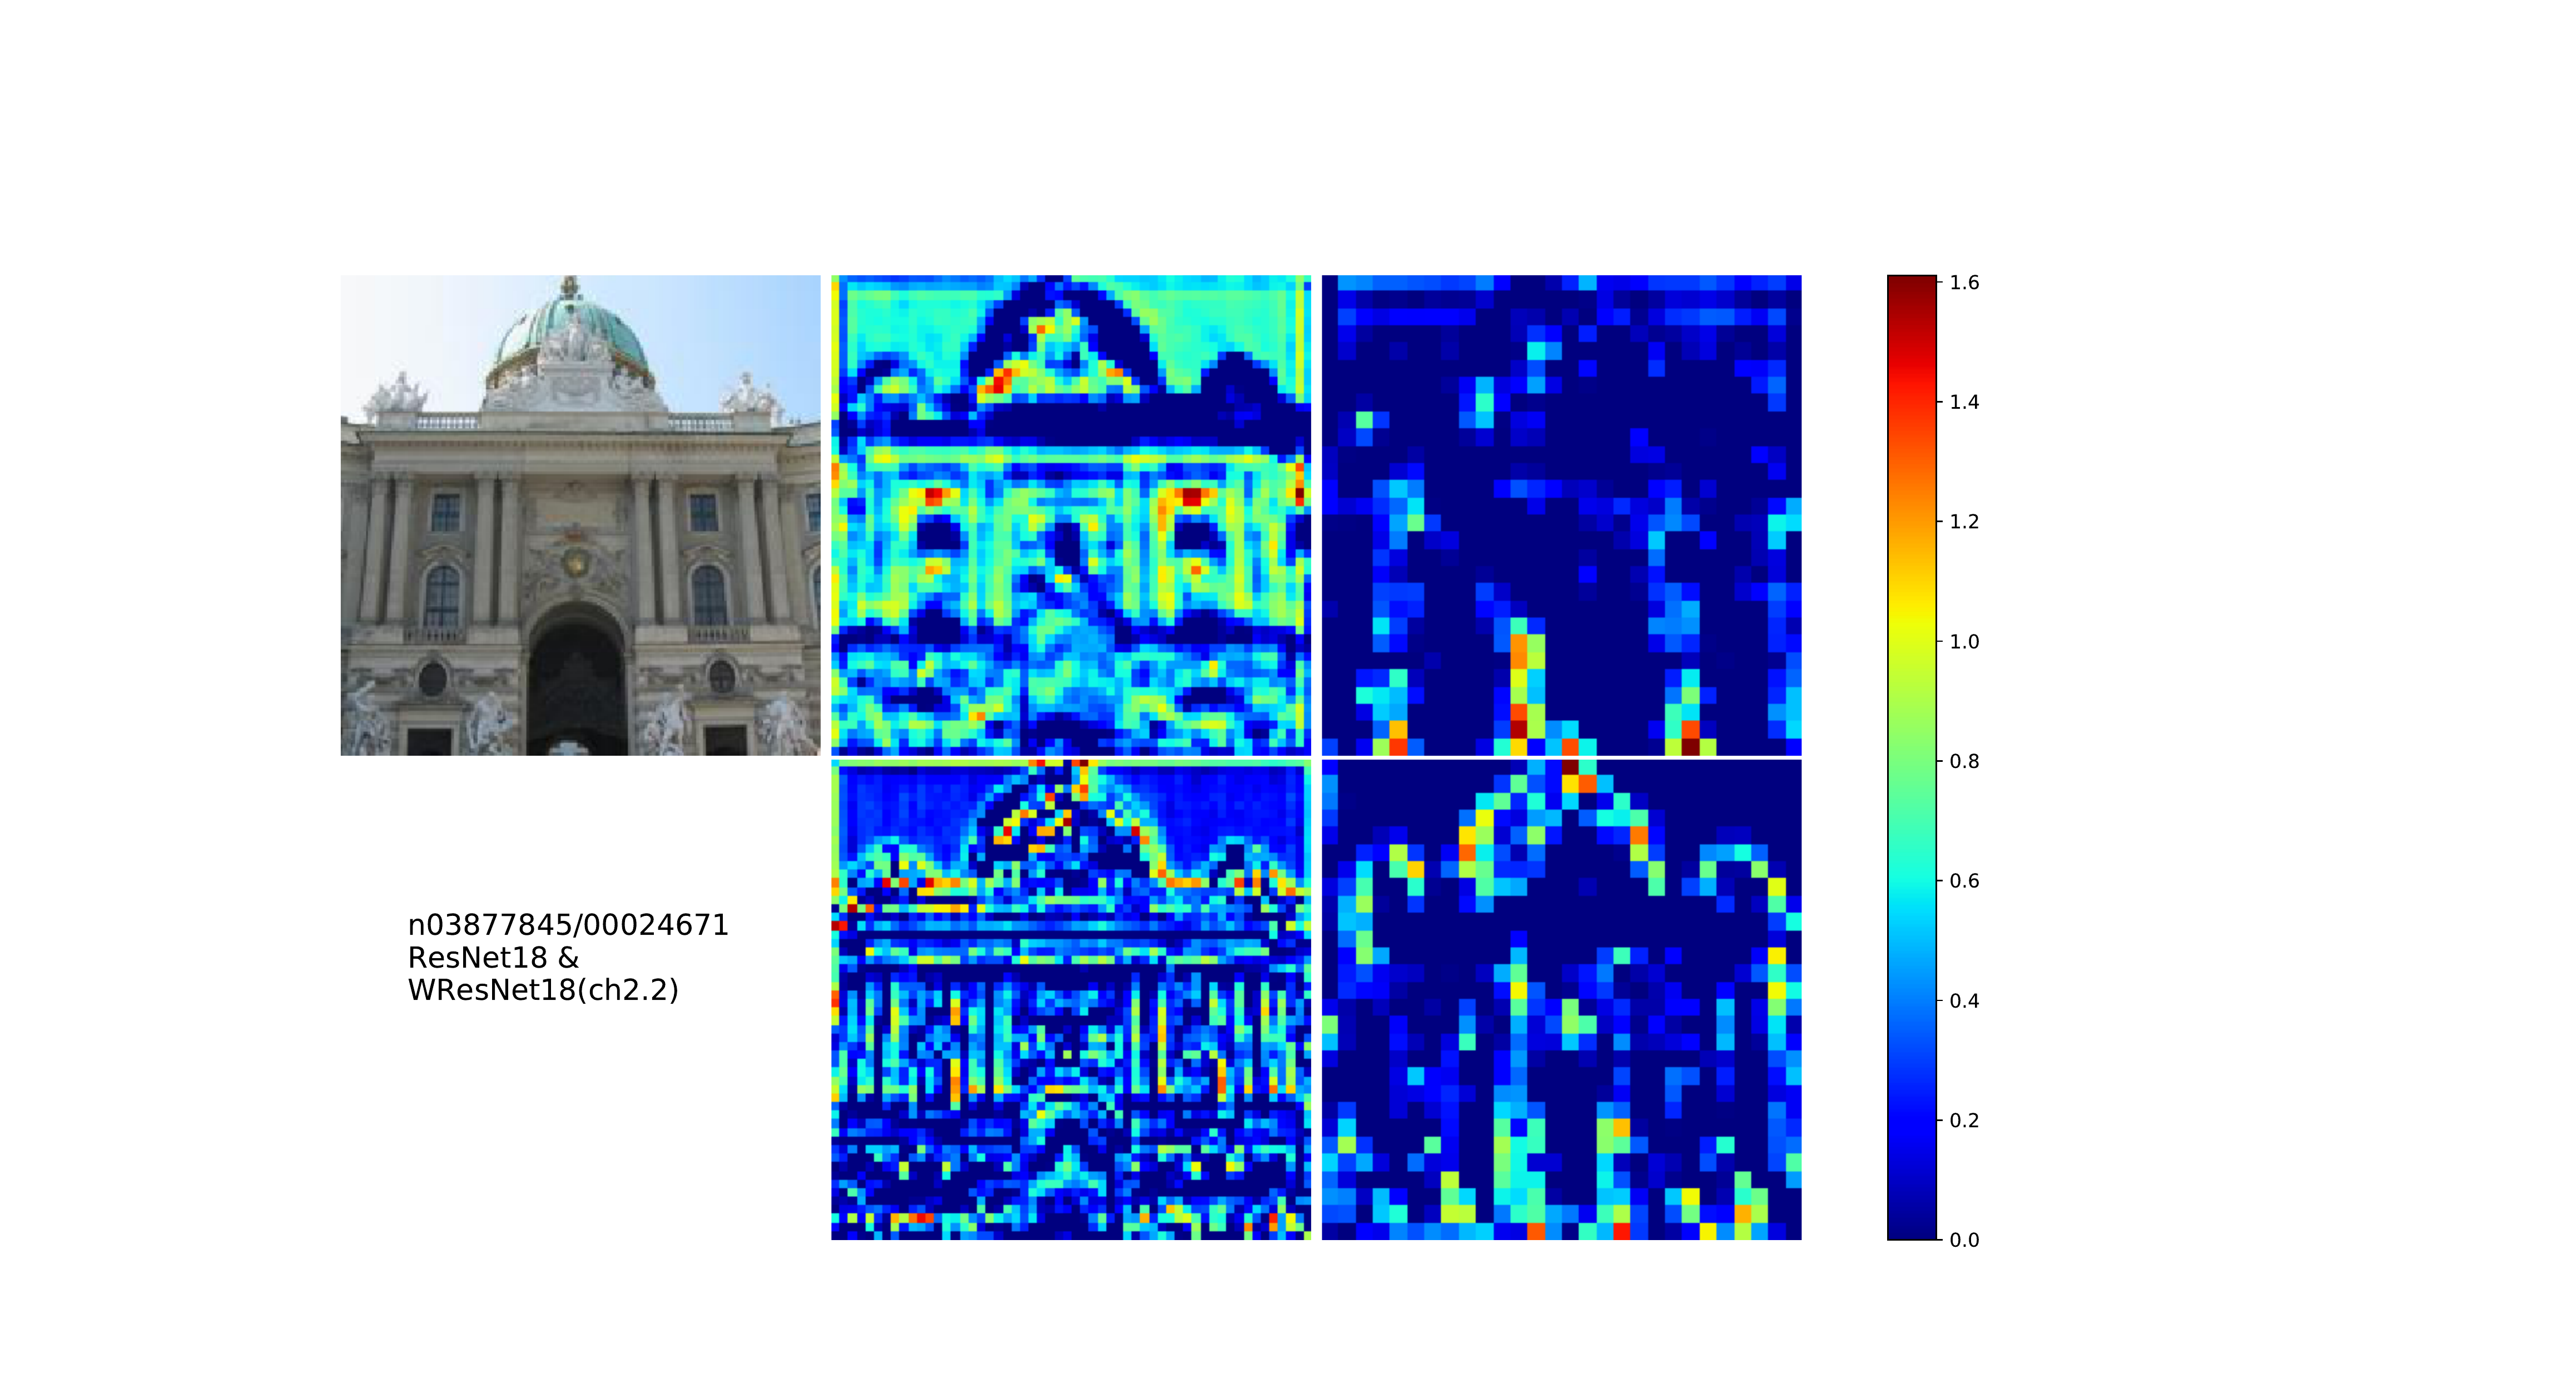}}\\
	\subfigure[]
	{\includegraphics*[scale=0.25, viewport=175 65 1025 575]{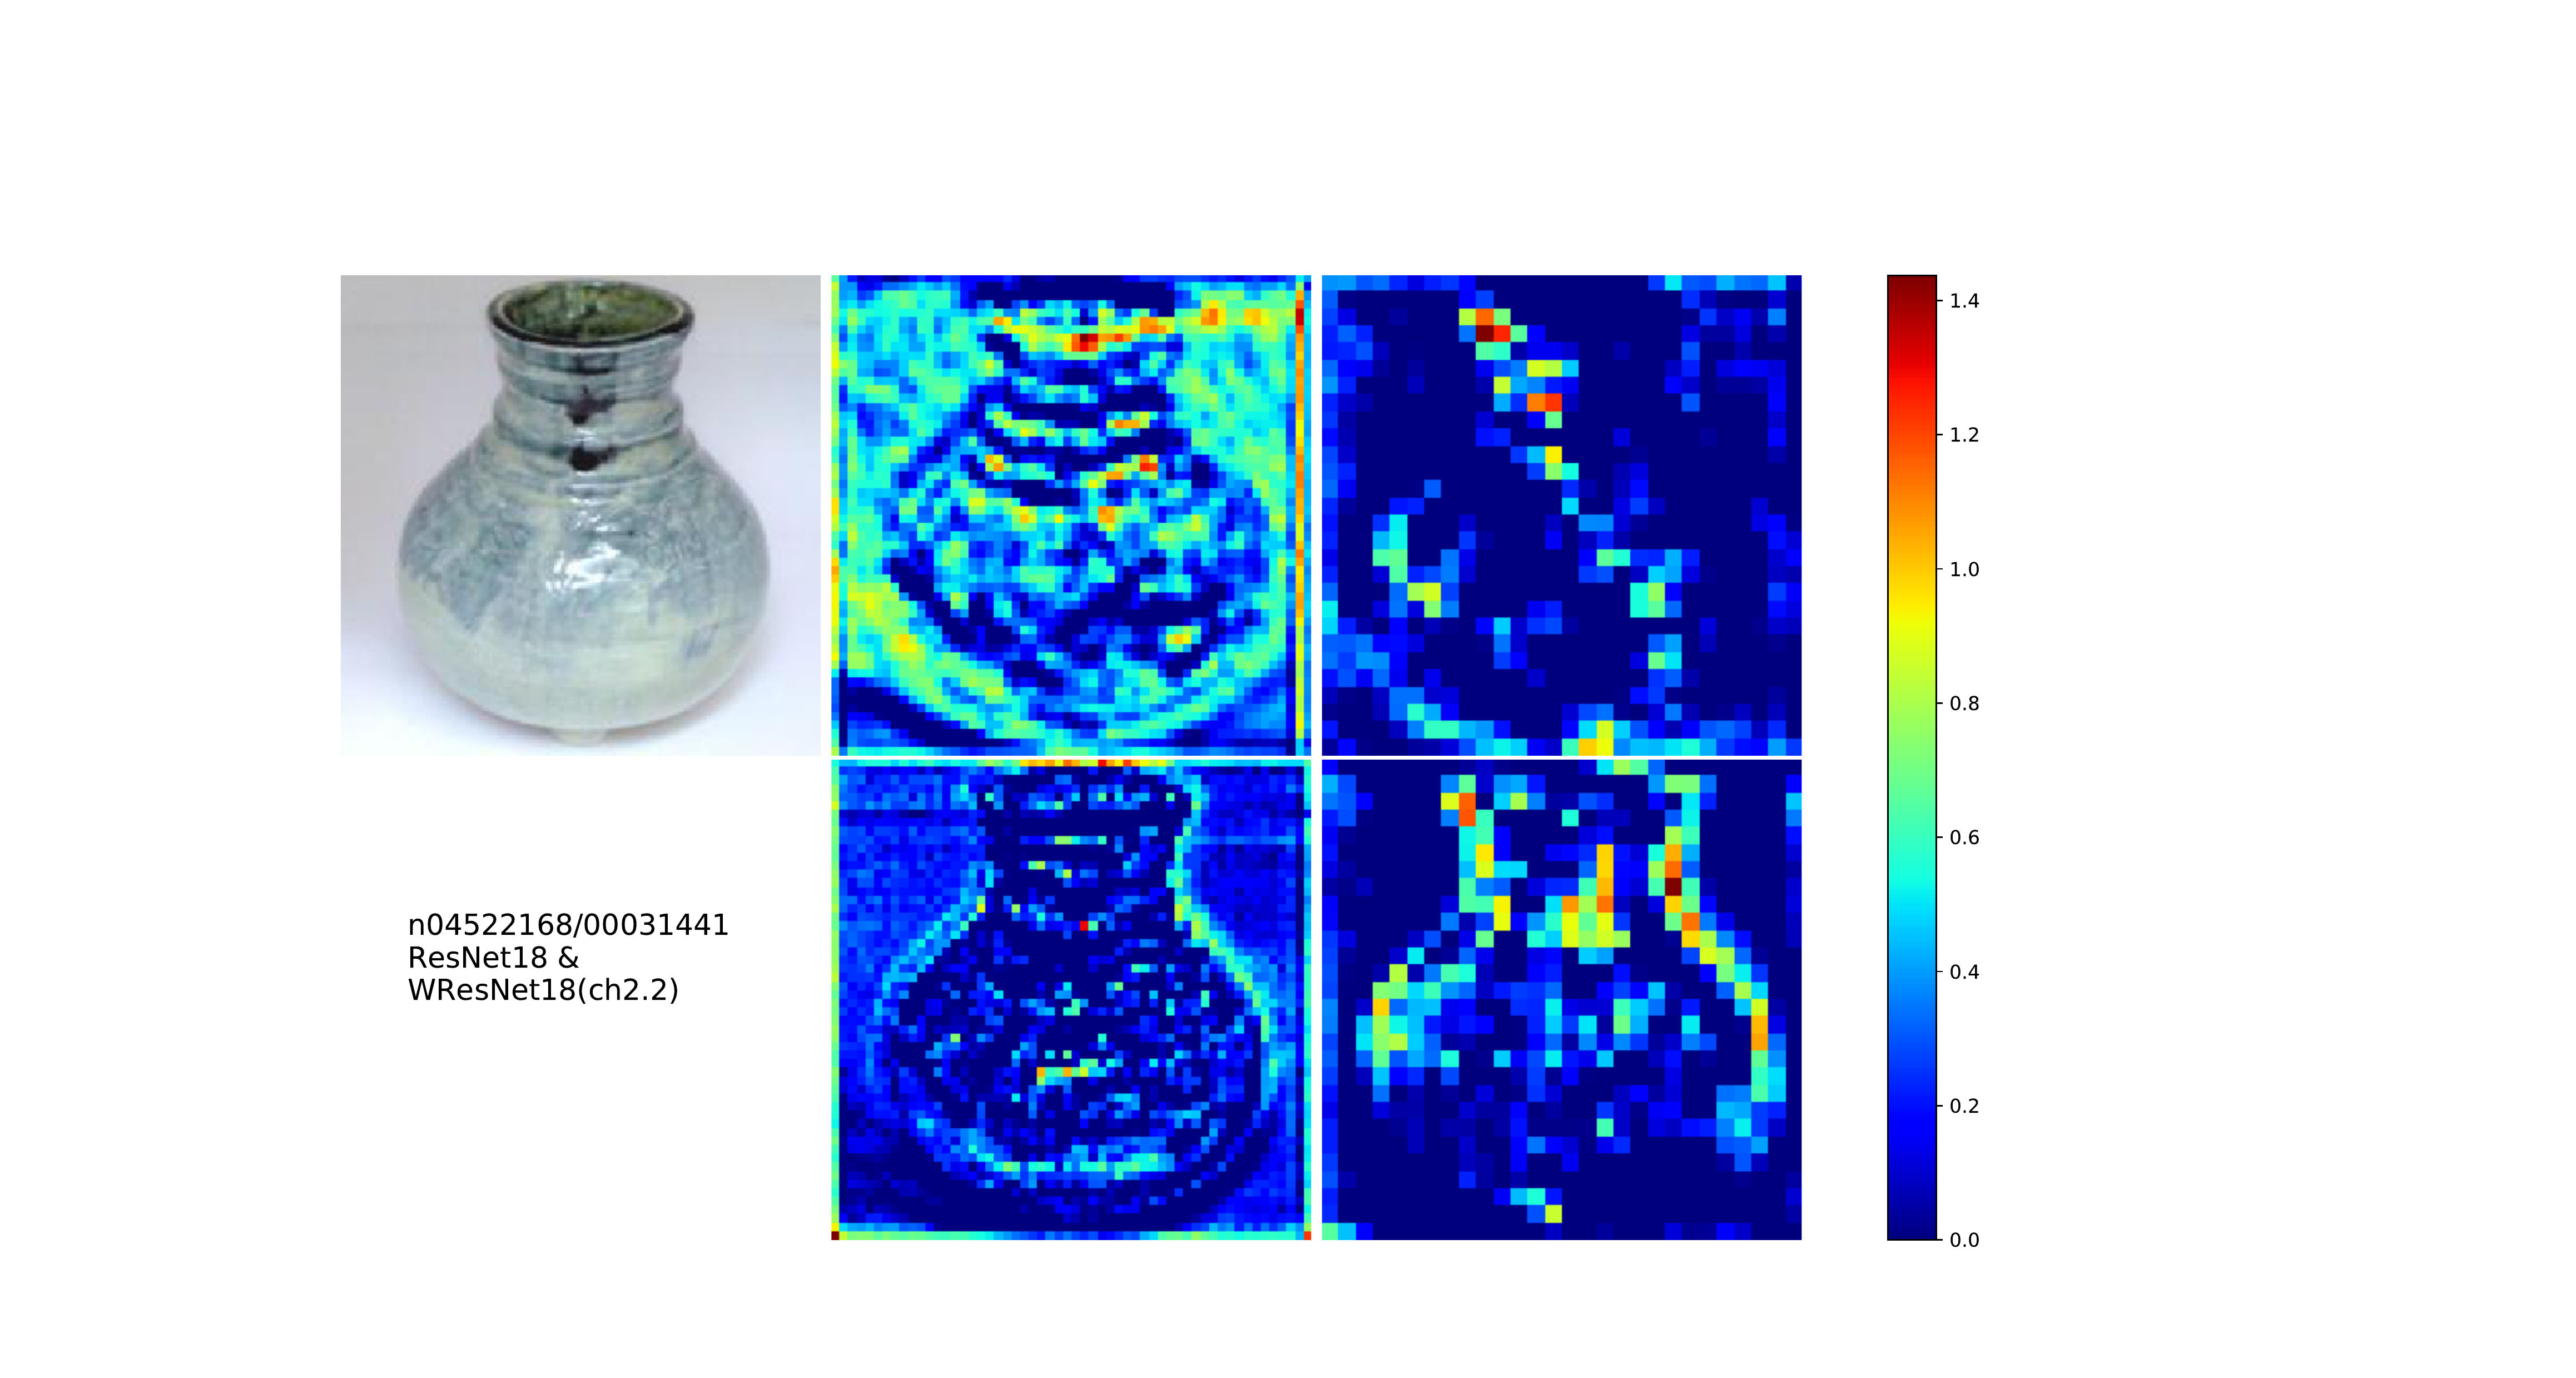}}\hspace{30pt}
	\subfigure[]
	{\includegraphics*[scale=0.25, viewport=175 65 1025 575]{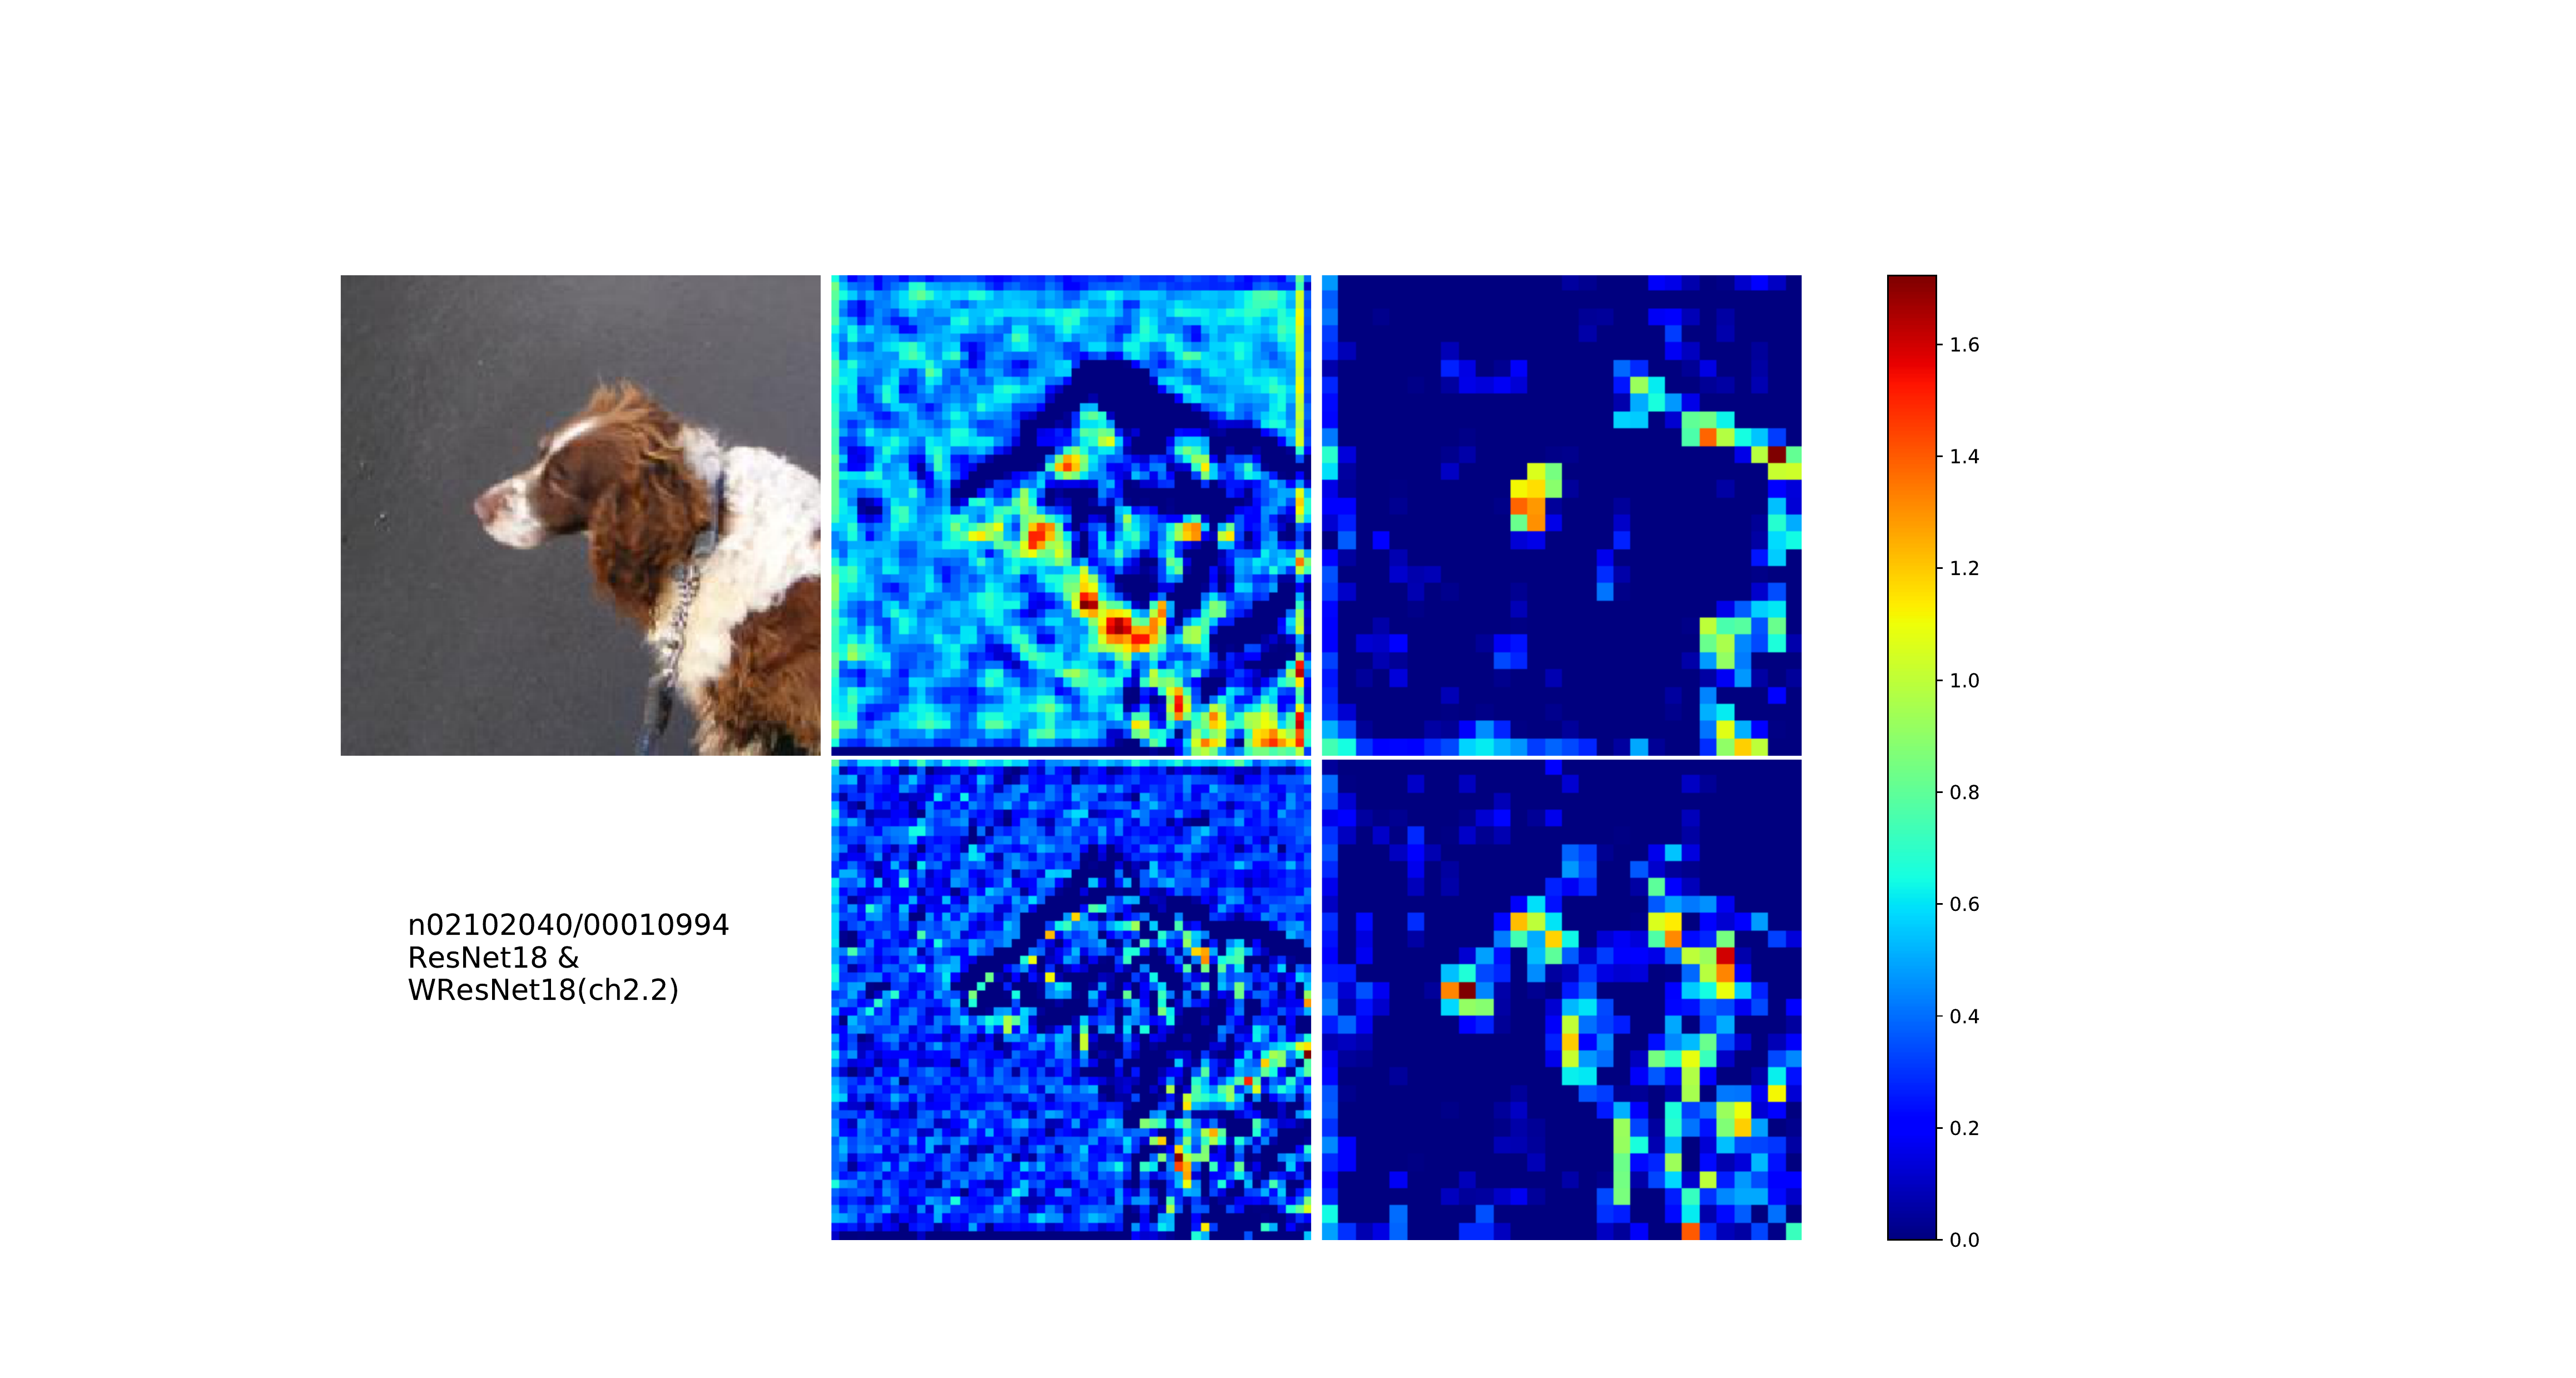}}\\
	\subfigure[]
	{\includegraphics*[scale=0.25, viewport=175 65 1025 575]{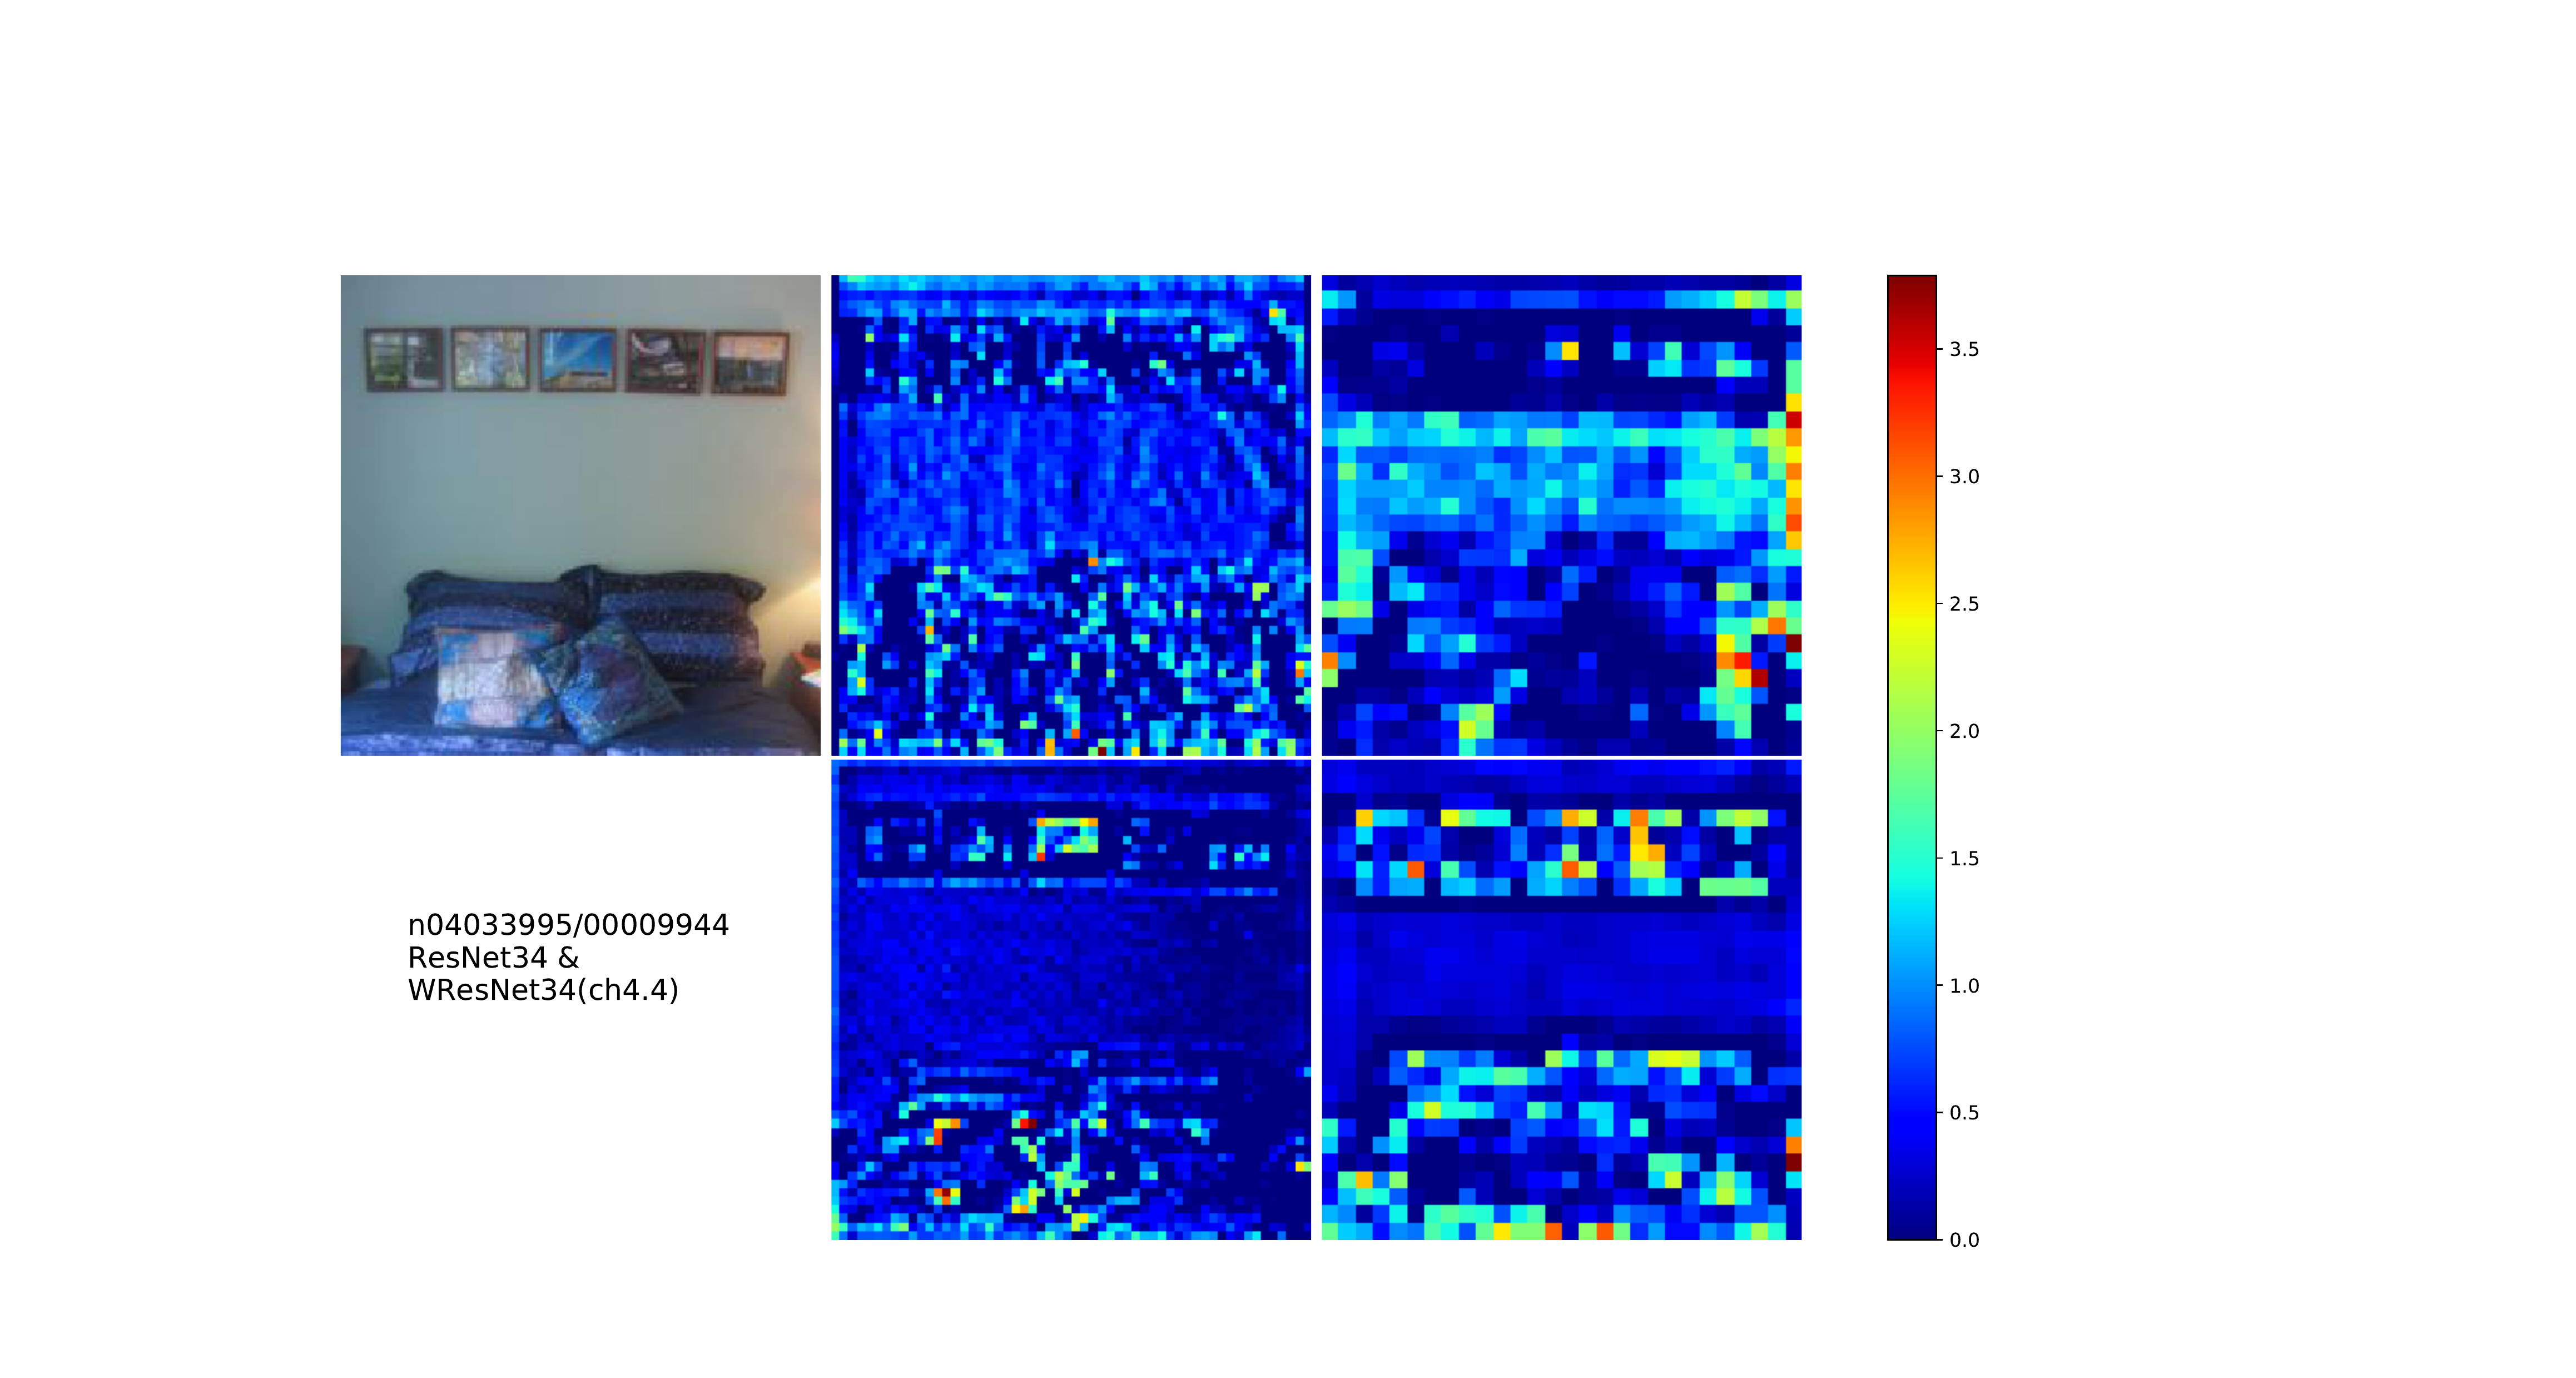}}\hspace{30pt}
	\subfigure[]
	{\includegraphics*[scale=0.25, viewport=175 65 1025 575]{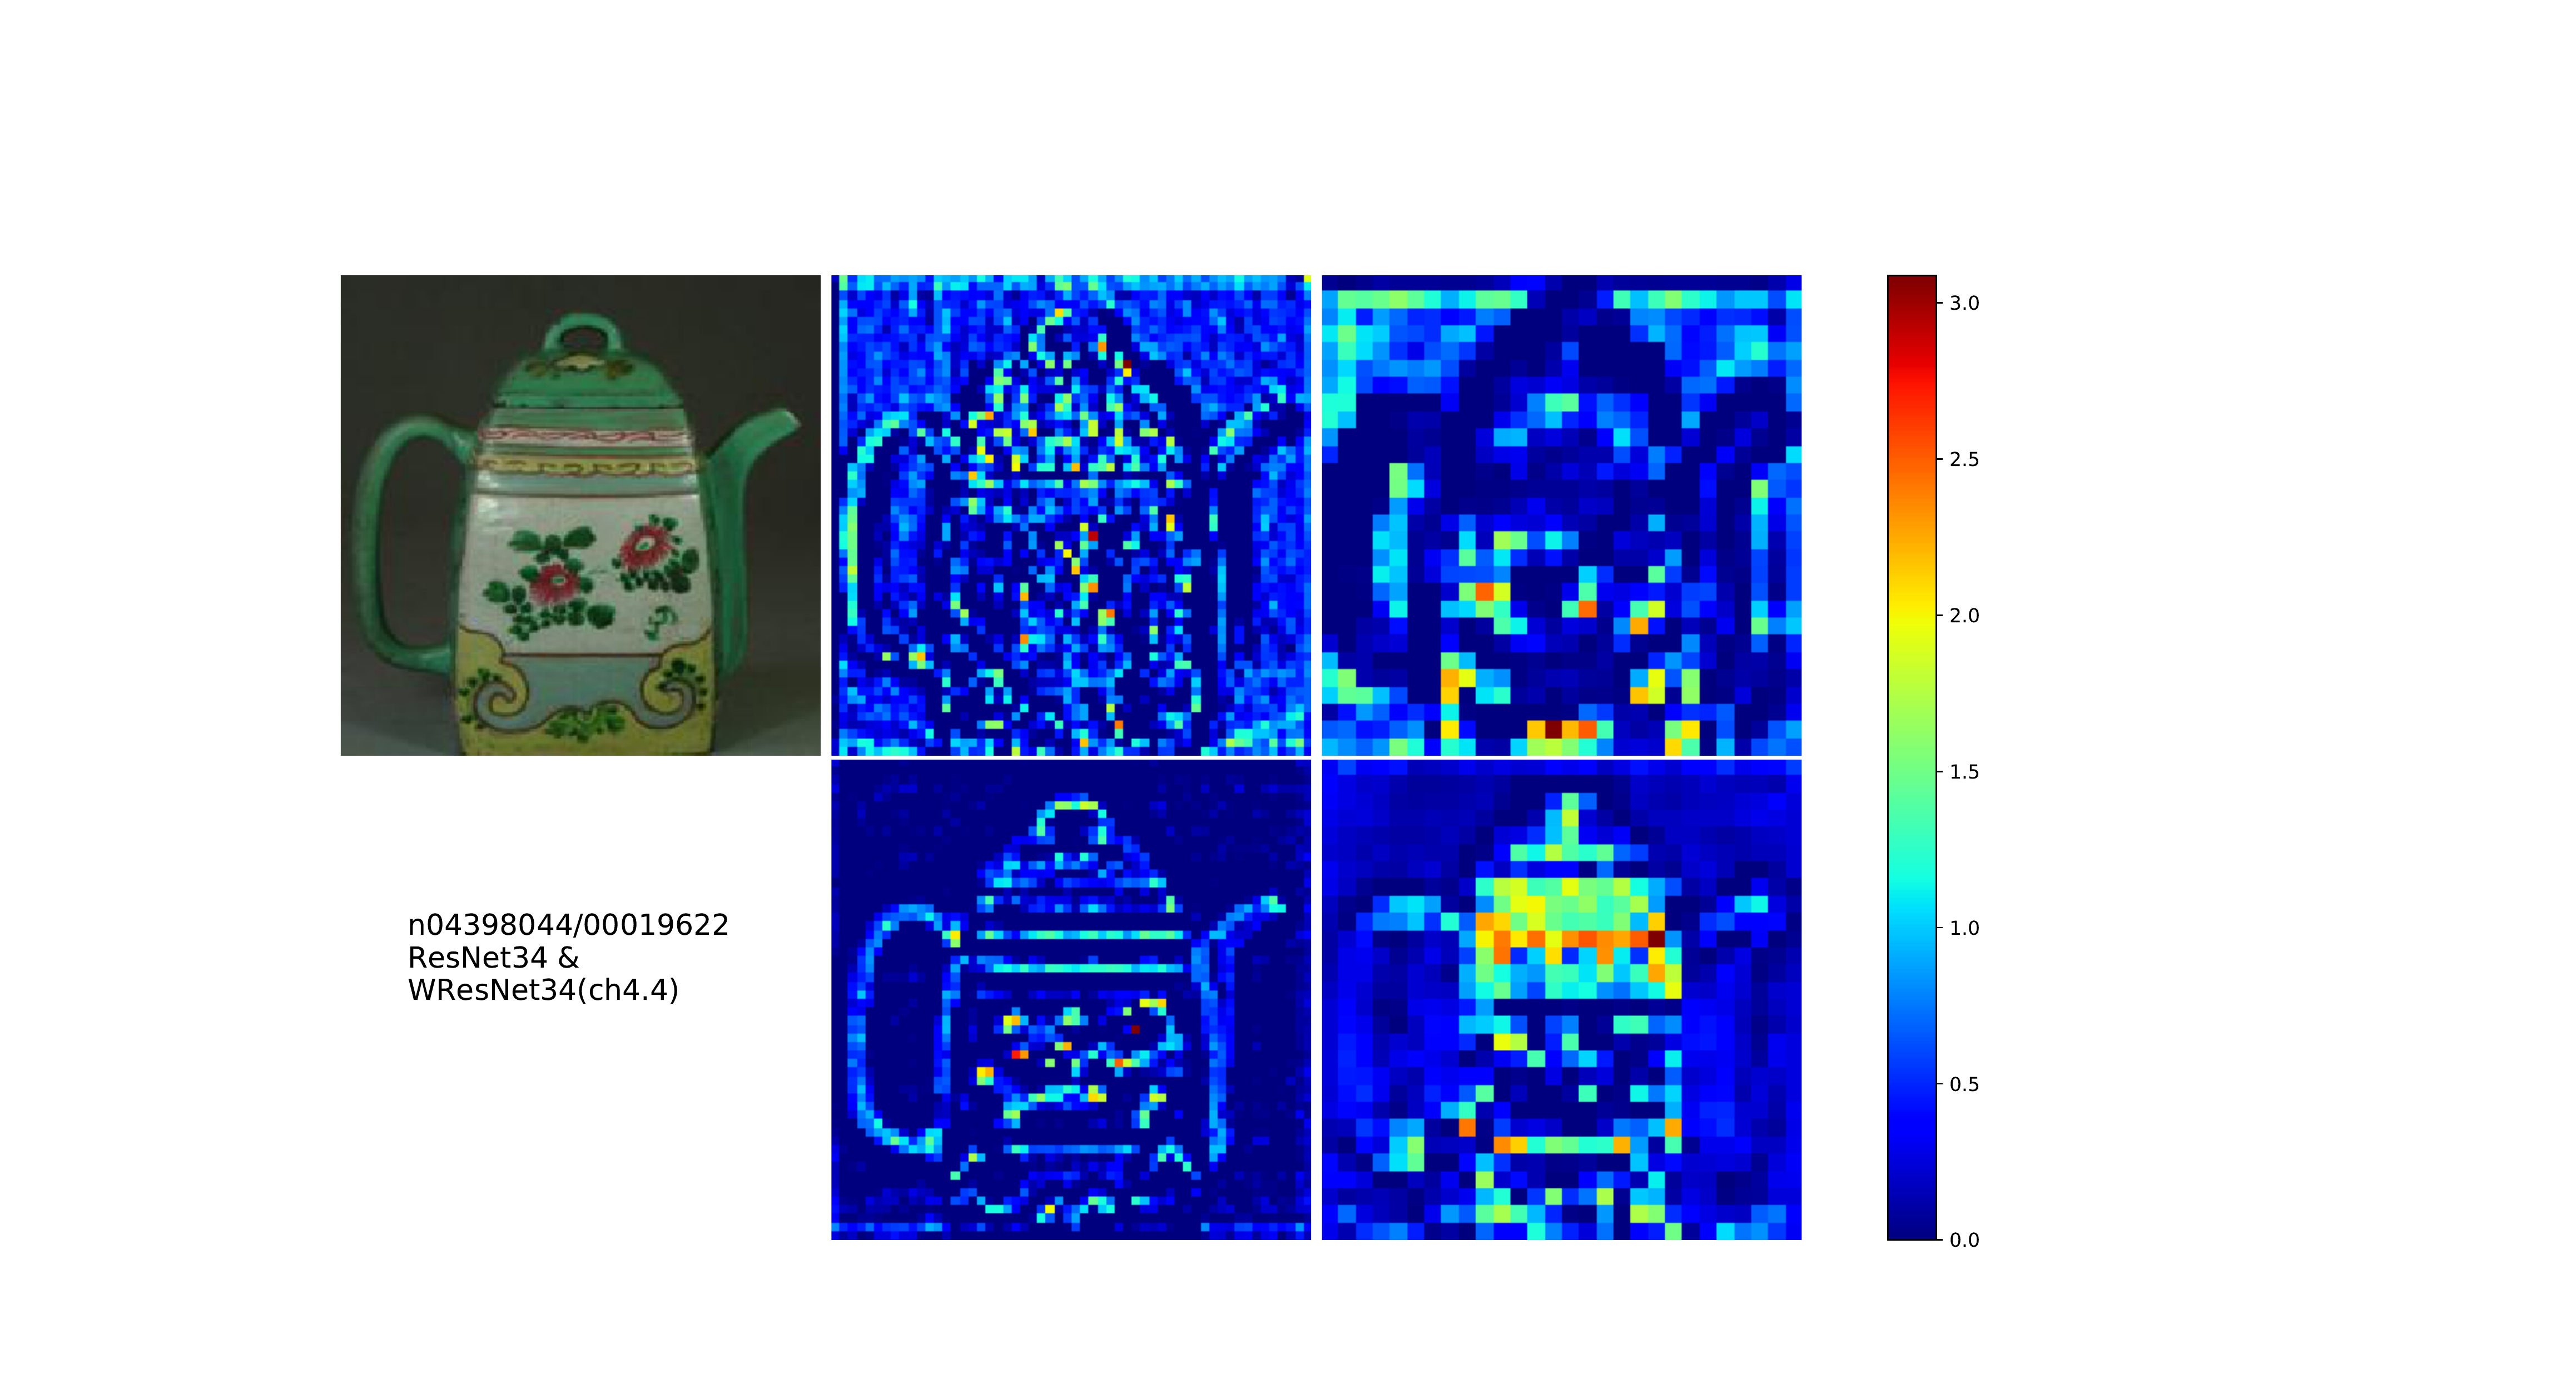}}
	\caption{The feature maps of CNNs (top) and WaveCNets (bottom).}
	\label{fig_feature_maps_more_0}
\end{figure*}
\begin{figure*}[!bpt]
	\centering
	\subfigure[]
	{\includegraphics*[scale=0.25, viewport=175 65 1025 575]{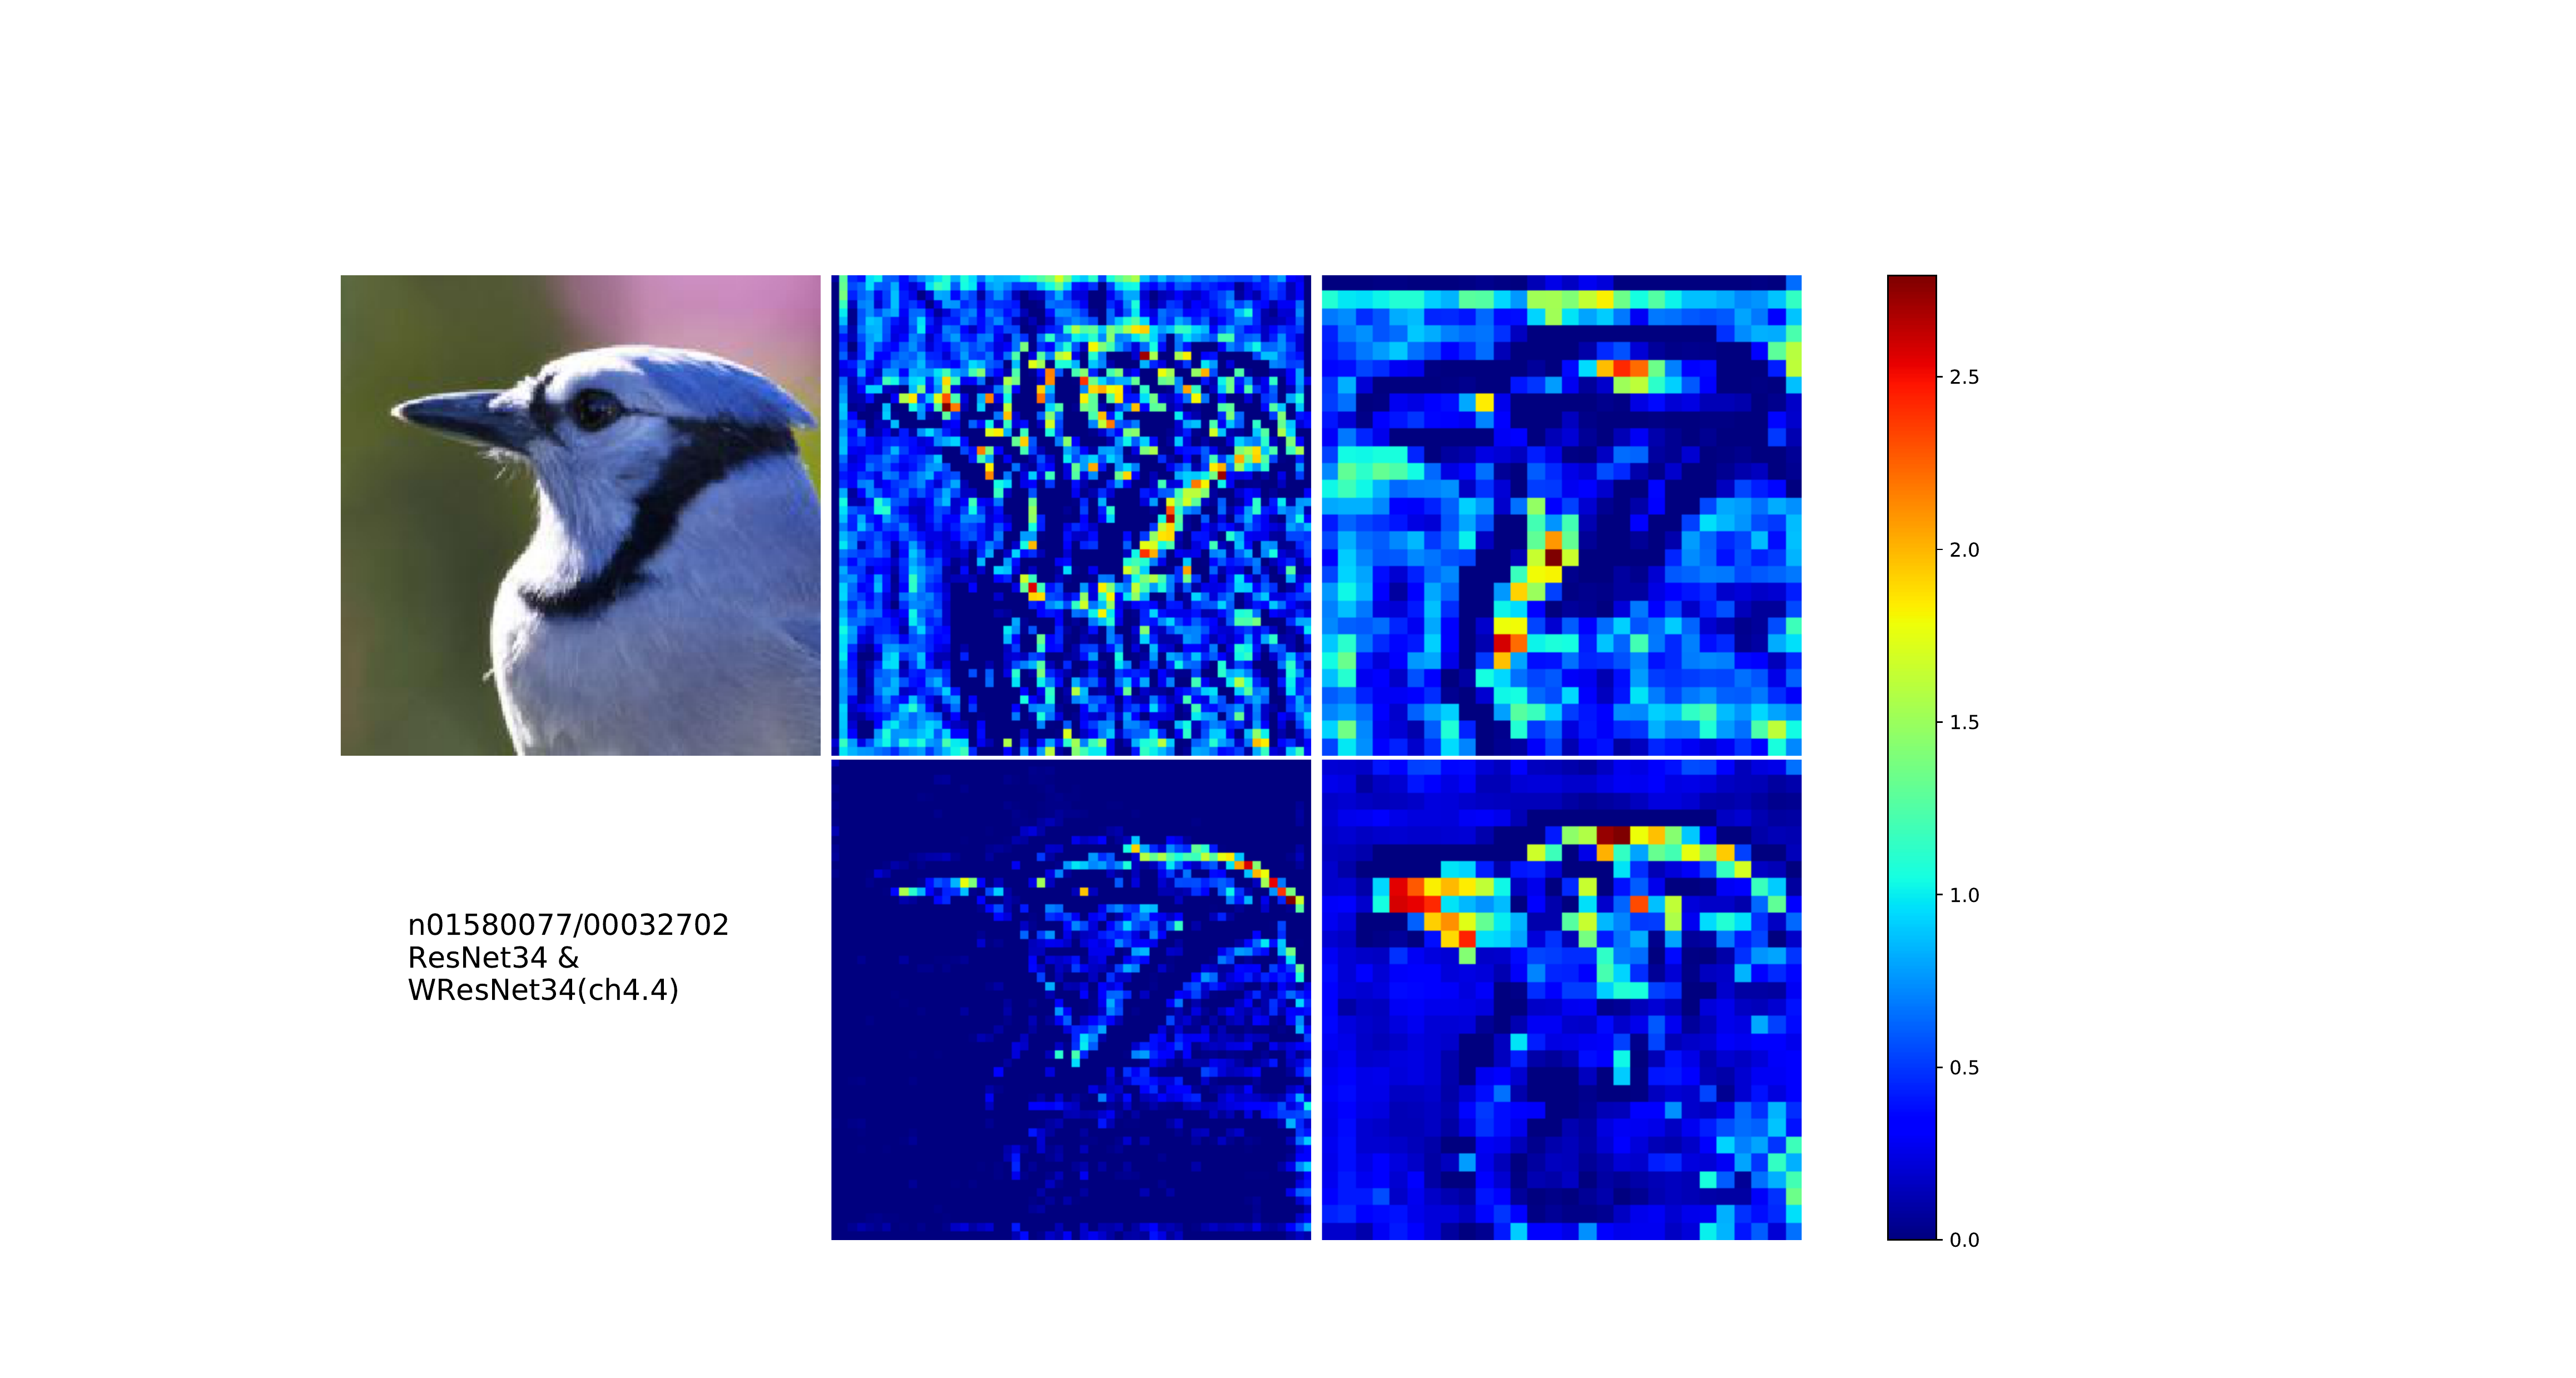}}\hspace{30pt}
	\subfigure[]
	{\includegraphics*[scale=0.25, viewport=175 65 1025 575]{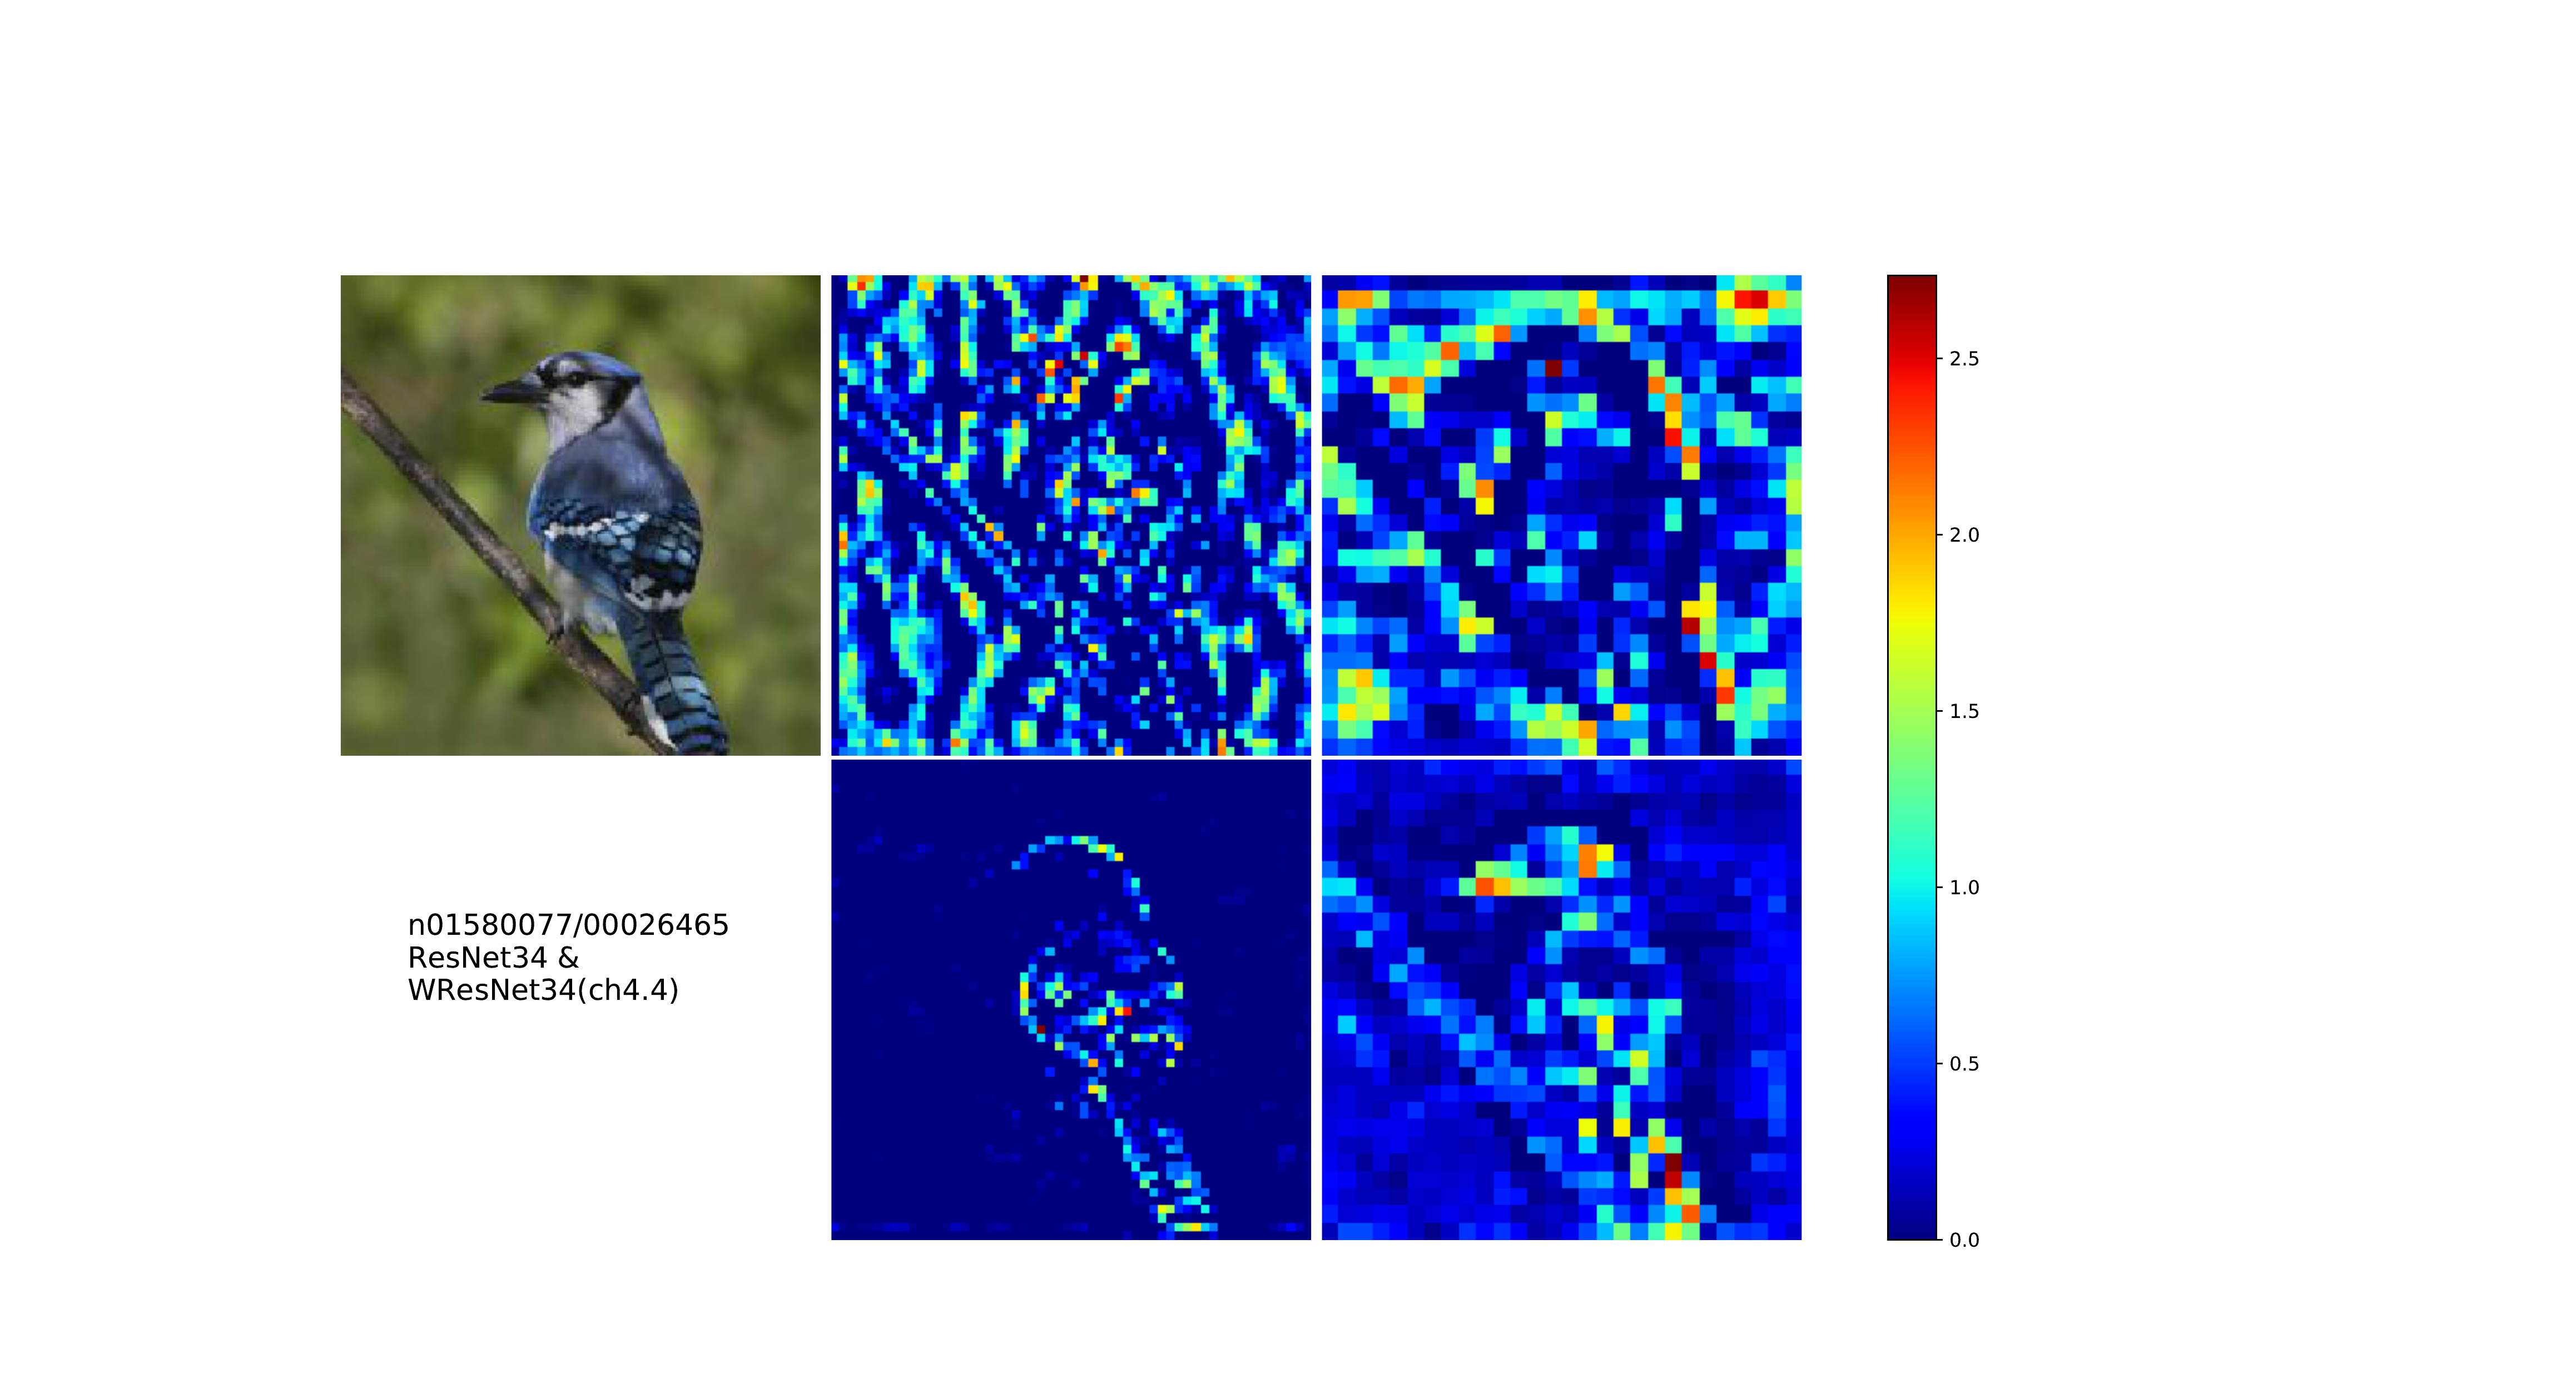}}\\
	\subfigure[]
	{\includegraphics*[scale=0.25, viewport=175 65 1025 575]{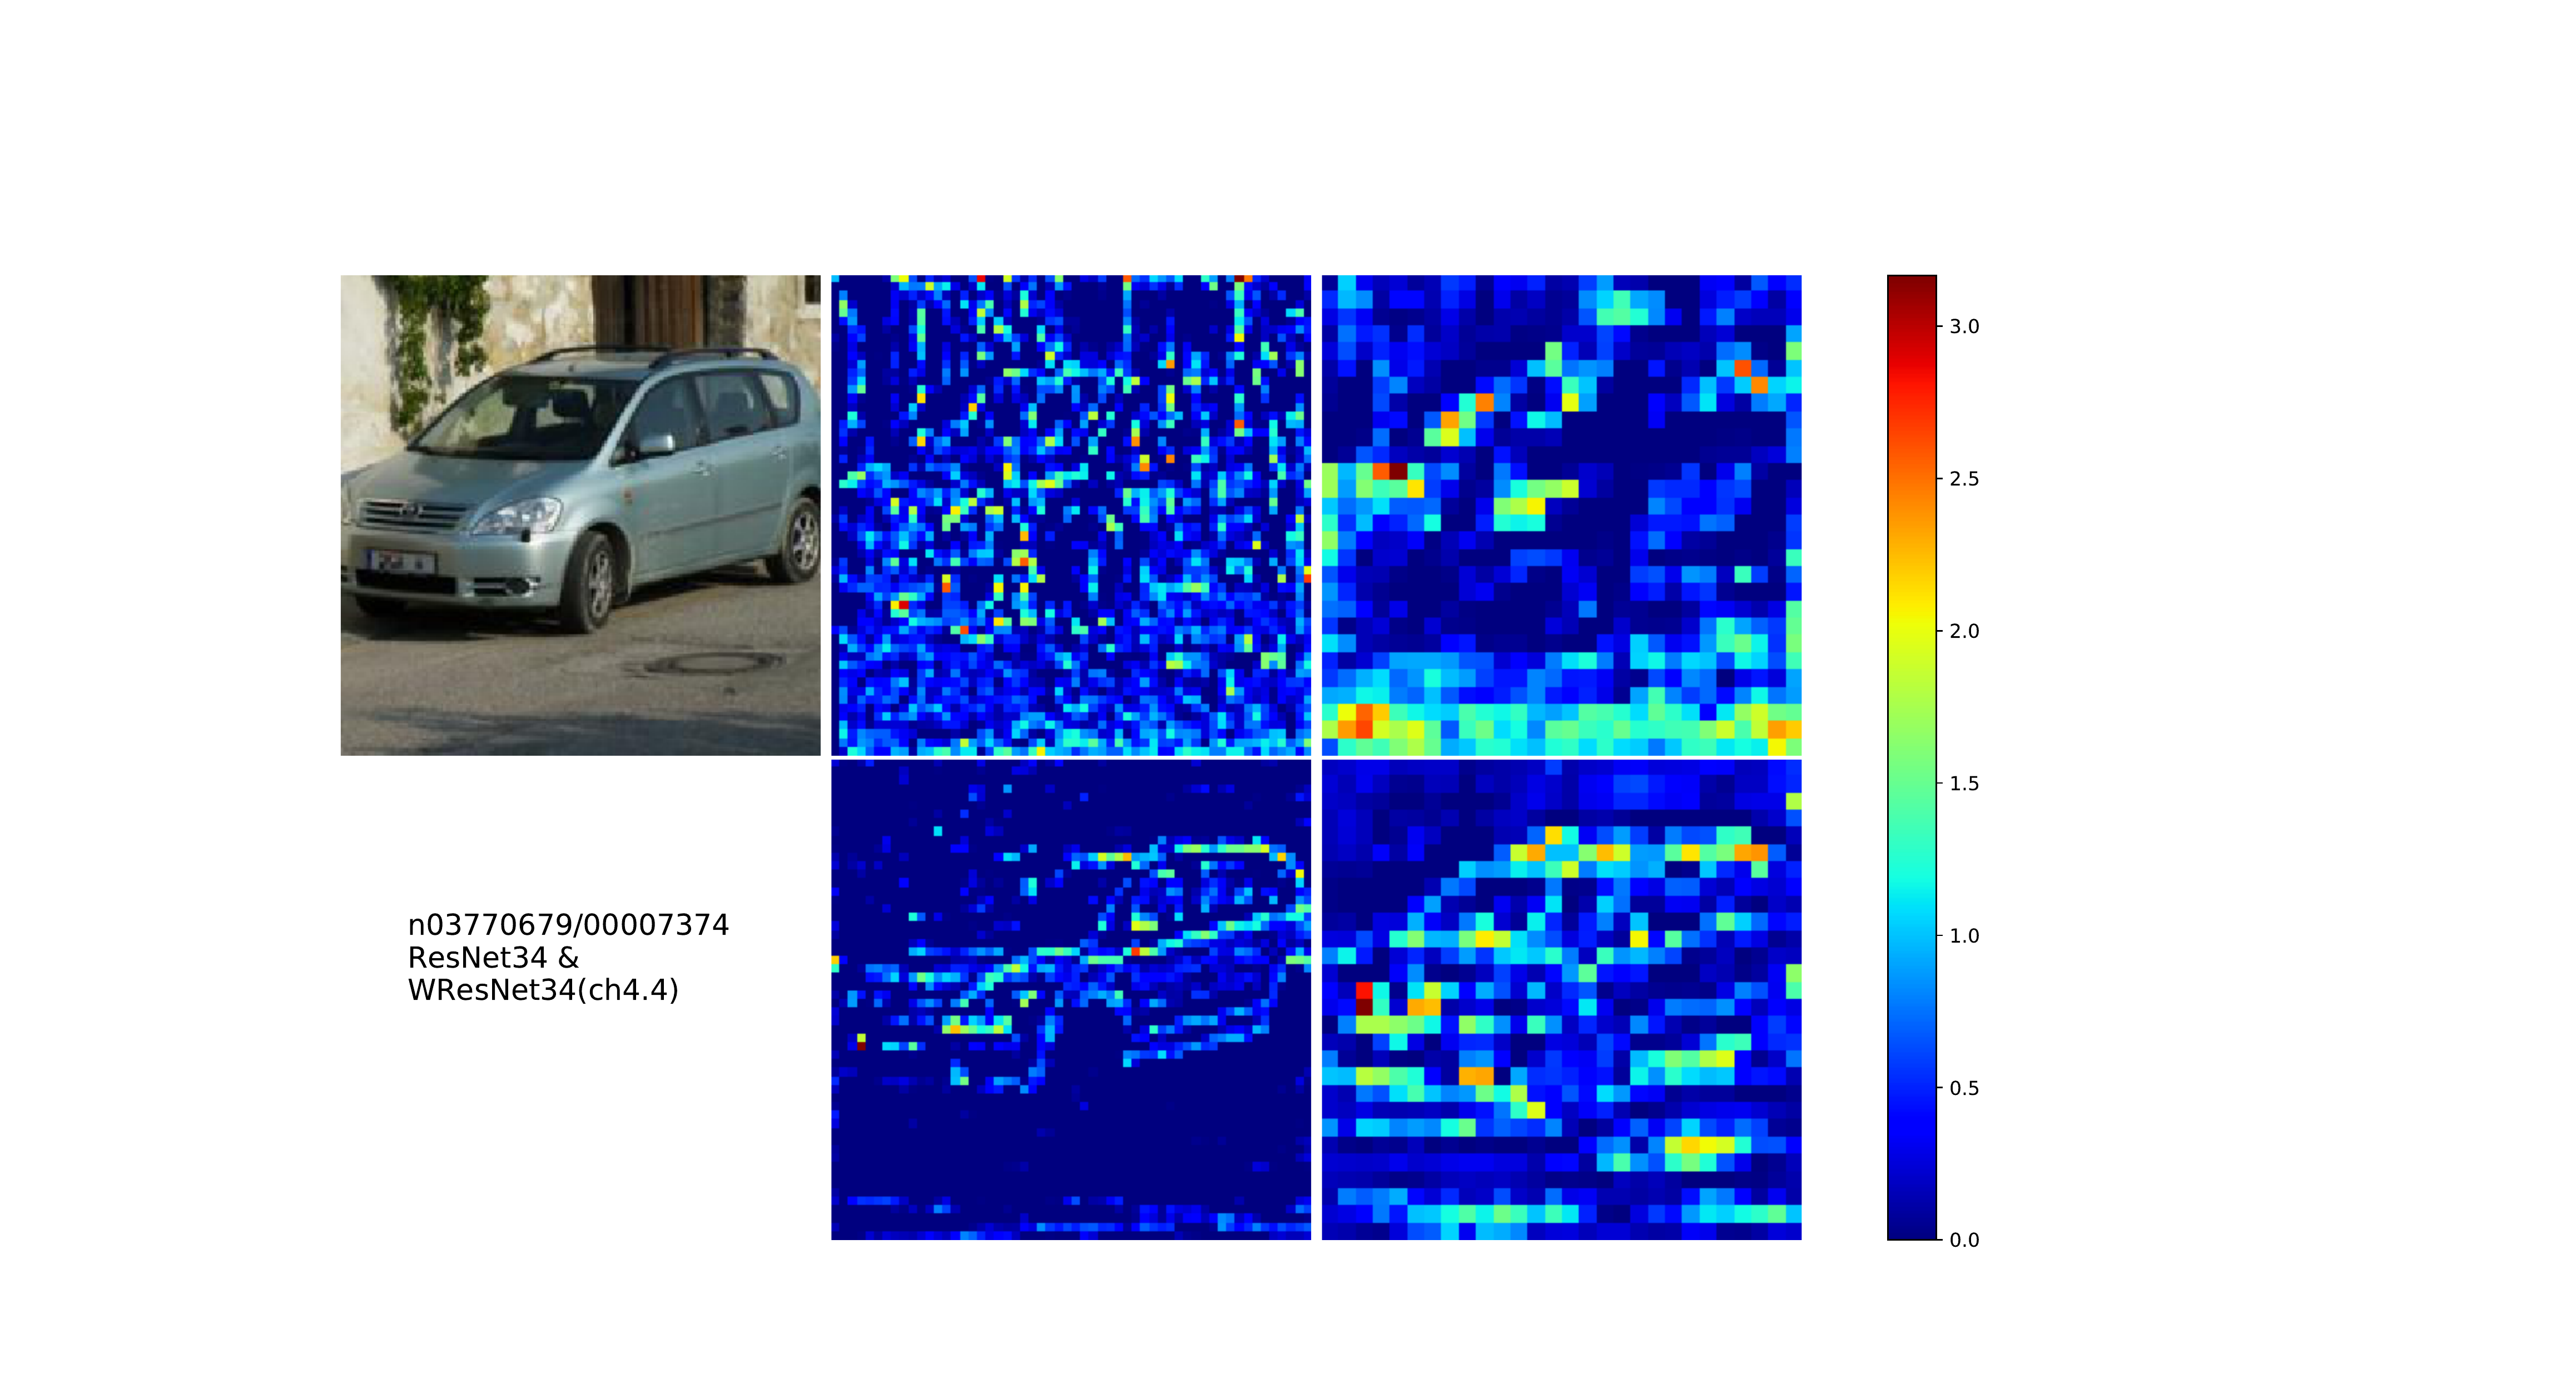}}\hspace{30pt}
	\subfigure[]
	{\includegraphics*[scale=0.25, viewport=175 65 1025 575]{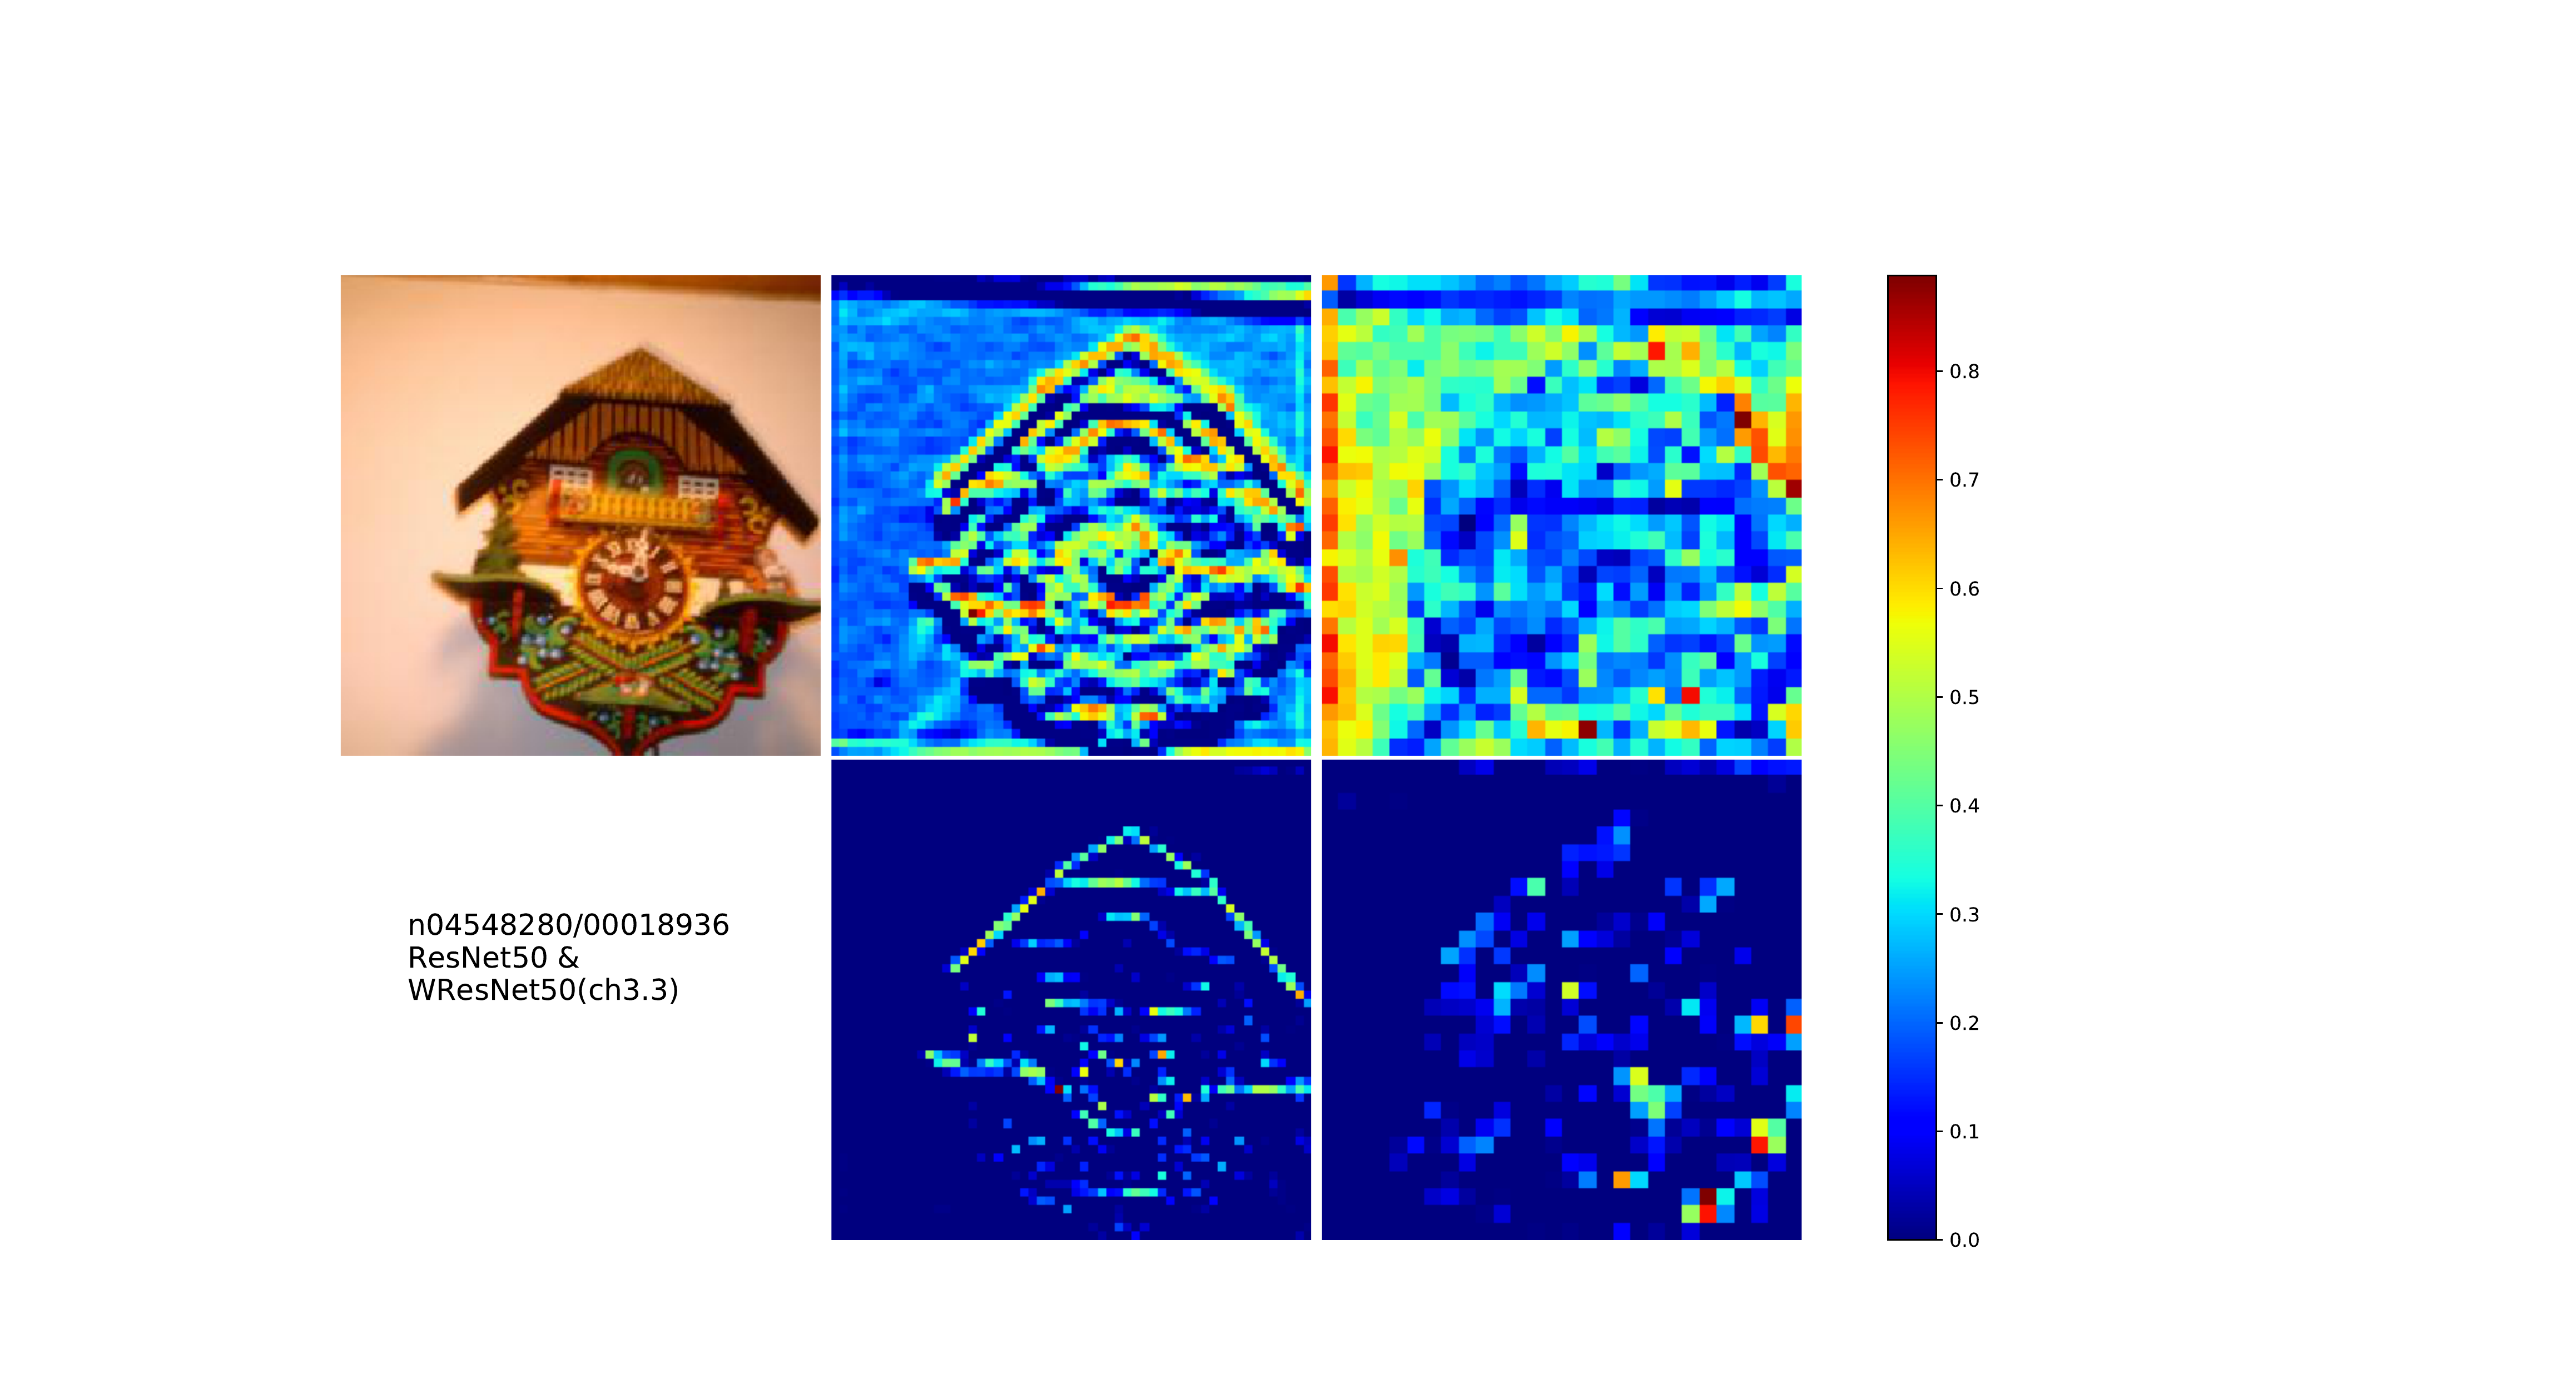}}\\
	\subfigure[]
	{\includegraphics*[scale=0.25, viewport=175 65 1025 575]{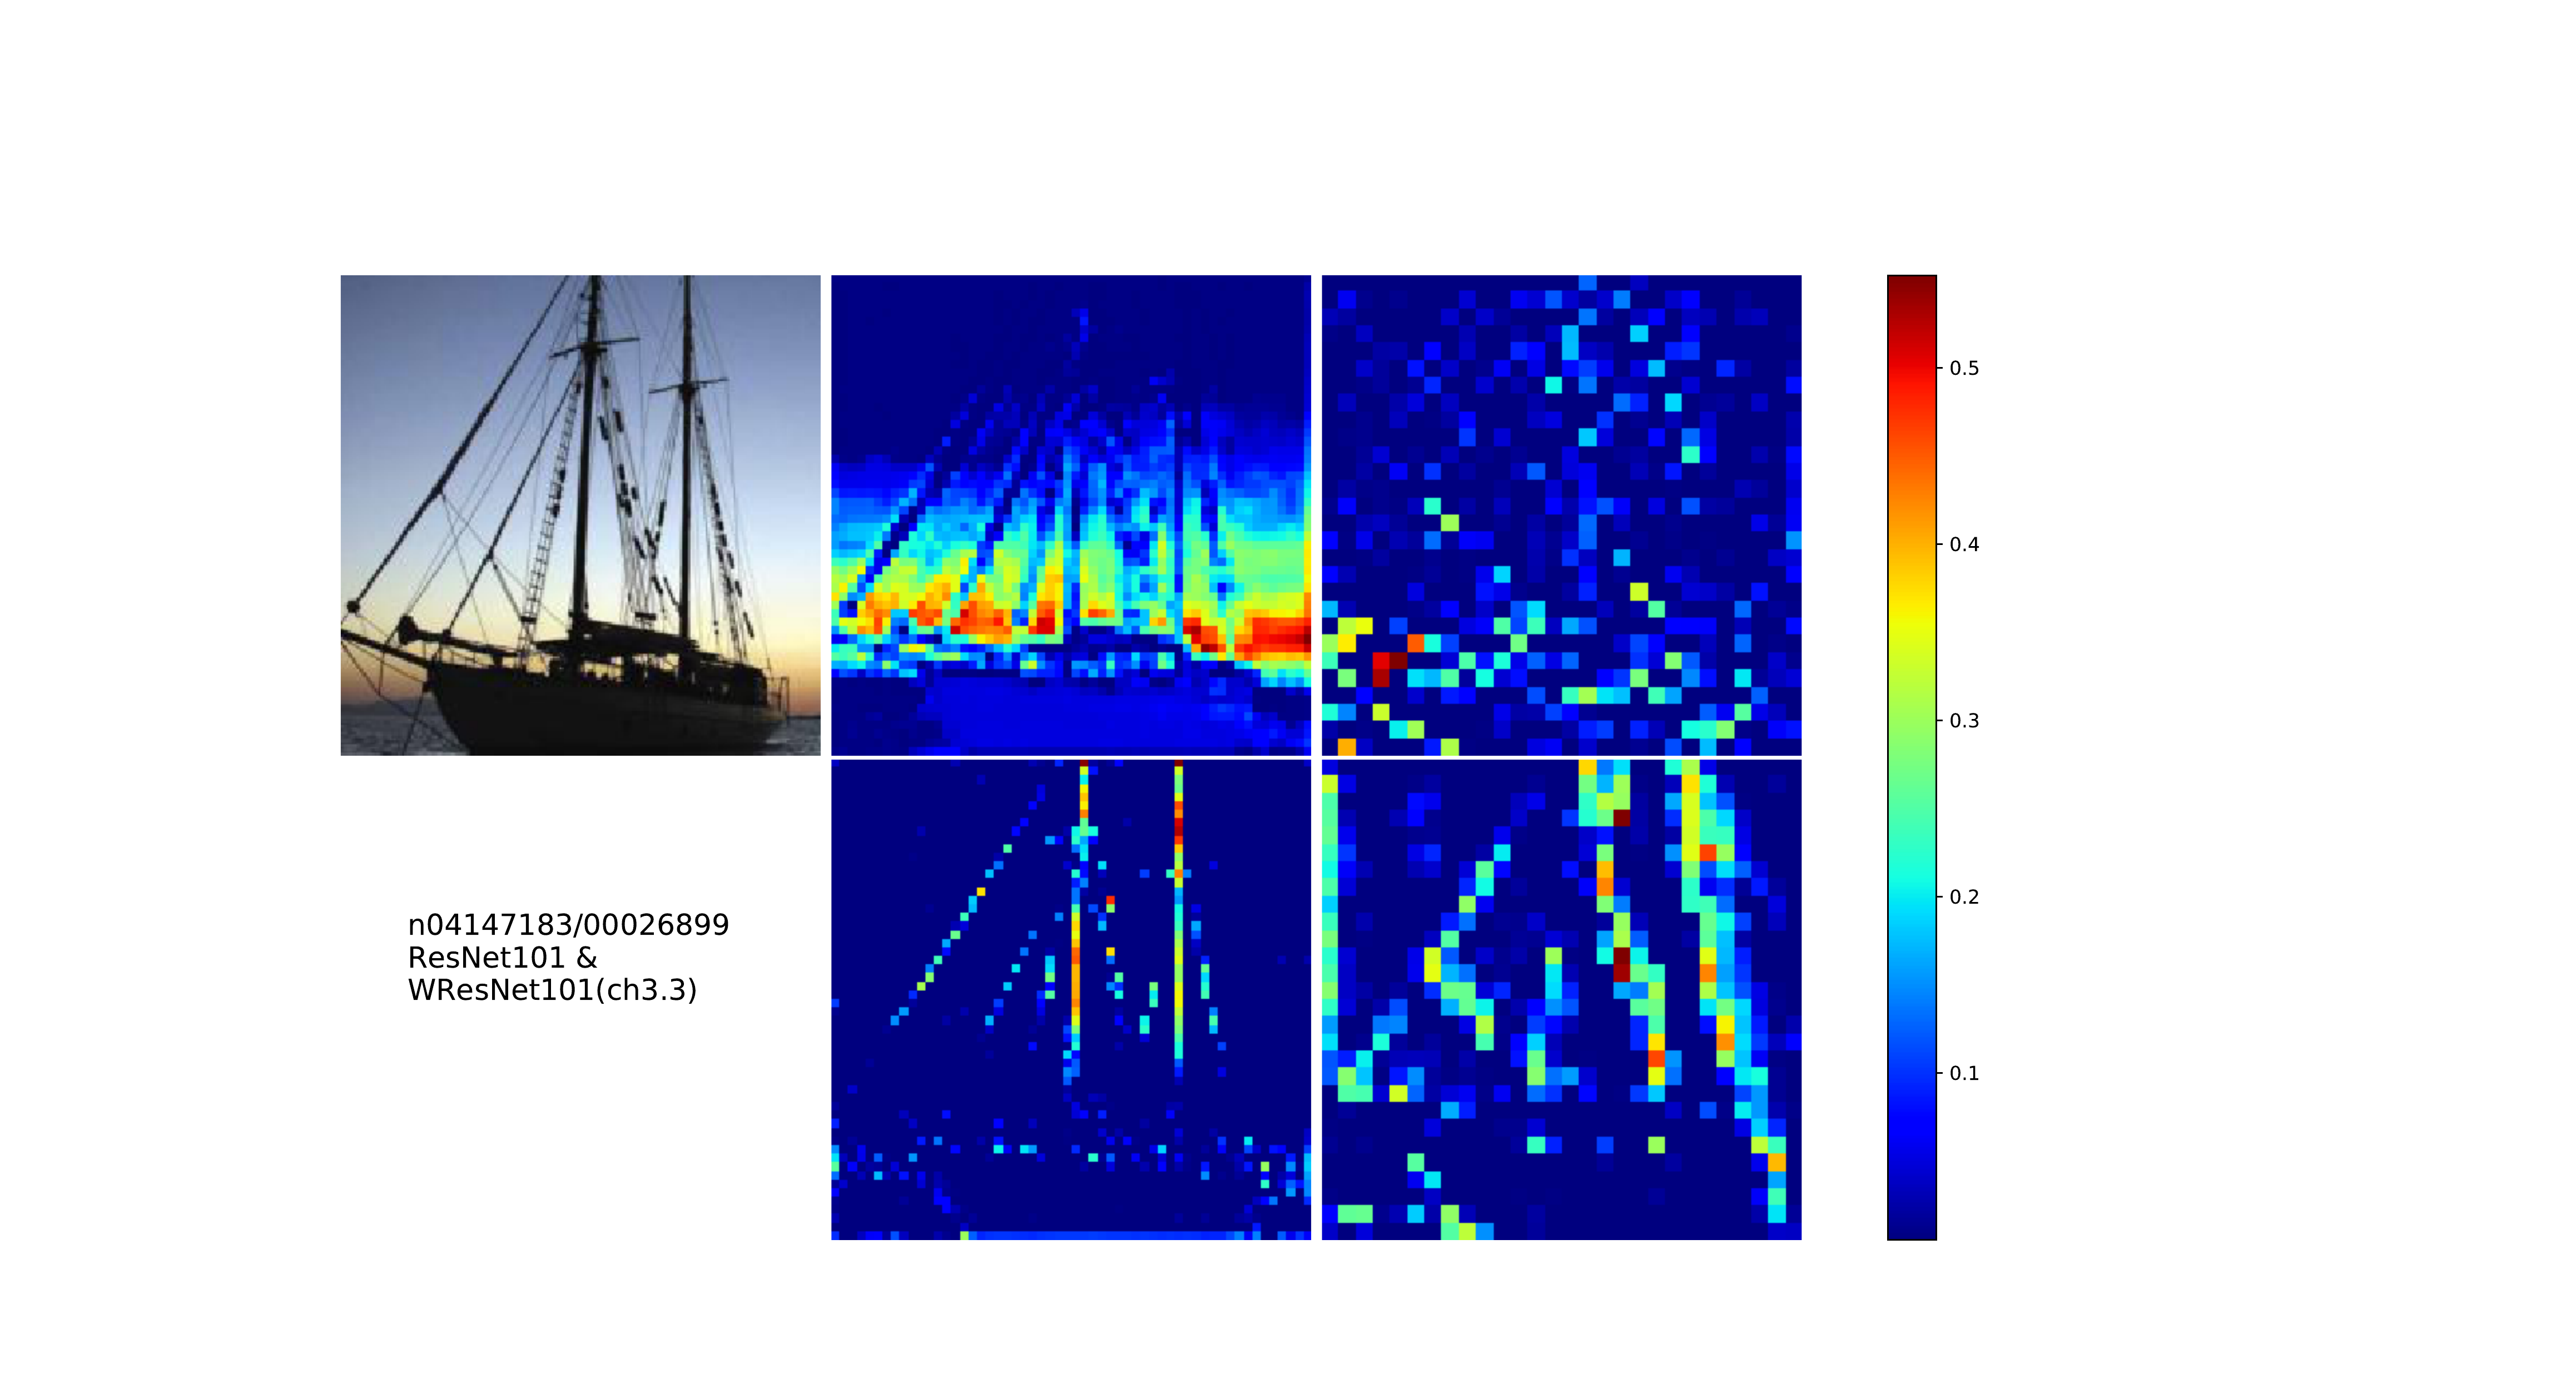}}\hspace{30pt}
	\subfigure[]
	{\includegraphics*[scale=0.25, viewport=175 65 1025 575]{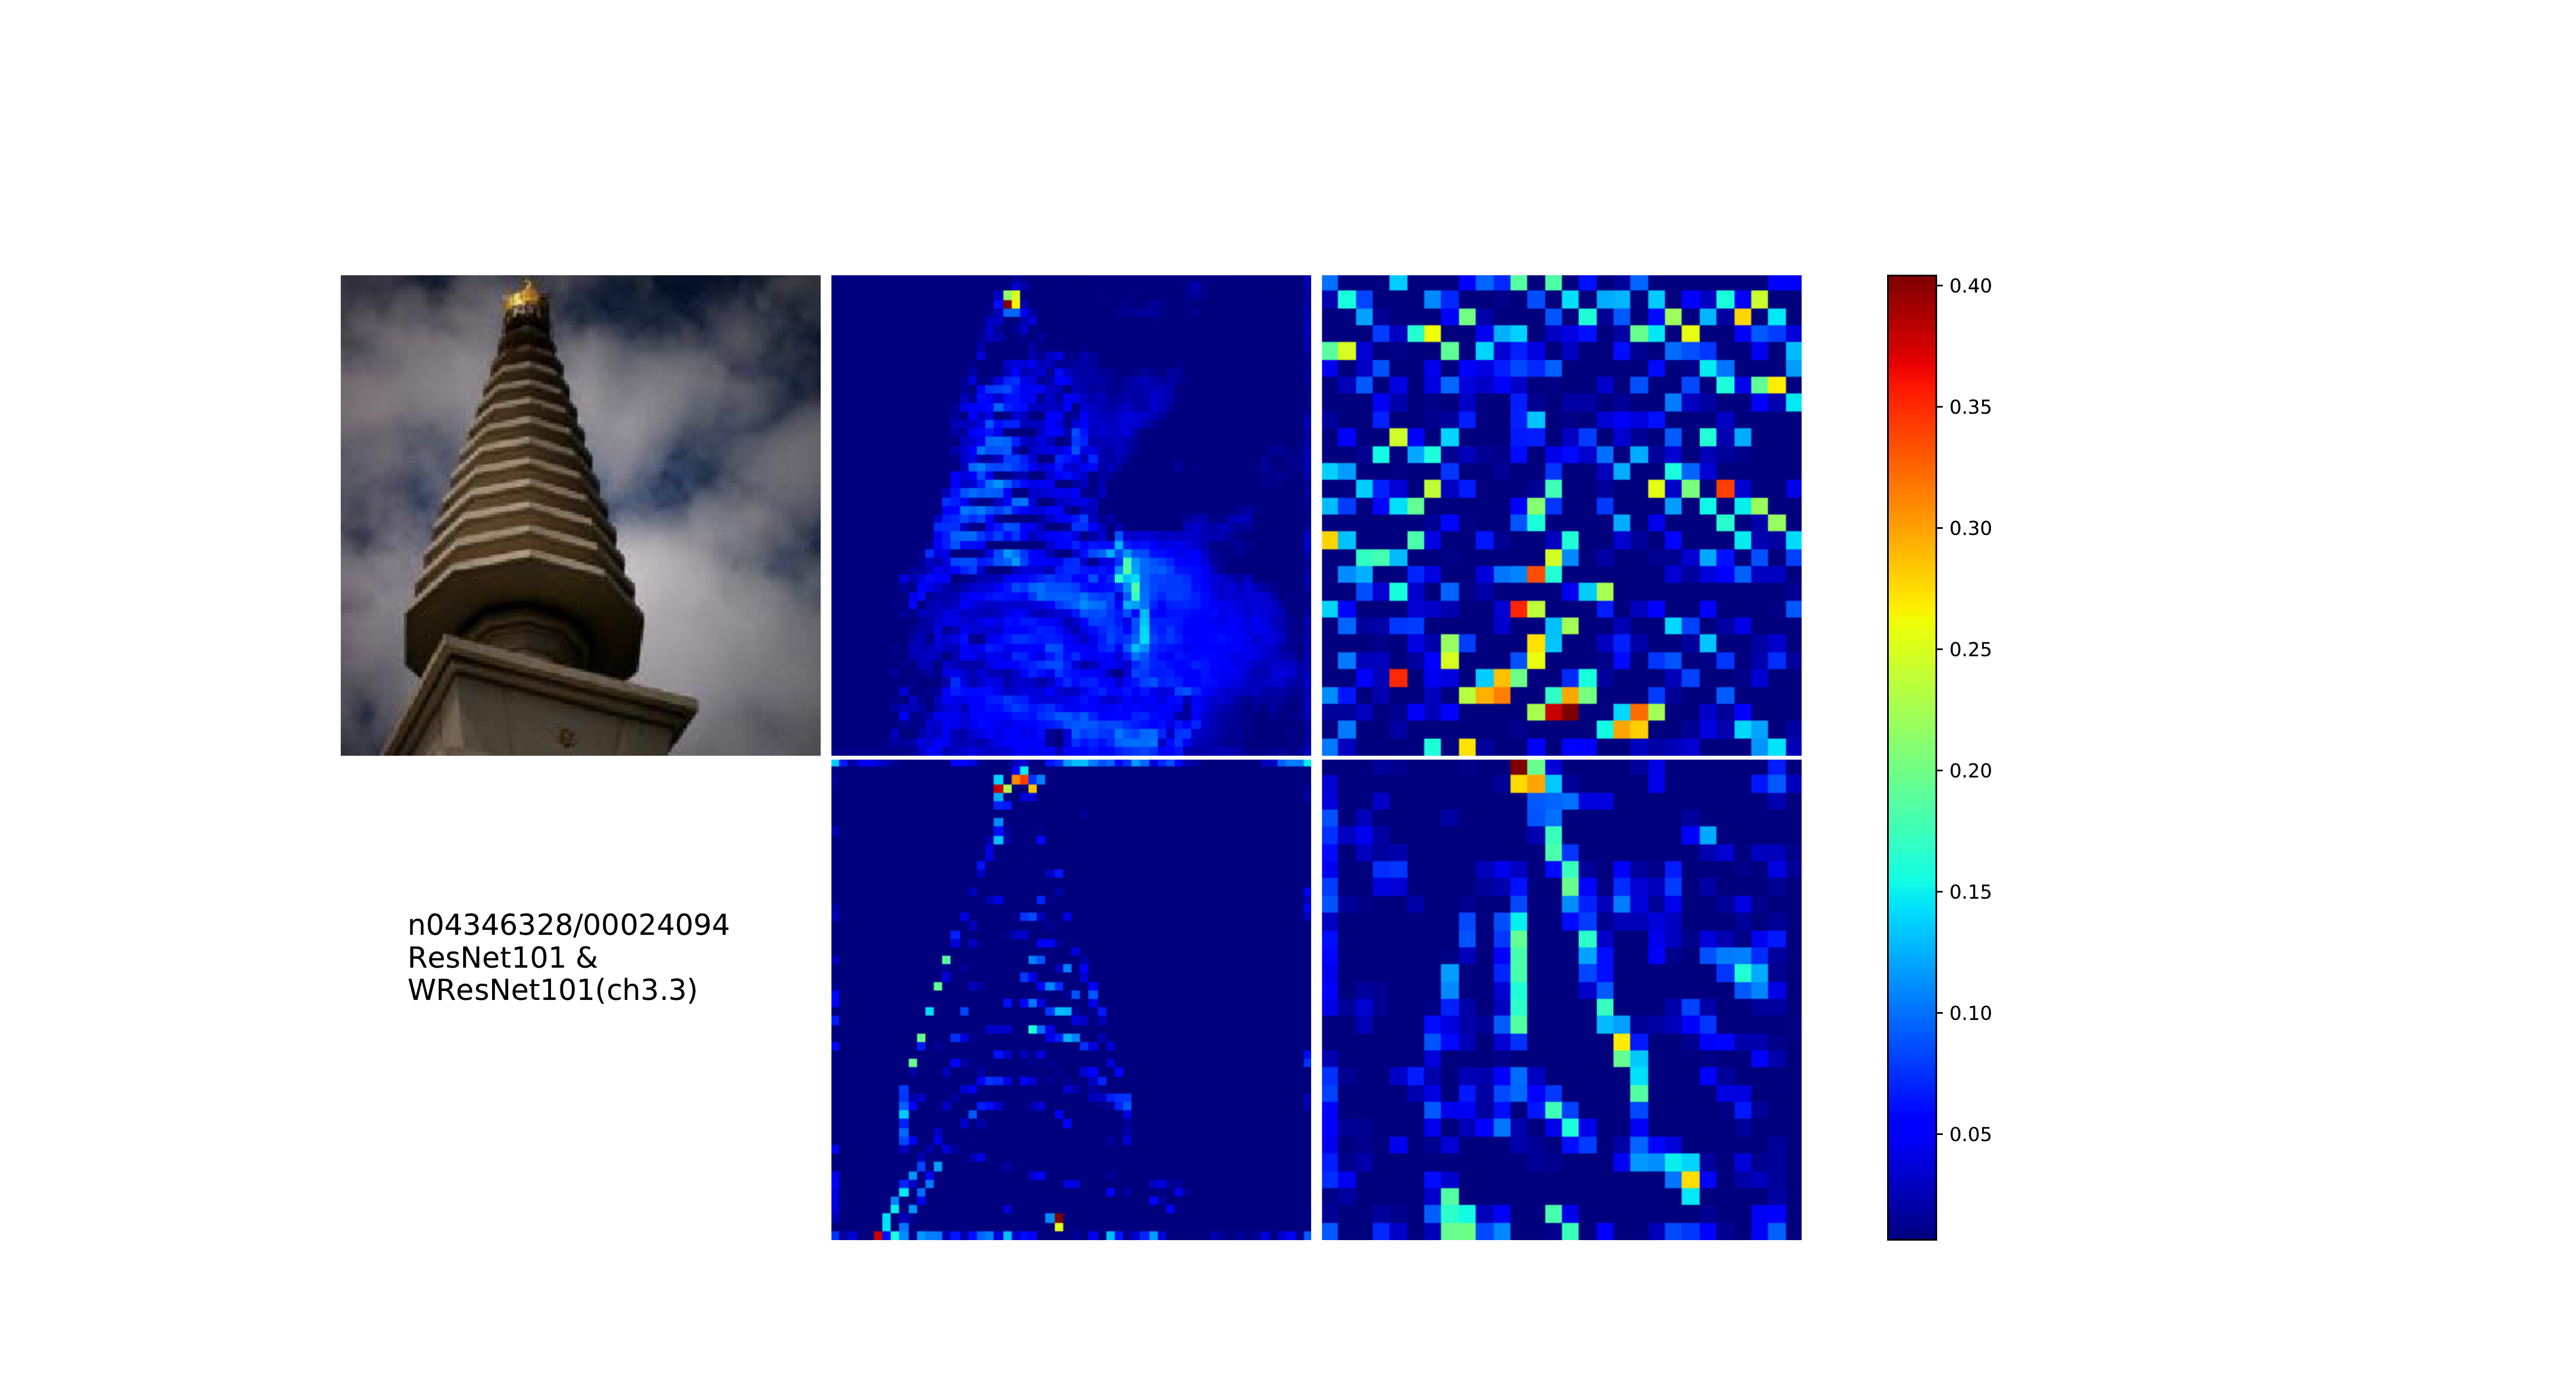}}\\
	\subfigure[]
	{\includegraphics*[scale=0.25, viewport=175 65 1025 575]{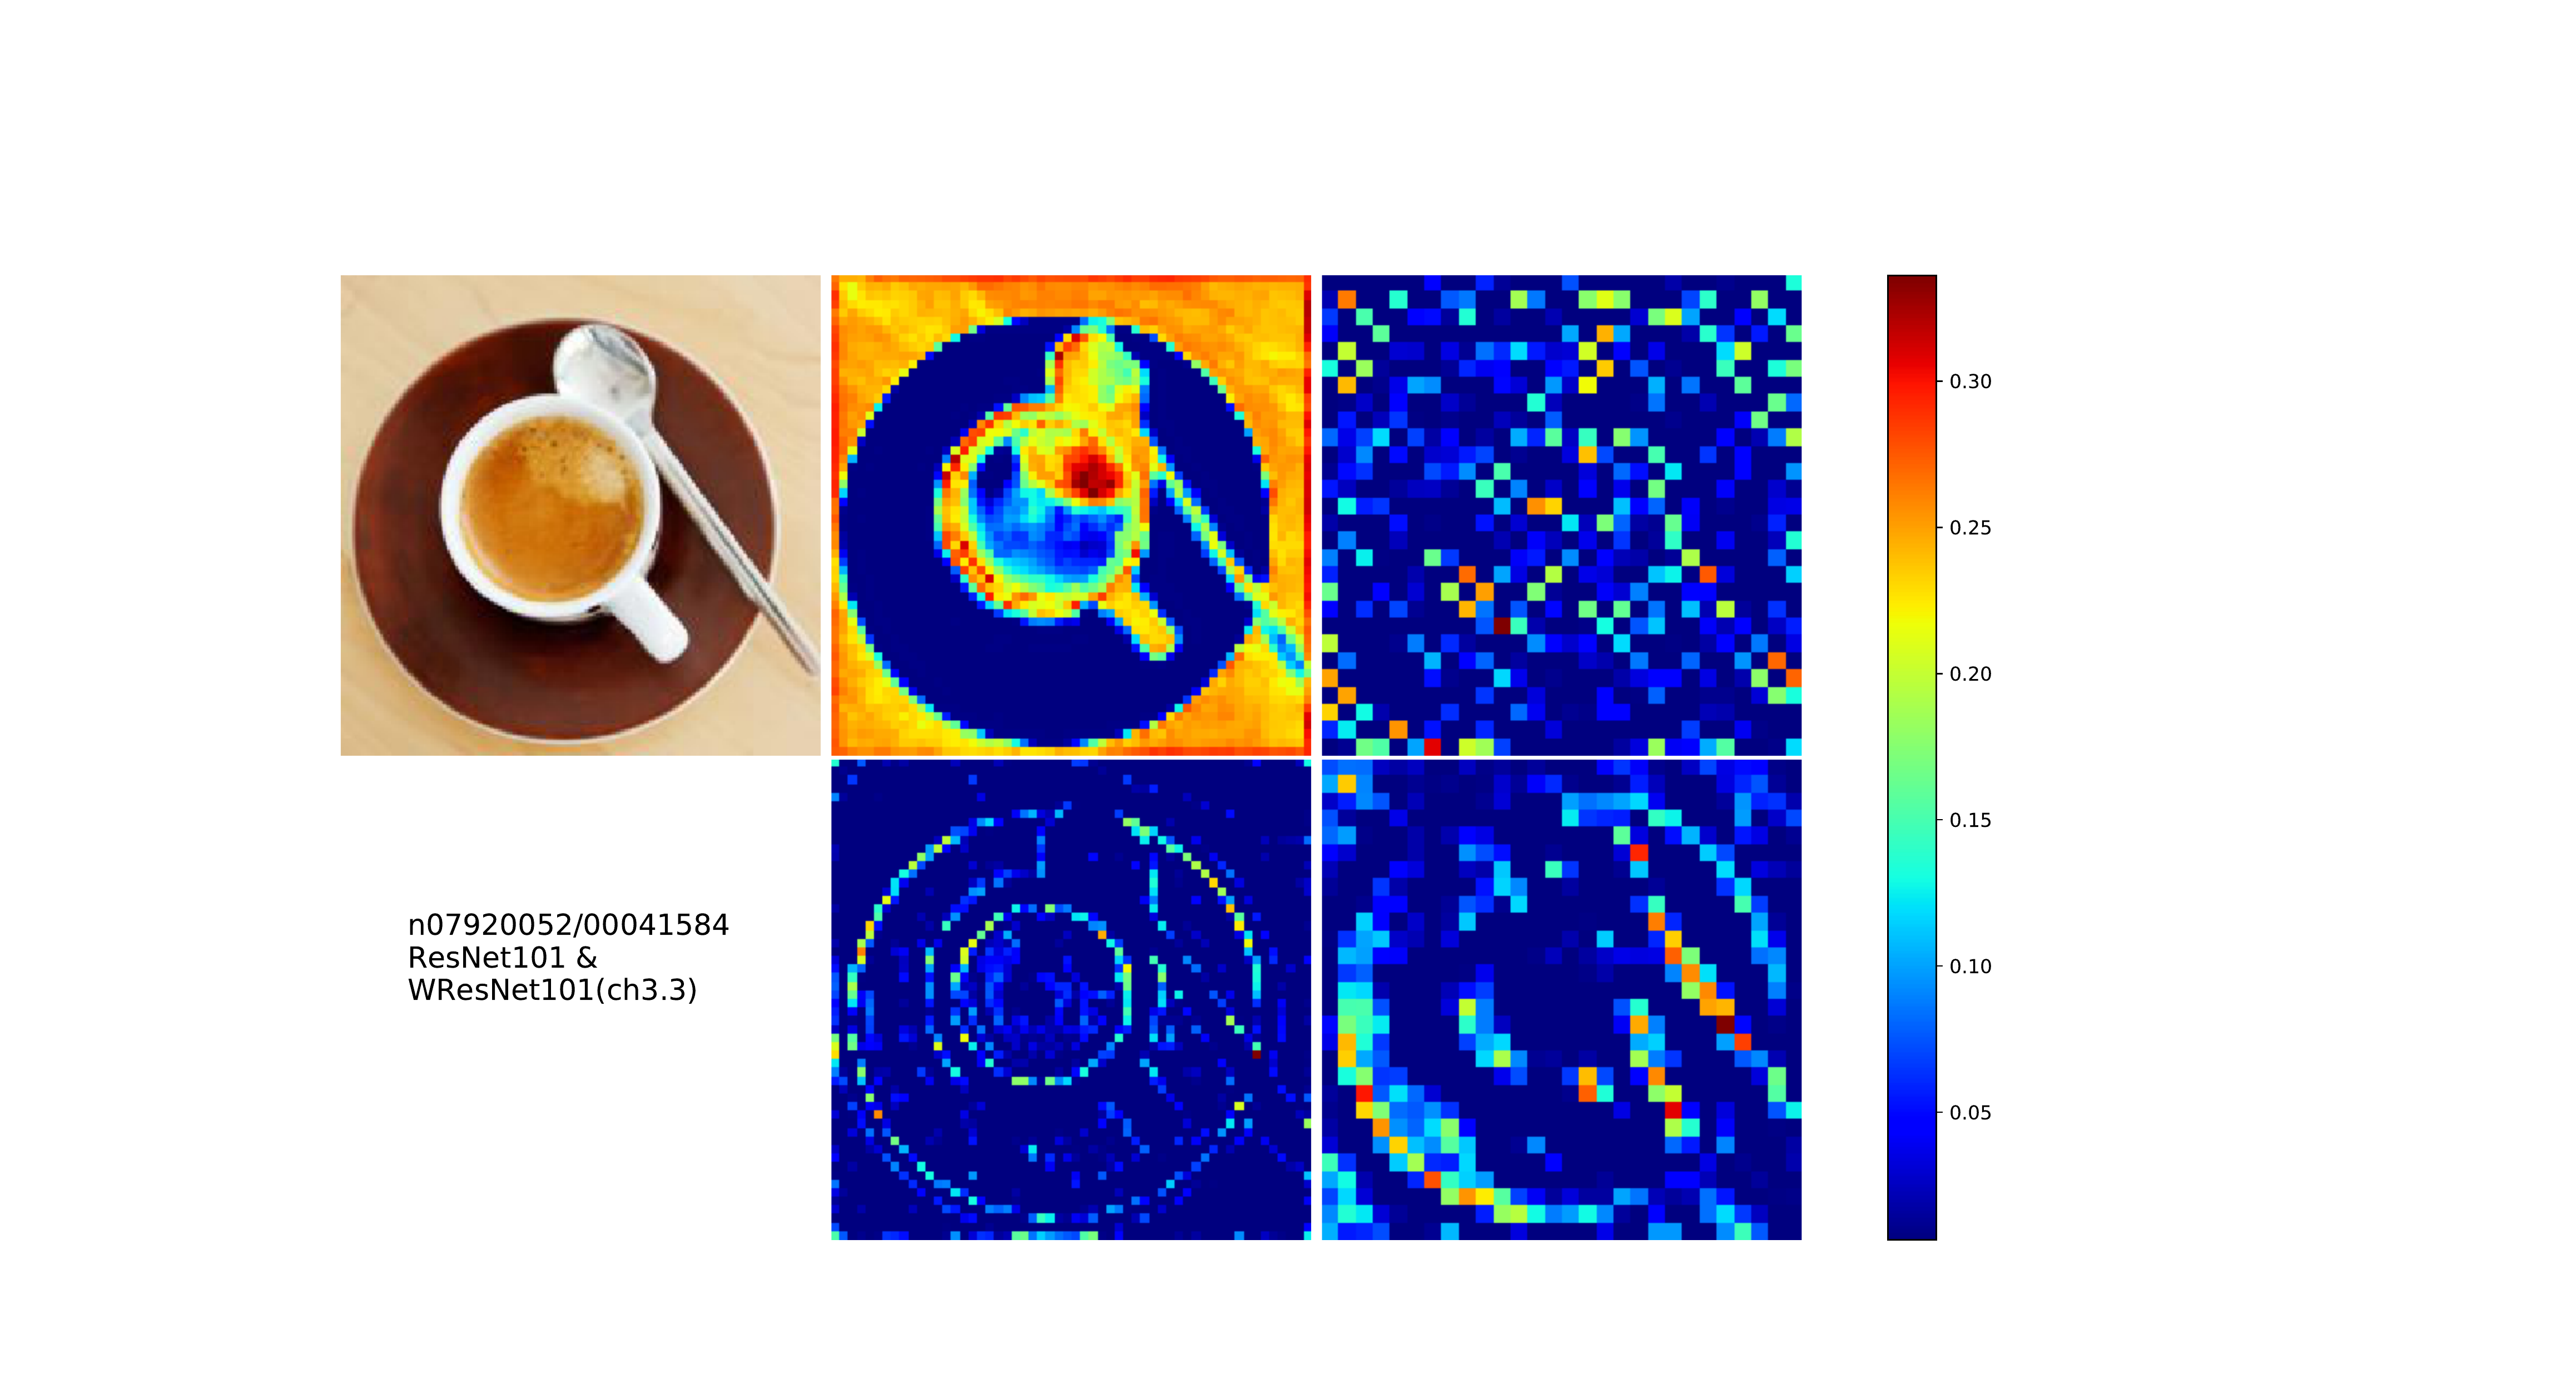}}\hspace{30pt}
	\subfigure[]
	{\includegraphics*[scale=0.25, viewport=175 65 1025 575]{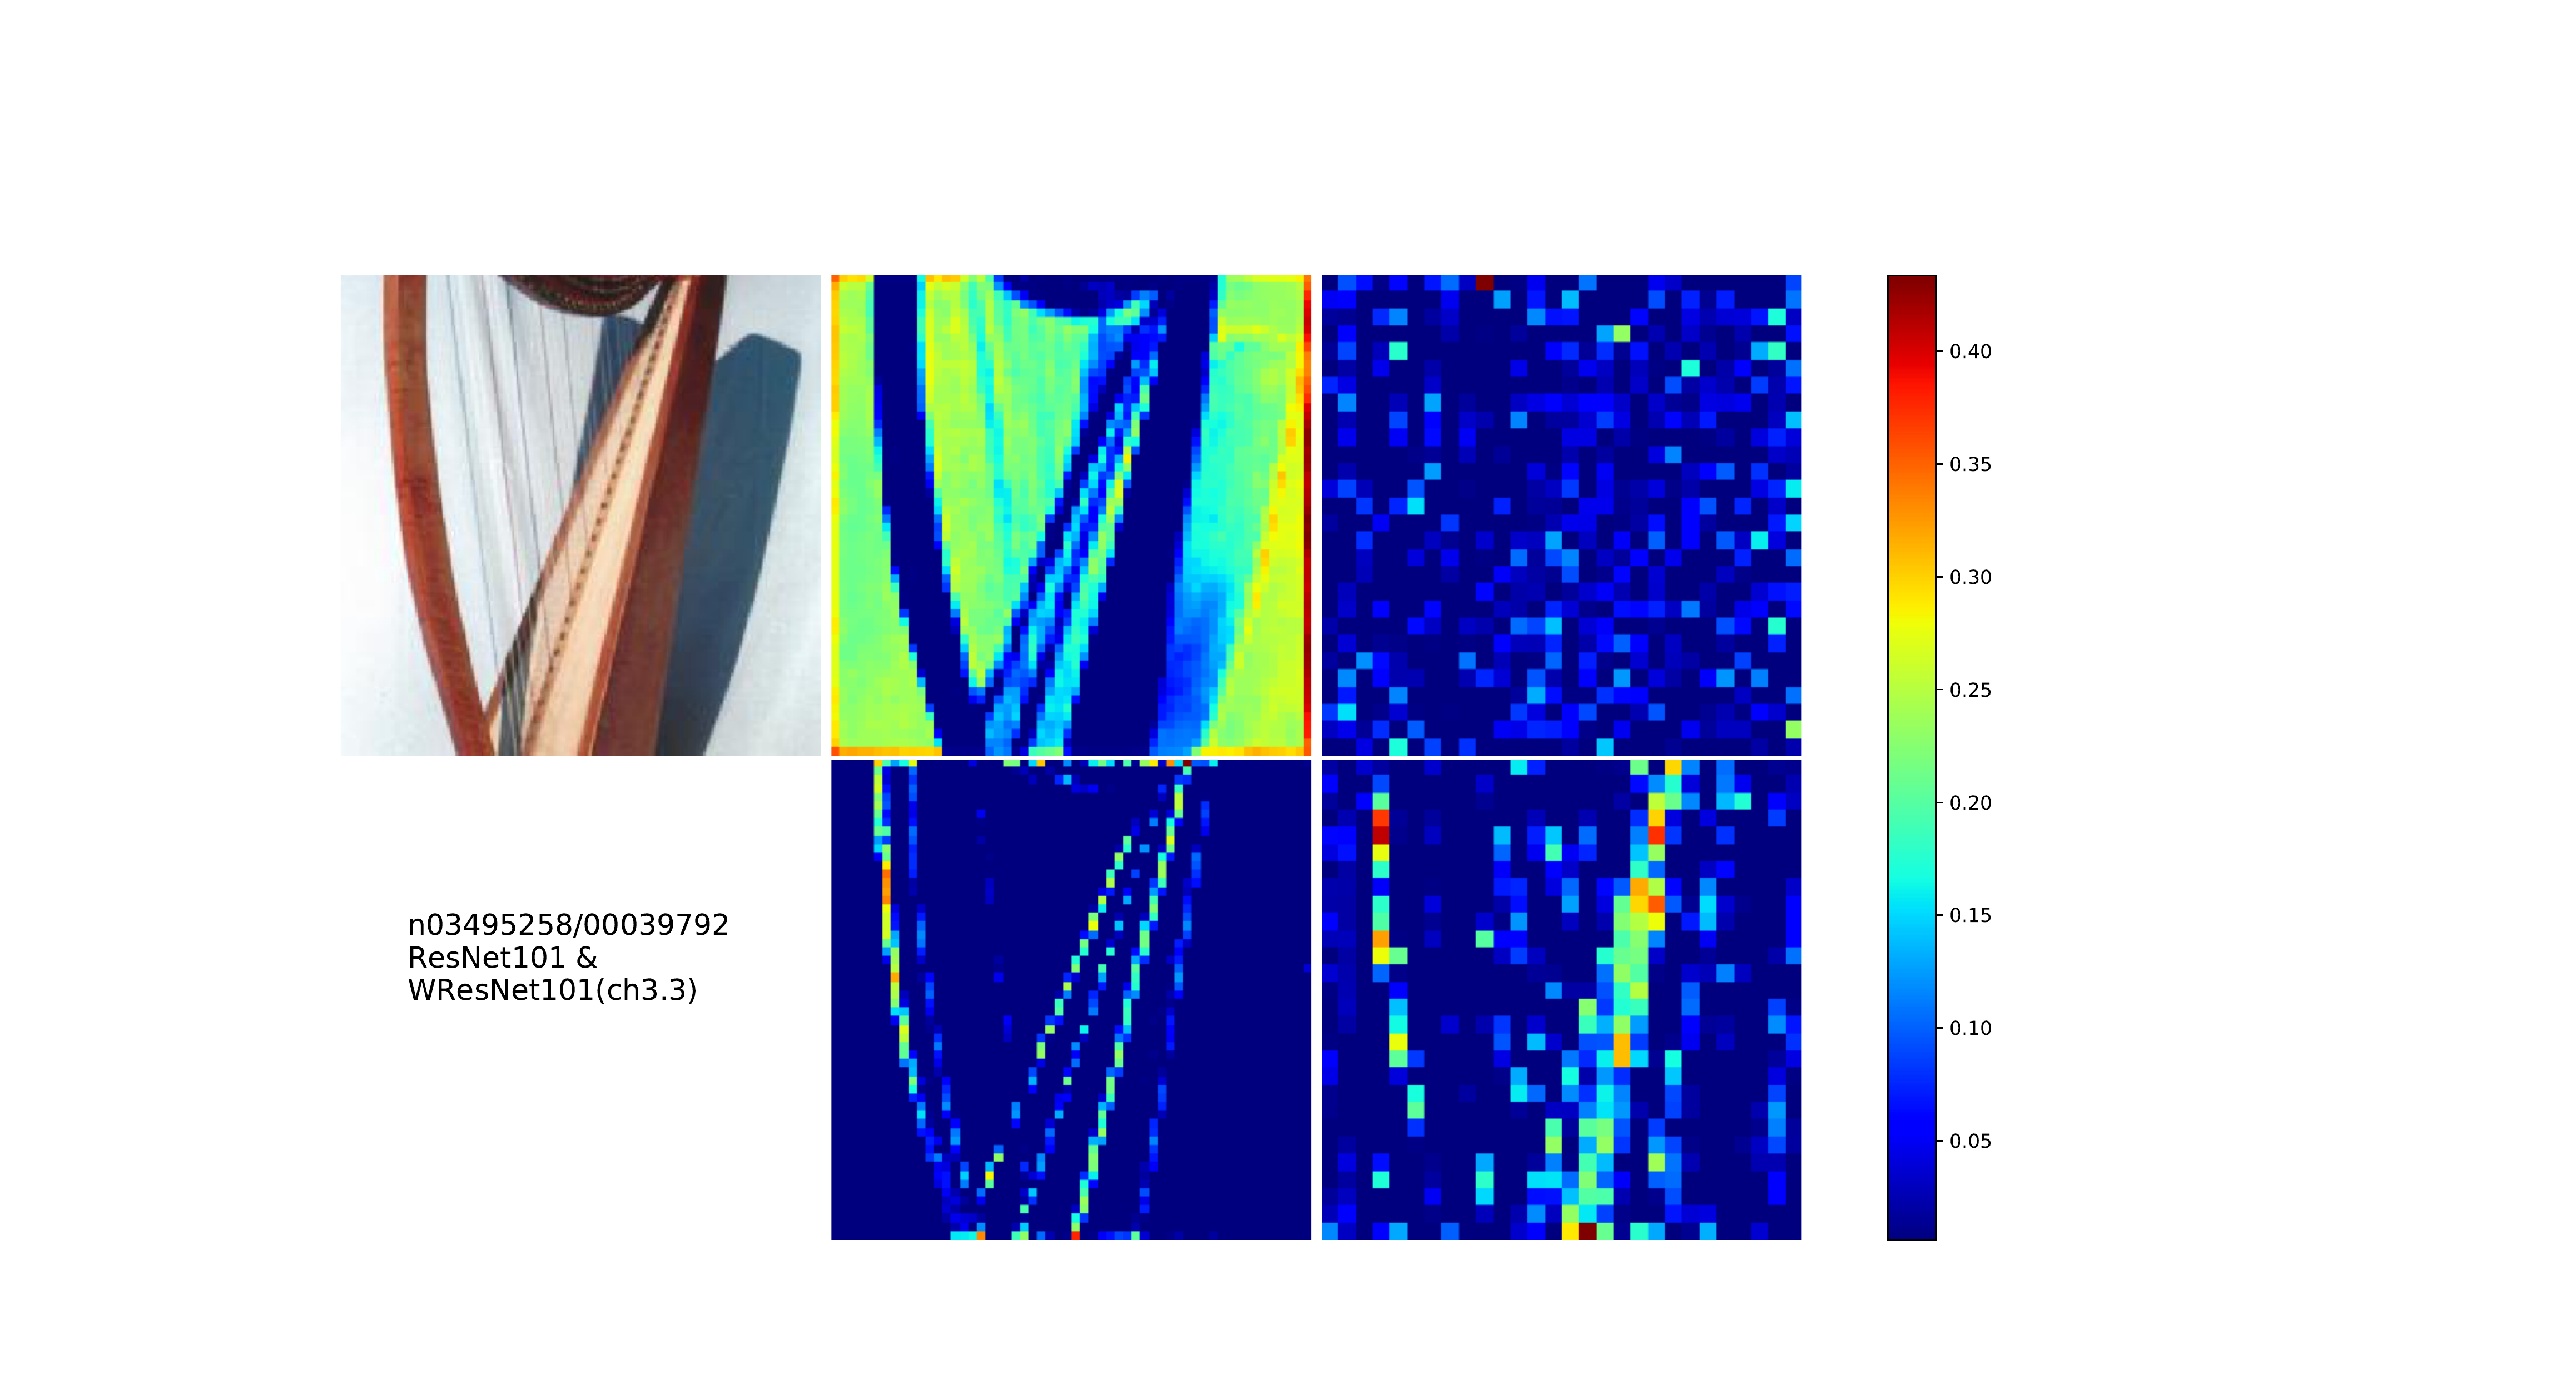}}
	\caption{The feature maps of CNNs (top) and WaveCNets (bottom).}
	\label{fig_feature_maps_more_1}
\end{figure*}

These examples cover the various deep network architectures (VGG16bn, ResNet18, ResNet34, ResNet50, and ResNet101)
and various objects (building, person, cup, dog, bird, car, and boat, etc.).
While the original CNNs adopt various down-sampling operations, such as max-pooling, average-pooling, and strided-convolution,
WaveCNets replace them using DWT.
The feature maps with size of $56\times56$ generated by WaveCNets are cleaner than that generated by original CNNs,
and the object structures in the WaveCNet feature maps with size of $28 \times 28$ are more complete than that in CNN feature maps.
These examples illustrate the aliasing effects introduced by the down-sampling operations in the deep networks,
and the application of DWT in suppressing the effects.

\subsection*{C. The detailed results on ImageNet-C}
\begin{table*}[!t]
	\scriptsize
	%\small
	\caption{Corruption Error (CE) of WVGG16bn on ImageNet-C (lower is better).}\vspace{0pt}
	\label{Tab_mCE_VGG16bn}
	\begin{center}
	\setlength{\tabcolsep}{0.75mm}{
	\begin{tabular}{r|cccc|ccccc|ccccc|ccccc}\hline
		& \multicolumn{4}{c|}{Noise}& \multicolumn{5}{c|}{Blur}& \multicolumn{5}{c|}{Weather}& \multicolumn{5}{c}{Digital}\\\cline{2-20}
		& Gauss&Shot&Impulse&mCE&Defocus&Glass&Motion&Zoom&mCE&Snow&Frost&Fog&Bright&mCE&Contrast&Elastic&Pixel&Jpeg&mCE\\\hline
baseline&  86.28&   87.48&   89.11& 87.62&  83.95&   \textbf{94.80}&   86.36&   87.56& 88.17&  83.25&   \textbf{79.98}&   72.06&   \textbf{63.53}& 74.70&  75.02&   \textbf{95.22}&   94.87&   \textbf{88.88}& \textbf{88.50}\\\cdashline{1-20}[2.25pt/3pt]
haar&      85.80&   86.67&   89.82& 87.43&  84.24&   95.23&   85.46&   86.84& 87.94&  84.62&   80.68&   72.02&   64.38& 75.43&  75.74&   96.40&   96.49&   89.34& 89.49\\
ch2.2&     87.29&   87.80&   88.29& 87.79&  \textbf{83.63}&   95.63&   84.91&   \textbf{86.08}& \textbf{87.56}&  \textbf{82.70}&   80.65&   \textbf{71.55}&   63.64& \textbf{74.63}&  \textbf{74.66}&   96.17&   92.95&   90.34& 88.53\\
ch3.3&     86.40&   87.39&   91.04& 88.28&  84.03&   95.90&   \textbf{85.30}&   86.34& 87.89&  83.81&   81.01&   72.43&   64.14& 75.35&  75.18&   96.05&   93.34&   89.73& 88.58\\
ch4.4&     \textbf{85.01}&   \textbf{85.45}&   \textbf{86.44}& \textbf{85.63}&  84.34&   95.58&   85.77&   86.59& 88.07&  84.21&   82.11&   73.02&   64.73& 76.02&  76.62&   96.72&   \textbf{91.19}&   90.13& 88.67\\
ch5.5&     88.38&   89.14&   92.01& 89.84&  84.56&   96.80&   86.02&   86.77& 88.54&  86.58&   82.51&   74.24&   65.52& 77.21&  76.57&   97.50&   93.46&   90.23& 89.44\\\cdashline{1-20}[2.25pt/3pt]
db2&       86.54&   88.27&   87.51& 87.44&  84.46&   95.69&   85.43&   86.41& 88.00&  84.37&   81.46&   72.94&   64.76& 75.88&  76.57&   96.35&   93.14&   90.86& 89.23\\\hline
	\end{tabular}}
	\end{center}
\end{table*}
\begin{table*}[!t]
	\scriptsize
	%\small
	\caption{Corruption Error (CE) of WResNet18 on ImageNet-C (lower is better).}\vspace{0pt}
	\label{Tab_mCE_ResNet18}
	\begin{center}
	\setlength{\tabcolsep}{0.75mm}{
	\begin{tabular}{r|cccc|ccccc|ccccc|ccccc}\hline
		& \multicolumn{4}{c|}{Noise}& \multicolumn{5}{c|}{Blur}& \multicolumn{5}{c|}{Weather}& \multicolumn{5}{c}{Digital}\\\cline{2-20}
		& Gauss&Shot&Impulse&mCE&Defocus&Glass&Motion&Zoom&mCE&Snow&Frost&Fog&Bright&mCE&Contrast&Elastic&Pixel&Jpeg&mCE\\\hline
baseline& 87.15&   88.47&   91.30&  88.97&   83.82&   91.43&   86.82&   88.70&   87.69&    86.10&   84.40&   78.48&   68.90&    79.47&   78.29&   90.23&   80.40&    \textbf{85.46}&    83.60\\\cdashline{1-20}[2.25pt/3pt]
haar&     80.64&   80.94&   81.16&  80.91&   80.18&   90.55&   84.04&   86.49&   85.32&    85.04&   81.93&   73.32&   65.78&    76.52&   75.72&   \textbf{87.78}&   \textbf{74.87}&    87.77  &  81.54  \\
ch2.2&    \textbf{80.15}&   \textbf{80.49}&   \textbf{80.50}&  \textbf{80.38}&   79.65&   \textbf{89.79}&   83.61&   84.82&   \textbf{84.47}&    84.91&   80.84&   73.99&   66.34&    76.52&   75.07&   88.19&   75.07&    88.61 &   \textbf{81.73} \\
ch3.3&    80.85&   81.44&   80.77&  81.02&   \textbf{79.28}&   91.20&   \textbf{82.71}&   85.52&   84.68&    84.48&   81.20&   \textbf{71.76}&   \textbf{65.44}&    \textbf{75.72}&   \textbf{73.77}&   89.66&   77.46&    86.06 &   81.74 \\
ch4.4&    81.83&   82.65&   82.10&  82.19&   79.55&   91.01&   82.88&   \textbf{84.55}&   84.50&    \textbf{83.91}&   \textbf{80.81}&   73.95&   66.27&    76.23&   75.67&   90.21&   78.35&    86.10 &   82.58 \\
ch5.5&    83.60&   83.87&   83.84&  83.77&   80.73&   91.64&   83.04&   85.45&   85.21&    84.39&   81.42&   73.83&   67.10&    76.68&   76.21&   91.07&   78.95&    89.35 &   83.89 \\\cdashline{1-20}[2.25pt/3pt]
db2&      82.30&   82.65&   82.68&  82.54&   80.16&   91.22&   83.55&   84.73&   84.92&    85.42&   81.74&   74.34&   66.51&    77.00&   75.92&   90.41&   79.54&    91.71   & 84.39   \\
db3&      83.75&   84.14&   83.87&  83.92&   81.36&   90.92&   84.14&   86.24&   85.66&    85.01&   81.73&   75.79&   68.14&    77.67&   78.47&   90.02&   78.41&    89.35   & 84.06   \\
db4&      86.00&   85.83&   86.85&  86.22&   82.12&   92.93&   85.75&   87.38&   87.04&    85.31&   83.02&   77.87&   68.97&    78.79&   79.33&   91.07&   74.95&    85.63   & 82.74   \\
db5&      85.22&   85.86&   85.33&  85.47&   82.96&   92.65&   87.83&   88.63&   88.02&    87.60&   85.21&   78.66&   71.33&    80.70&   80.85&   91.11&   78.21&    92.99   & 85.79   \\
db6&      86.29&   86.73&   86.68&  86.57&   84.72&   94.50&   87.73&   88.68&   88.91&    87.88&   86.62&   80.58&   72.81&    81.97&   82.29&   93.46&   78.32&    95.53    & 87.40    \\\hline
	\end{tabular}}
	\end{center}
\end{table*}
\begin{table*}[!t]
	\scriptsize
	%\small
	\caption{Corruption Error (CE) of WResNet34 on ImageNet-C (lower is better).}\vspace{0pt}
	\label{Tab_mCE_ResNet34}
	\begin{center}
	\setlength{\tabcolsep}{0.75mm}{
	\begin{tabular}{r|cccc|ccccc|ccccc|ccccc}\hline
		& \multicolumn{4}{c|}{Noise}& \multicolumn{5}{c|}{Blur}& \multicolumn{5}{c|}{Weather}& \multicolumn{5}{c}{Digital}\\\cline{2-20}
		& Gauss&Shot&Impulse&mCE&Defocus&Glass&Motion&Zoom&mCE&Snow&Frost&Fog&Bright&mCE&Contrast&Elastic&Pixel&Jpeg&mCE\\\hline
baseline&   81.36&   83.01&   84.94&   83.10&   76.04&   86.95&   79.59&   84.56&   81.79&   79.87&   77.02&   69.34&   61.97&   72.05&   71.80&   86.17&   70.54&   \textbf{74.60}& 75.78\\\cdashline{1-20}[2.25pt/3pt]
haar&       75.80&   77.21&   76.89&   76.64&   76.17&   87.25&   76.86&   81.08&   80.34&   80.51&   75.85&   68.33&   60.29&   71.25&   71.17&   84.10&   71.61&   80.17& 76.76\\
ch2.2&      76.91&   77.56&   78.36&   77.61&   73.49&   87.09&   75.77&   80.34&   79.17&   79.59&   \textbf{75.71}&   67.25&   59.59&   70.53&   69.87&   86.27&   67.28&   77.33& 75.19\\
ch3.3&      73.73&   74.66&   74.50&   74.30&   74.42&   89.02&   76.15&   \textbf{79.83}&   79.86&   79.59&   76.74&   \textbf{65.70}&   \textbf{58.82}&   \textbf{70.21}&   \textbf{68.95}&   84.51&   71.95&   77.47& 75.72\\
ch4.4&      74.60&   76.21&   77.75&   76.19&   \textbf{72.99}&   88.37&   \textbf{73.25}&   80.17&   \textbf{78.69}&   79.51&   76.01&   67.48&   60.18&   70.80&   69.93&   85.46&   65.42&   77.37& 74.54\\
ch5.5&      75.92&   76.68&   75.41&   76.00&   73.60&   87.49&   75.10&   81.23&   79.36&   \textbf{78.80}&   75.99&   69.01&   60.41&   71.05&   71.39&   85.86&   67.06&   77.14& 75.36\\\cdashline{1-20}[2.25pt/3pt]
db2&        \textbf{71.80}&   \textbf{73.24}&   73.16&   \textbf{72.73}&   73.82&   \textbf{86.79}&   75.68&   81.25&   79.38&   80.77&   76.34&   67.99&   60.28&   71.34&   70.41&   \textbf{83.63}&   65.64&   76.41& \textbf{74.02}\\
db3&        75.77&   76.78&   76.74&   76.43&   73.77&   88.69&   76.30&   81.03&   79.94&   80.67&   77.12&   70.22&   60.68&   72.17&   72.34&   85.61&   \textbf{64.53}&   81.27& 75.94\\
db4&        78.21&   79.46&   79.19&   78.96&   73.51&   88.68&   76.80&   81.70&   80.17&   79.16&   77.38&   69.90&   61.79&   72.06&   71.75&   84.77&   73.90&   79.91& 77.58\\
db5&        72.82&   73.58&   \textbf{73.06}&   73.15&   75.88&   88.75&   80.86&   84.83&   82.58&   80.36&   77.29&   70.71&   62.33&   72.67&   72.48&   85.18&   66.46&   80.59& 76.18\\
db6&        80.91&   81.98&   83.17&   82.02&   76.35&   91.06&   81.37&   83.92&   83.18&   82.25&   79.69&   70.77&   63.35&   74.02&   72.93&   87.84&   75.06&   88.55& 81.09\\\hline
	\end{tabular}}
	\end{center}
\end{table*}
\begin{table*}[!t]
	\scriptsize
	%\small
	\caption{Corruption Error (CE) of WResNet50 on ImageNet-C (lower is better).}\vspace{0pt}
	\label{Tab_mCE_ResNet50}
	\begin{center}
	\setlength{\tabcolsep}{0.75mm}{
	\begin{tabular}{r|cccc|ccccc|ccccc|ccccc}\hline
		& \multicolumn{4}{c|}{Noise}& \multicolumn{5}{c|}{Blur}& \multicolumn{5}{c|}{Weather}& \multicolumn{5}{c}{Digital}\\\cline{2-20}
		& Gauss&Shot&Impulse&mCE&Defocus&Glass&Motion&Zoom&mCE&Snow&Frost&Fog&Bright&mCE&Contrast&Elastic&Pixel&Jpeg&mCE\\\hline
baseline&  79.77&   81.57&   82.58&   81.31&   74.71&   88.61&   78.03&   79.86&   80.30&    \textbf{77.83}&   74.84&   \textbf{66.11}&   \textbf{56.64}&   \textbf{68.85}&   71.43&   84.75&   76.92&   76.82&  77.48\\\cdashline{1-20}[2.25pt/3pt]
haar&      77.41&   78.80&   79.22&   78.48&   71.00&   86.38&   76.80&   77.18&   77.84&    80.22&   74.73&   66.18&   57.23&   69.59&   \textbf{70.90}&   84.06&   75.07&   76.51&  76.64\\
ch2.2&     76.08&   77.24&   77.28&   76.87&   71.92&   85.95&   77.54&   77.26&   78.17&    79.24&   75.02&   69.26&   58.44&   70.49&   72.25&   84.63&   68.18&   75.86&  75.23\\
ch3.3&     74.17&   75.63&   75.31&   75.04&   71.67&   86.49&   77.74&   77.89&   78.45&    80.67&   75.50&   66.44&   57.99&   70.15&   71.34&   84.87&   65.61&   \textbf{74.01}&  73.96\\
ch4.4&     76.09&   77.38&   76.72&   76.73&   72.00&   87.03&   77.62&   78.47&   78.78&    79.13&   75.30&   68.80&   57.31&   70.13&   72.03&   85.27&   71.17&   75.80&  76.07\\
ch5.5&     \textbf{71.49}&   \textbf{73.04}&   \textbf{71.70}&   \textbf{72.08}&   72.77&   86.09&   77.61&   77.45&   78.48&    78.55&   \textbf{74.00}&   67.82&   57.48&   69.46&   71.94&   85.99&   74.05&   75.88&  76.97\\\cdashline{1-20}[2.25pt/3pt]
db2&       78.64&   79.23&   78.51&   78.80&   \textbf{69.15}&   \textbf{85.08}&   \textbf{74.56}&   \textbf{76.80}&   \textbf{76.40}&    79.15&   74.96&   68.01&   57.76&   69.97&   71.05&   \textbf{82.56}&   \textbf{60.67}&   78.54&  \textbf{73.20}\\
db3&       78.74&   79.93&   79.36&   79.34&   70.71&   86.92&   76.26&   78.45&   78.09&    78.32&   76.12&   67.07&   57.44&   69.74&   72.04&   87.17&   70.70&   82.13&  78.01\\
db4&       77.16&   78.62&   78.19&   77.99&   73.74&   88.97&   80.20&   79.88&   80.70&    79.74&   76.18&   69.52&   59.29&   71.18&   73.49&   87.84&   74.10&   75.27&  77.67\\
db5&       77.46&   78.80&   78.74&   78.33&   75.36&   89.05&   78.68&   81.08&   81.04&    81.12&   77.97&   71.87&   61.07&   73.01&   74.26&   85.81&   73.96&   84.13&  79.54\\
db6&       79.23&   79.87&   80.23&   79.78&   77.25&   90.20&   82.20&   82.36&   83.00&    82.76&   79.86&   74.50&   64.29&   75.35&   77.66&   88.45&   81.67&   86.14&  83.48\\\hline
	\end{tabular}}
	\end{center}
\end{table*}
\begin{table*}[!t]
	\scriptsize
	%\small
	\caption{Corruption Error (CE) of WResNet101 on ImageNet-C (lower is better).}\vspace{0pt}
	\label{Tab_mCE_ResNet101}
	\begin{center}
	\setlength{\tabcolsep}{0.75mm}{
	\begin{tabular}{r|cccc|ccccc|ccccc|ccccc}\hline
		& \multicolumn{4}{c|}{Noise}& \multicolumn{5}{c|}{Blur}& \multicolumn{5}{c|}{Weather}& \multicolumn{5}{c}{Digital}\\\cline{2-20}
		& Gauss&Shot&Impulse&mCE&Defocus&Glass&Motion&Zoom&mCE&Snow&Frost&Fog&Bright&mCE&Contrast&Elastic&Pixel&Jpeg&mCE\\\hline
baseline&  73.59&   75.31&   76.93&   75.28&   67.98&   81.58&   70.86&   74.17&    73.65&    73.26&   70.50&   62.07&   53.40& 64.81&  66.83&   77.23&   64.76&   67.11&  68.98\\\cdashline{1-20}[2.25pt/3pt]
haar&      70.33&   70.95&   70.10&   70.46&   \textbf{62.93}&   80.93&   \textbf{64.83}&   72.97&    \textbf{70.41}&    71.54&   67.27&   59.94&   50.46& 62.30&  \textbf{62.23}&   76.24&   57.39&   68.25&  66.03\\
ch2.2&     \textbf{64.25}&   \textbf{65.91}&   \textbf{65.04}&   \textbf{65.06}&   63.57&   \textbf{80.35}&   68.22&   \textbf{71.75}&    70.97&    71.55&   67.45&   60.21&   50.13& 62.33&  62.89&   \textbf{74.64}&   \textbf{52.33}&   67.96&  \textbf{64.46}\\
ch3.3&     69.32&   70.91&   69.24&   69.82&   63.78&   81.02&   71.07&   72.00&    71.97&    71.46&   68.60&   60.73&   51.36& 63.04&  64.02&   78.16&   59.05&   \textbf{64.48}&  66.42\\
ch4.4&     67.70&   69.30&   69.71&   68.91&   65.24&   81.05&   69.61&   72.36&    72.07&    71.75&   \textbf{67.18}&   60.10&   50.64& 62.41&  63.47&   77.76&   63.64&   66.96&  67.96\\
ch5.5&     69.67&   71.00&   70.21&   70.30&   64.22&   82.00&   70.15&   74.12&    72.62&    \textbf{71.10}&   67.21&   \textbf{59.07}&   \textbf{50.07}& \textbf{61.86}&  62.31&   78.53&   59.16&   65.01&  66.25\\\cdashline{1-20}[2.25pt/3pt]
db2&       69.70&   71.33&   71.25&   70.76&   65.24&   81.50&   73.36&   74.26&    73.59&    73.66&   68.56&   61.58&   50.65& 63.61&  64.40&   75.81&   62.48&   69.27&  67.99\\  \hline
	\end{tabular}}
	\end{center}
\end{table*}
\begin{table*}[!t]
	\scriptsize
	%\small
	\caption{Corruption Error (CE) of WDenseNet121 on ImageNet-C (lower is better).}
	\label{Tab_mCE_DenseNet121}
	\begin{center}
	\setlength{\tabcolsep}{0.75mm}{
	\begin{tabular}{r|cccc|ccccc|ccccc|ccccc}\hline
		& \multicolumn{4}{c|}{Noise}& \multicolumn{5}{c|}{Blur}& \multicolumn{5}{c|}{Weather}& \multicolumn{5}{c}{Digital}\\\cline{2-20}
		& Gauss&Shot&Impulse&mCE&Defocus&Glass&Motion&Zoom&mCE&Snow&Frost&Fog&Bright&mCE&Contrast&Elastic&Pixel&Jpeg&mCE\\\hline
baseline&80.79&   82.34&   83.75&   82.29&   76.82&   88.72&   80.54&   82.58&   82.16&  78.24&   74.86&   70.18&   59.50&   70.70&  74.07&   87.39&   74.47&   \textbf{74.57}&   77.62\\\cdashline{1-20}[2.25pt/3pt]
haar&	 77.35&   78.74&   78.91&   78.33&   72.82&   86.99&   79.46&   80.04&   79.83&  78.64&   74.61&   67.17&   58.44&   69.72&  70.85&   \textbf{84.16}&   75.72&   77.12&   76.96\\
ch2.2&	 76.15&   77.07&   77.69&   76.97&   72.07&   87.21&   78.04&   80.84&   79.54&  79.85&   73.58&   66.23&   \textbf{57.60}&   69.32&  69.54&   86.15&   74.56&   77.34&   76.90\\
ch3.3&	 77.14&   77.65&   80.15&   78.31&   73.97&   88.14&   78.77&   80.65&   80.38&  77.78&   74.63&   67.03&   58.50&   69.48&  72.12&   85.84&   72.26&   75.44&   \textbf{76.42}\\
ch4.4&	 \textbf{75.26}&   \textbf{76.38}&   \textbf{76.39}&   \textbf{76.01}&   \textbf{71.78}&   \textbf{86.93}&   78.42&   \textbf{79.67}&   \textbf{79.20}&  77.52&   73.57&   66.06&   58.24&   68.85&  \textbf{68.66}&   85.06&   78.18&   79.28&   77.79\\
ch5.5&	 75.45&   76.49&   76.86&   76.27&   73.27&   87.62&   \textbf{77.80}&   81.31&   80.00&  \textbf{76.13}&   \textbf{72.75}&   66.17&   58.25&   \textbf{68.32}&  70.43&   85.36&   73.98&   79.51&   77.32\\\cdashline{1-20}[2.25pt/3pt]
db2&	 79.14&   79.52&   80.80&   79.82&   72.77&   86.98&   78.21&   81.21&   79.79&  78.23&   74.30&   \textbf{65.03}&   57.95&   68.88&  69.83&   85.96&   \textbf{69.29}&   81.04&   76.53\\\hline
	\end{tabular}}
	\end{center}
\end{table*}
\begin{figure}[bpt]
	\centering
	\includegraphics*[scale=0.6, viewport=23 4 416 320]{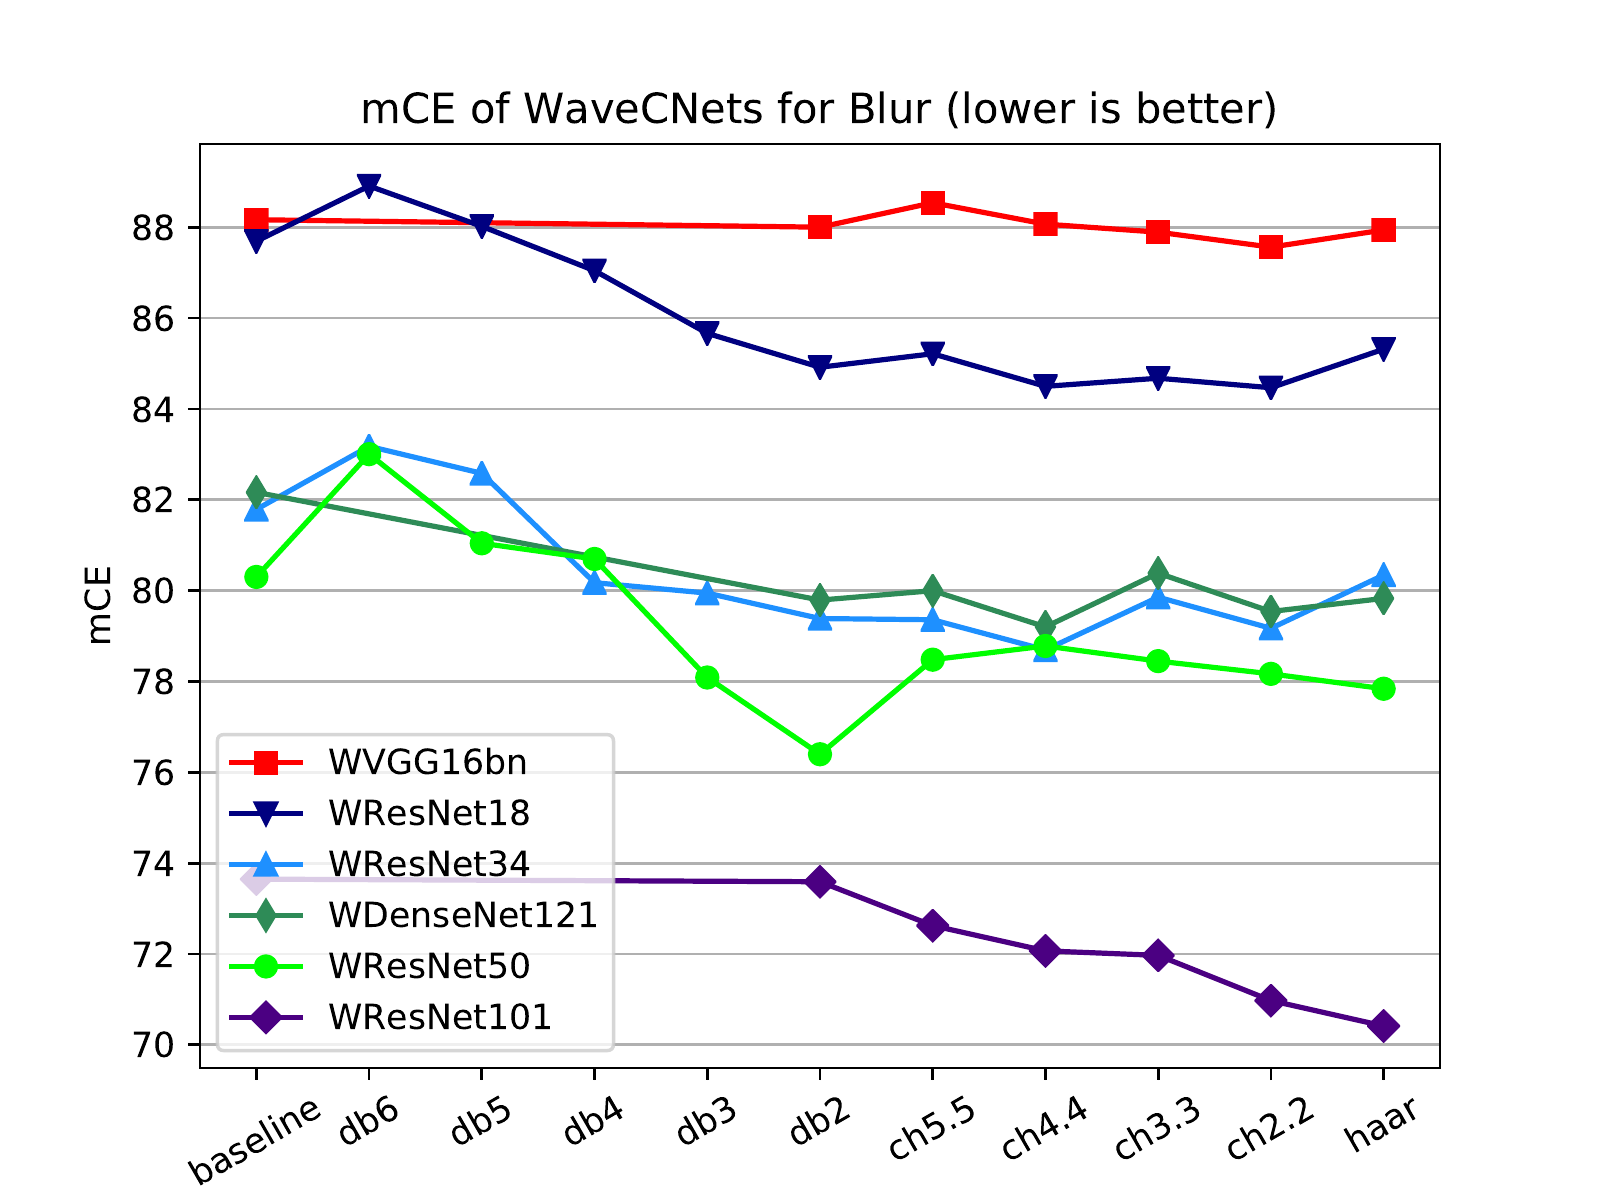}
	\caption{The blur mCE of WaveCNets.}
	\label{fig_mCE_blur}
\end{figure}
\begin{figure}[bpt]
	\centering
	\includegraphics*[scale=0.6, viewport=23 4 416 320]{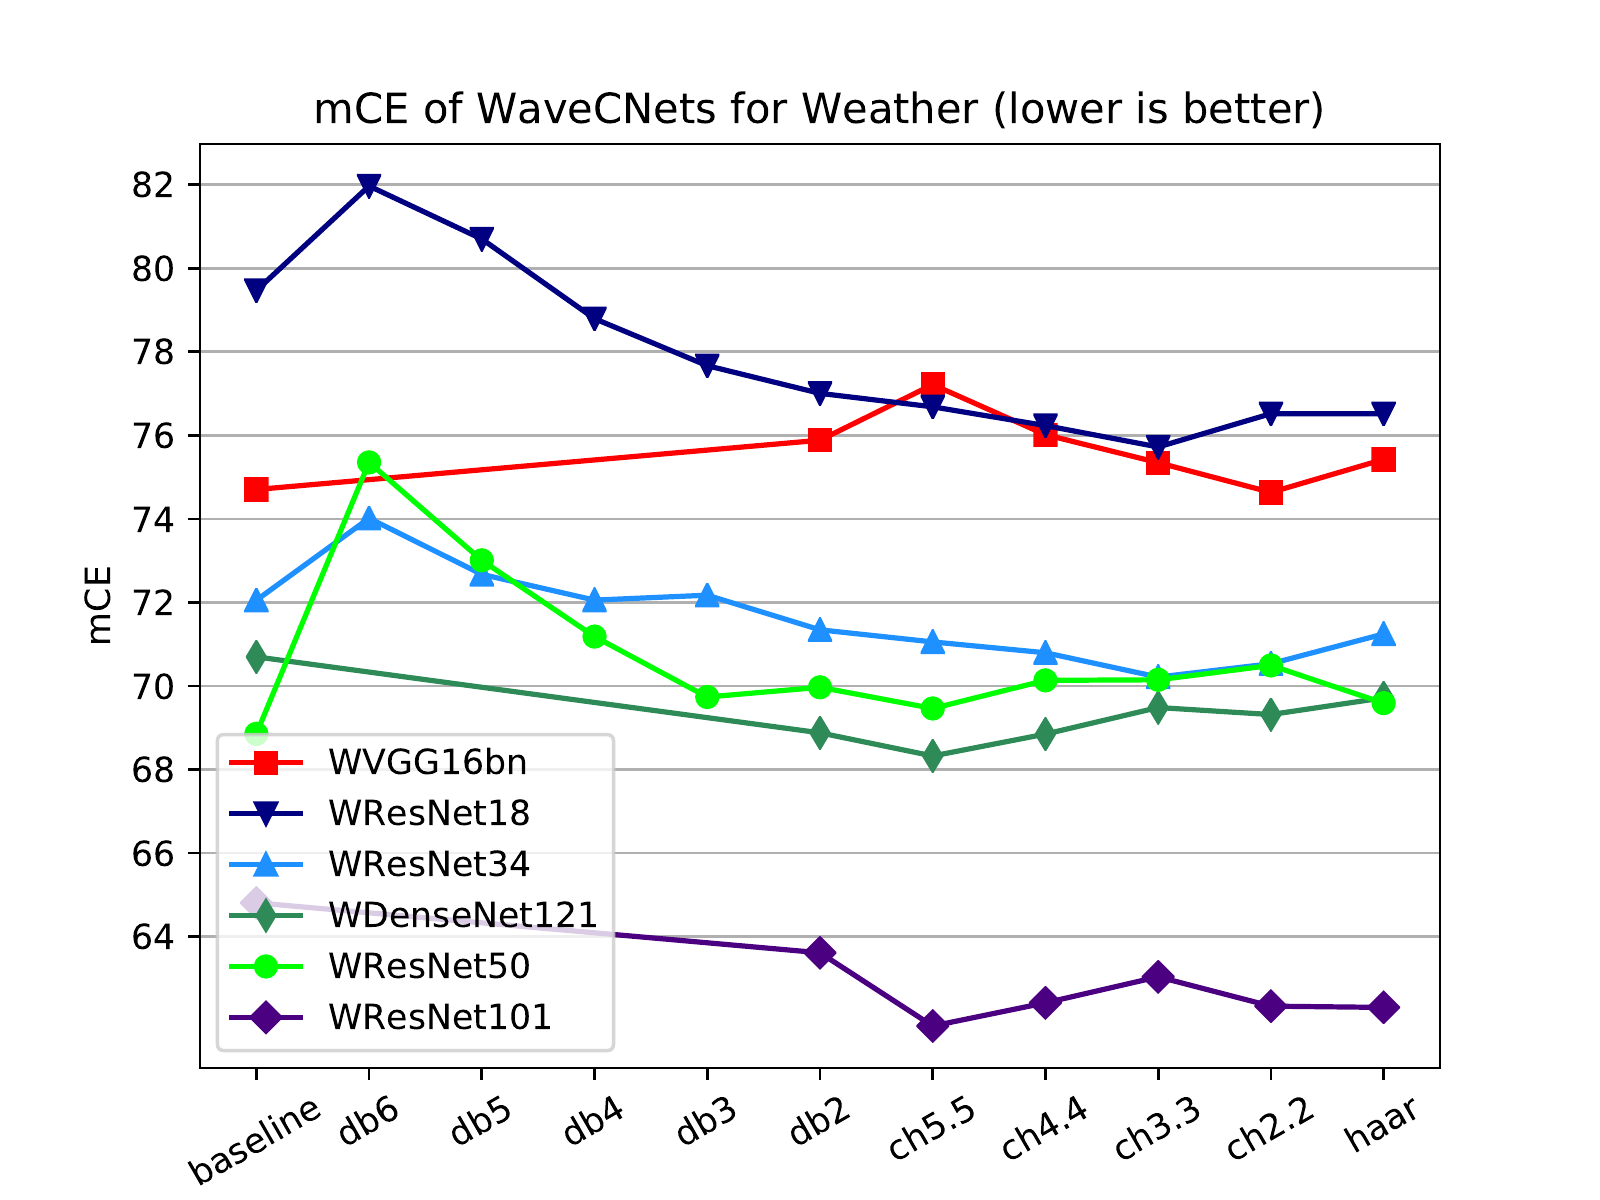}
	\caption{The weather mCE of WaveCNets.}
	\label{fig_mCE_weather}
\end{figure}
\begin{figure}[bpt]
	\centering
	\includegraphics*[scale=0.6, viewport=23 4 416 320]{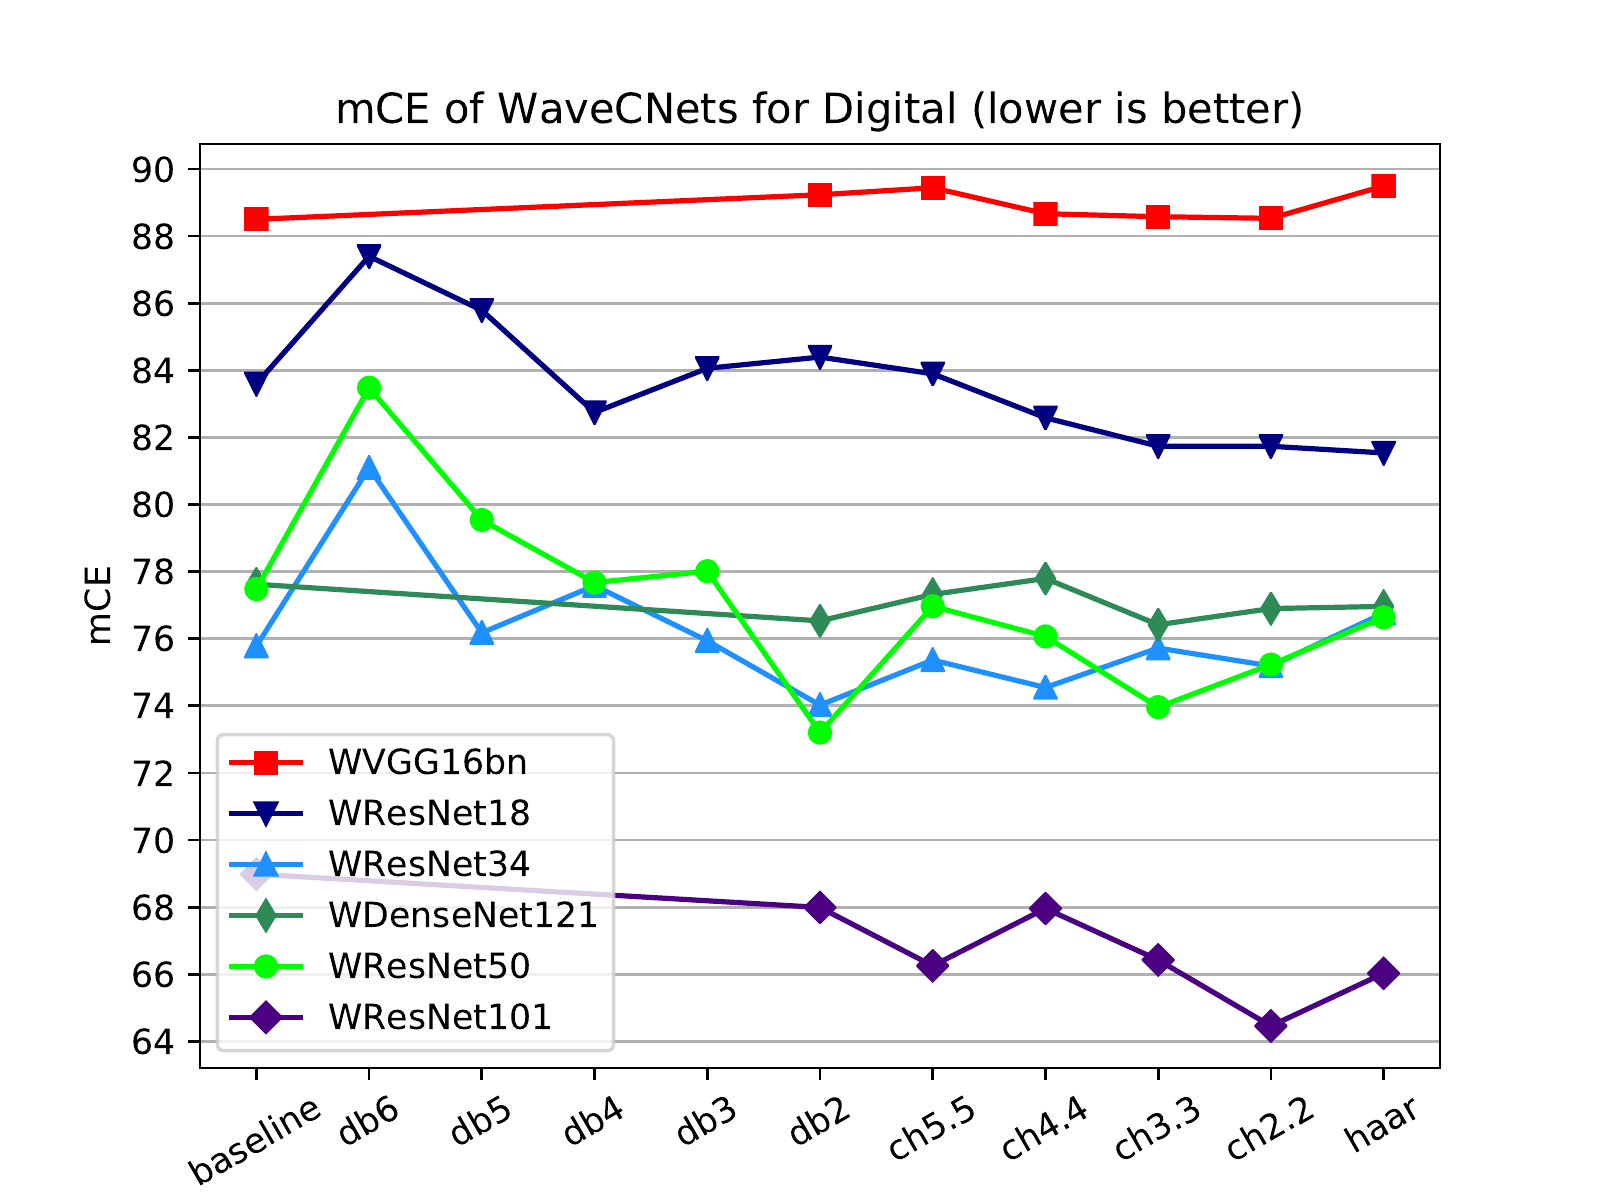}
	\caption{The digital mCE of WaveCNets.}
	\label{fig_mCE_digital}
\end{figure}

ImageNet-C is proposed in \cite{hendrycks2019benchmarking} to evaluate the robustness of a well-trained classifier to the common corruptions.
ImageNet-C contains various versions of ImageNet validation images produced with 15 visual corruptions with five severity levels.
We test WaveCNets on ImageNet-C, and compute the 15 CE values according to Eq. (\ref{eq_CE}).
Because the 15 corruptions are sourced form four categories,
i.e., noise (Gaussian noise, shot noise, impulse noise), blur (defocus blur, frosted glass blur, motion blur, zoom blur),
weather (snow, frost, fog, brightness), and digital (contrast, elastic, pixelate, JPEG-compression),
we compute four mCE according to Eq. (\ref{eq_mCE_noise}) and
\begin{align}
\label{eq_mCE_blur}
\text{mCE}_{\text{blur}}^f &= \dfrac{1}{4}\sum_{ c\in  \{\text{defocus},\ \text{glass}, \atop \quad\text{motion},\ \text{zoom}\}} \text{CE}_c^f,
\end{align}
\begin{align}
\label{eq_mCE_weather}
\text{mCE}_{\text{weather}}^f &= \dfrac{1}{4}\sum_{ c\in  \{\text{snow},\ \text{frost}, \atop \quad\text{fog},\ \text{bright}\}} \text{CE}_c^f,
\end{align}
\begin{align}
\label{eq_mCE_digital}
\text{mCE}_{\text{digital}}^f &= \dfrac{1}{4}\sum_{ c\in  \{\text{contrast},\ \text{elastic}, \atop \quad\text{pixel},\ \text{jpeg}\}} \text{CE}_c^f.
\end{align}

Table \ref{Tab_mCE_VGG16bn} - Table \ref{Tab_mCE_DenseNet121} present the detailed CE and mCE results for
WVGG16bn, WResNet18, WResNet34, WResNet50, WResNet101, WDenseNet121, respectively.
In these tables, the ``baseline'' corresponds to the results of original CNN architecture,
while ``haar'', ``chx.y'', and ``dbx'' correspond to the results of WaveCNets with different wavelets.
From these tables, one can find the robustness of various CNN architectures for corruption Noise
have been improved after the wavelets are integrated,
although the best wavelet varies with the architecture.
However, for corruption Blur, Weather, and Digital, wavelets do not evidently improve the robustness of the CNN architectures 
as what they do for the corruption Noise.
Fig. \ref{fig_mCE_blur}, Fig. \ref{fig_mCE_weather}, and Fig. \ref{fig_mCE_digital} 
show the mCE curves of every architecture for the three corruptions, respectively.
The corruption Blur, Weather, and Digital tend to damage the low-frequency component of the image,
which oppose the application of DWT in suppressing the aliasing effects in deep networks.

\subsection*{D. More discussion about wavelet based noise-robustness improvement}
%\begin{figure}[bpt]%
%	\centering
%	\includegraphics*[scale=0.7, viewport=265 308 585 402]{figures/Visio-down_sampling_of_dwt.pdf}
%	\caption{The general denoising approach using wavelet.}
%	\label{fig_general_denoising_way}
%\end{figure}
\begin{table*}[!t]
	\scriptsize
	\caption{Noise mCE of WaveCNets with different versions of input data (lower is better).}
	\label{Tab_mCE_noise_different_versions}
	\begin{center}
	\begin{threeparttable}
	\setlength{\tabcolsep}{1.25mm}{
	\begin{tabular}{cc||cc||cc||cc||cc||cc||cc}\hline
	\multicolumn{2}{c||}{\multirow{2}{*}{Wavelet}}&\multicolumn{2}{c||}{WVGG16bn} &\multicolumn{2}{c||}{WResNet18}
	&\multicolumn{2}{c||}{WResNet34}&\multicolumn{2}{c||}{WResNet50}&\multicolumn{2}{c||}{WResNet101}&\multicolumn{2}{c}{WDenseNet121} \\\cline{3-14}
	&&noisy\tnote{b}& denoised\tnote{c}&noisy & denoised&noisy & denoised&noisy & denoised&noisy & denoised&noisy & denoised\\\hline\hline
\multicolumn{2}{c||}{None (baseline)\tnote{a}}&               87.62&     86.76&     88.97&    87.77&     83.10&    81.52&      81.31&    79.45&     75.28&    73.72&     82.29&  80.92\\\hline
\multicolumn{2}{c||}{Haar}                    &               87.43&     85.93&     80.91&    79.68&     76.63&    75.62&      78.48&    77.18&     70.46&    68.50&     78.33&  77.02\\\hline
{\multirow{4}{*}{Cohen}}&\multicolumn{1}{|c||}{ch2.2}    &    87.79&     86.18&     80.38&    \textbf{78.93}&     77.61&    75.98&      76.87&    75.84&     65.06&    \textbf{64.01}&     76.97&  76.19\\
&\multicolumn{1}{|c||}{ch3.3}                 &               88.28&     87.58&     81.02&    79.80&     74.30&    73.26&      75.04&    73.42&     69.82&    68.46&     78.31&  76.88\\
&\multicolumn{1}{|c||}{ch4.4}                 &               85.63&     \textbf{84.67}&     82.19&    80.66&     76.19&    74.70&      76.73&    75.05&     68.91&    67.62&     76.01&  \textbf{74.84}\\
&\multicolumn{1}{|c||}{ch5.5}                 &               89.84&     88.70&     83.77&    81.97&     76.00&    74.09&      72.08&    \textbf{70.99}&     70.30&    68.90&     76.27&  75.18\\\hline
{\multirow{5}{*}{Daubechies}}&\multicolumn{1}{|c||}{db2} &    87.44&     85.97&     82.54&    81.23&     72.73&    \textbf{71.45}&      78.80&    77.21&     70.76&    68.82&     79.82&  78.69\\
&\multicolumn{1}{|c||}{db3}	                  &                    &          &     83.92&    82.02&     76.43&    74.83&      79.34&    77.31&          &         &          &       \\
&\multicolumn{1}{|c||}{db4}	                  &                    &          &     86.23&    84.32&     78.96&    77.39&      77.99&    76.85&          &         &          &       \\
&\multicolumn{1}{|c||}{db5}	                  &                    &          &     85.47&    83.92&     73.15&    72.03&      78.33&    77.16&          &         &          &       \\
&\multicolumn{1}{|c||}{db6}	                  &                    &          &     86.57&    84.76&     82.02&    80.06&      79.78&    78.61&          &         &          &       \\\hline
			\end{tabular}}
		\begin{tablenotes}
			\item[a] corresponding to the results of original CNNs without down-sampling upgrading, i.e., VGG16bn, ResNets, DenseNet121.
			\item[b] taking original corrupted images in noise part of ImageNet-C as input.
			\item[c] taking the denoised version of images in noise part of ImageNet-C as input.
		\end{tablenotes}
	\end{threeparttable}
	\end{center}
\end{table*}

The noisy images in ImageNet-C are generated by adding various noises into the original images.
Therefore, a natural way to decrease classification error of a classifier on the ImageNet-C
is to denoise the noisy images before feeding them into the classifier.

The random noises are mostly presented in high-frequency components.
Therefore, as Fig. \ref{fig_denoise_a} shows,
the general wavelet based denoising method \cite{donoho1995noising,donoho1994ideal} composes of three steps:
decompose the noisy image $\textbf{X}$ into various frequency components using DWT,
filter the high-frequency components $\textbf{X}_{lh}, \textbf{X}_{hl}, \textbf{X}_{hh}$ using denoising operations,
and reconstruct the image using the processed components with IDWT.
In high-frequency components, the noises are usually presented by the smaller coefficients.
Thus, the usual denoising operation is to choose threshold $\lambda$ and reset coefficients smaller than the threshold to zero.
Here, we choose the soft threshold filtering operations presented in Eq. (\ref{eq_hard_threshold}),
to process every coefficient $x$ in high-frequency components $\textbf{X}_{lh}, \textbf{X}_{lh}, \textbf{X}_{hh}$.
\begin{align}
\label{eq_hard_threshold}
\text{SoftShrinkage}(x) = \begin{cases}
        x - \lambda, & \text{ if } x > \lambda, \\
        x + \lambda, & \text{ if } x < -\lambda, \\
        0, & \text{otherwise}.
        \end{cases}
\end{align}
In wavelet based denoising field, the noisy image would be processed by multiple levels of DWT and IDWT.
Various threshold parameters $\lambda$ or threshold functions $\lambda(x)$ would be selected for the components in different levels.
\begin{figure}[bpt]
	\centering
	\includegraphics*[scale=0.5, viewport=35 21 490 505]{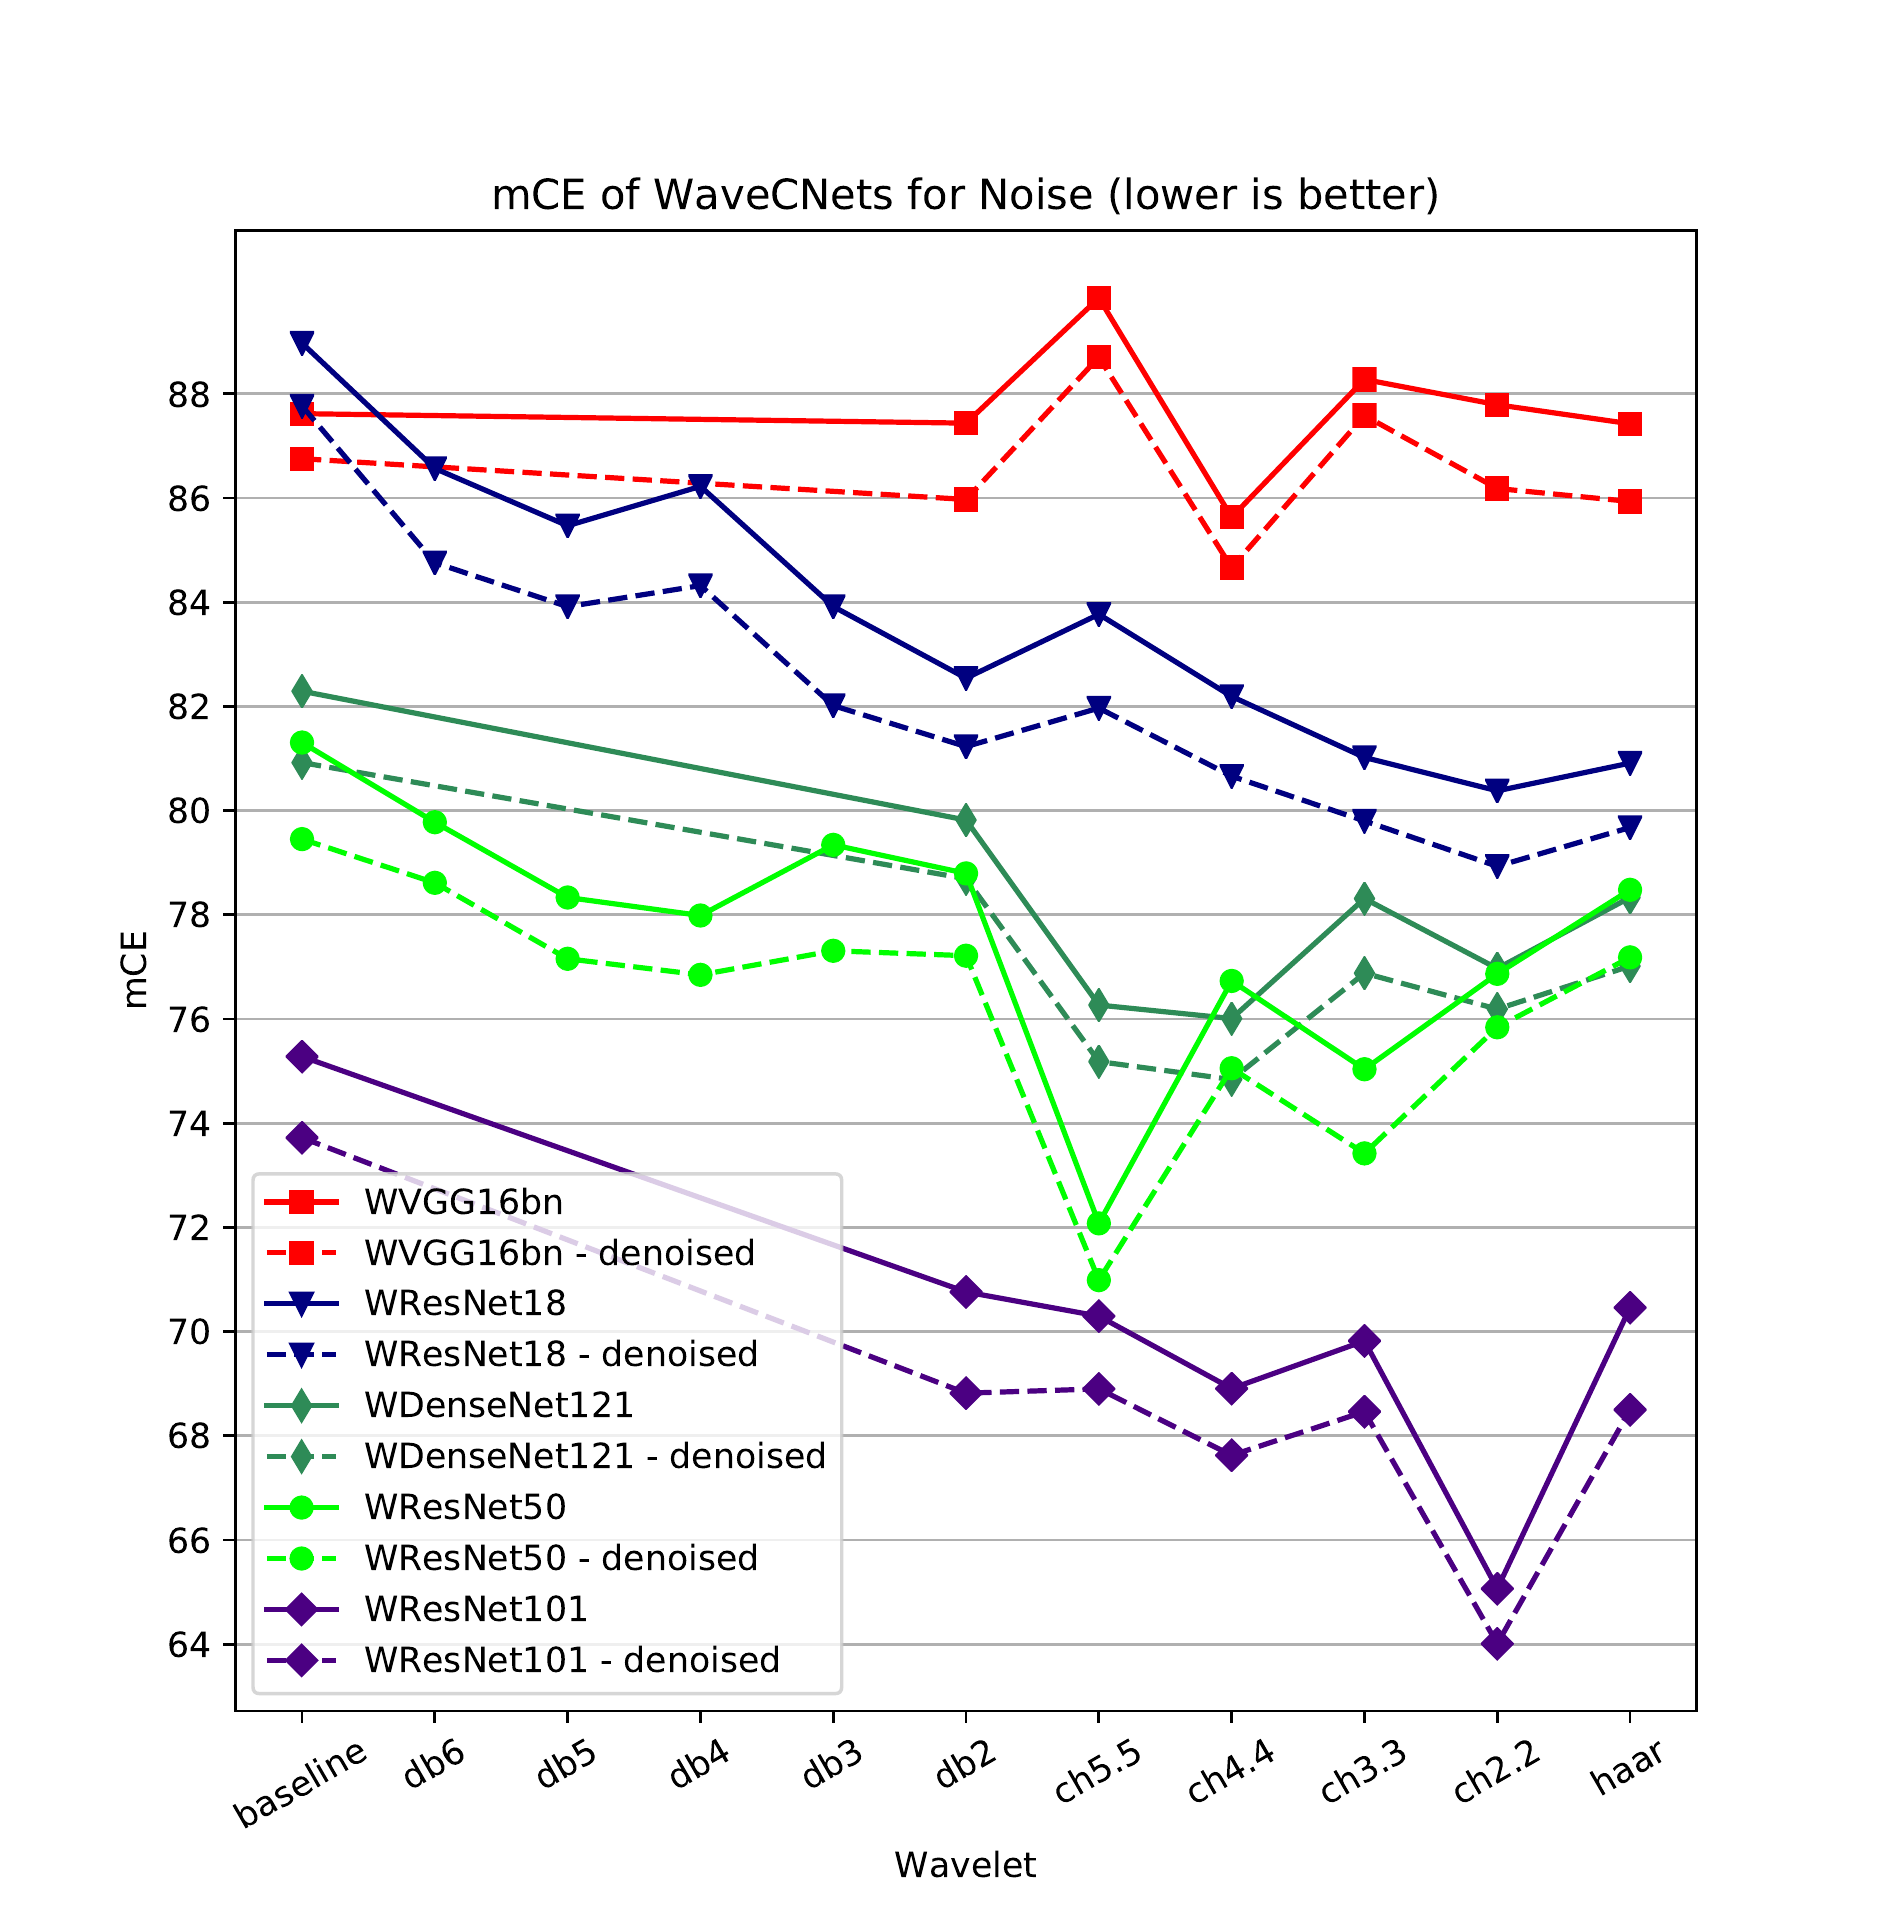}
	\caption{The noise mCE of WaveCNets with different input.}
	\label{fig_mCE_noise_denoise}
\end{figure}

In our experiments, we only do one DWT and IDWT, and set $\lambda = 0.1$.
We feed the denoised images into WaveCNets trained on the clean ImageNet training set.
We get the top-1 errors, and compute the $\text{mCE}_{\text{noise}}^f$
for every WaveCNet $f$ according to Eqs. (\ref{eq_CE}) and (\ref{eq_mCE_noise}).
The detailed results are shown in Table \ref{Tab_mCE_noise_different_versions}.
For better illustration, in Fig. \ref{fig_mCE_noise_denoise},
we plot the noise mCE curves of WaveCNets with different versions of input data.
In Fig. \ref{fig_mCE_noise_denoise}, the noise mCEs for denoised images (dashed lines)
are always lower than that for original noisy images (solid lines).
From Table \ref{Tab_mCE_noise_different_versions} and Fig. \ref{fig_mCE_noise_denoise},
one can find that the denoising method improves the noise-robustness of all CNN architectures,
for the all down-sampling versions including that without DWT.

\subsection*{E. Shift-invariance of WaveCNets}
Besides breaking object structures and accumulating noises,
down-sampling operations may also decrease the shift-invariance of CNNs \cite{azulay2018deep,zhang2019making},
if the down-sampling ignores the classic sampling theorem.
By integrating with low-pass filtering, anti-aliased CNNs \cite{zhang2019making} present increased shift-invariance.
DWT composes filtering and down-sampling, so it could also improve the shift-invariance.

In \cite{zhang2019making}, to evaluate the shift-invariance of a classifier $f$,
the author checks how often the classifier outputs the same predication, given the same image with two different shifts:
\begin{align}
\nonumber
\textbf{E}_{\textbf{X},h_1,w_1,h_0,w_0}\textbf{1}&\{\arg\max P_f(\text{shift}_{h_0,w_0}(\textbf{X})) \\
													&= \arg\max P_f(\text{shift}_{h_1,w_1}(\textbf{X}))\},
\end{align}
where $\textbf{E}$ denotes the expectation.
Using this criterion, we evaluate the shift-invariance of WaveCNets and the original CNNs.
Table \ref{Tab_shift_invariance} presents the results.
\begin{table}
%\scriptsize
\small
\caption{Shift-invariance of WaveCNets (higher is better).}
\label{Tab_shift_invariance}
\begin{center}
\setlength{\tabcolsep}{1.6mm}{
\begin{tabular}{r||c|cccc|c}\hline
\multirow{3}{*}{wavelet}	&\multicolumn{6}{c}{WaveCNet} \\\cline{2-7}
							&VGG & \multicolumn{4}{c|}{ResNet}&DenseNet  \\\cline{2-7}
							&16bn&18&34&50&101&121\\\hline
baseline&    89.24&     85.11&     87.56&      89.20&      89.81&     88.81\\\hline
haar    &    90.54&     86.43&     88.46&      89.93&      90.73&     89.12\\
ch2.2   &    91.03&     87.35&     89.02&      90.01&      91.06&     89.52\\
ch3.3   &    \textbf{91.32}&     \textbf{87.71}&     \textbf{89.11}&      \textbf{90.68}&      91.33&     \textbf{89.91}\\
ch4.4   &    90.68&     87.36&     89.04&      90.22&      \textbf{91.34}&     89.23\\
ch5.5   &    90.56&     86.97&     88.74&      89.94&      91.11&     89.33\\
db2     &    90.84&     86.96&     88.62&      89.69&      91.02&     89.05\\
db3     &         &     86.79&     88.50&      89.72&           &          \\
db4     &         &     86.44&     88.26&      89.47&           &          \\
db5     &         &     85.88&     87.96&      88.86&           &          \\
db6     &         &     84.84&     87.65&      87.87&           &          \\\hline
\end{tabular}}
\end{center}
\end{table}

In Table \ref{Tab_shift_invariance}, the ``baseline'' corresponds to the shift-invariance of original CNN architecture,
while ``haar'', ``chx.y'', and ``dbx'' correspond to the results of WaveCNets with different wavelets.
From Table \ref{Tab_shift_invariance}, WaveCNets improve the robustness to the image shift, compared with their original versions.
Generally, WaveCNets achieve the best shift-invariance using wavelet ``ch3.3''.
However, compared with the results of anti-aliased CNNs shown in \cite{zhang2019making},
the shift-invariance of WaveCNets are somewhat inferior.
We believe that is sourced from the Max operation that WaveCNets drop and anti-aliased CNNs keep.

\begin{figure*}[t]
	\centering
	\includegraphics*[scale=0.8, viewport=43 558 558 710]{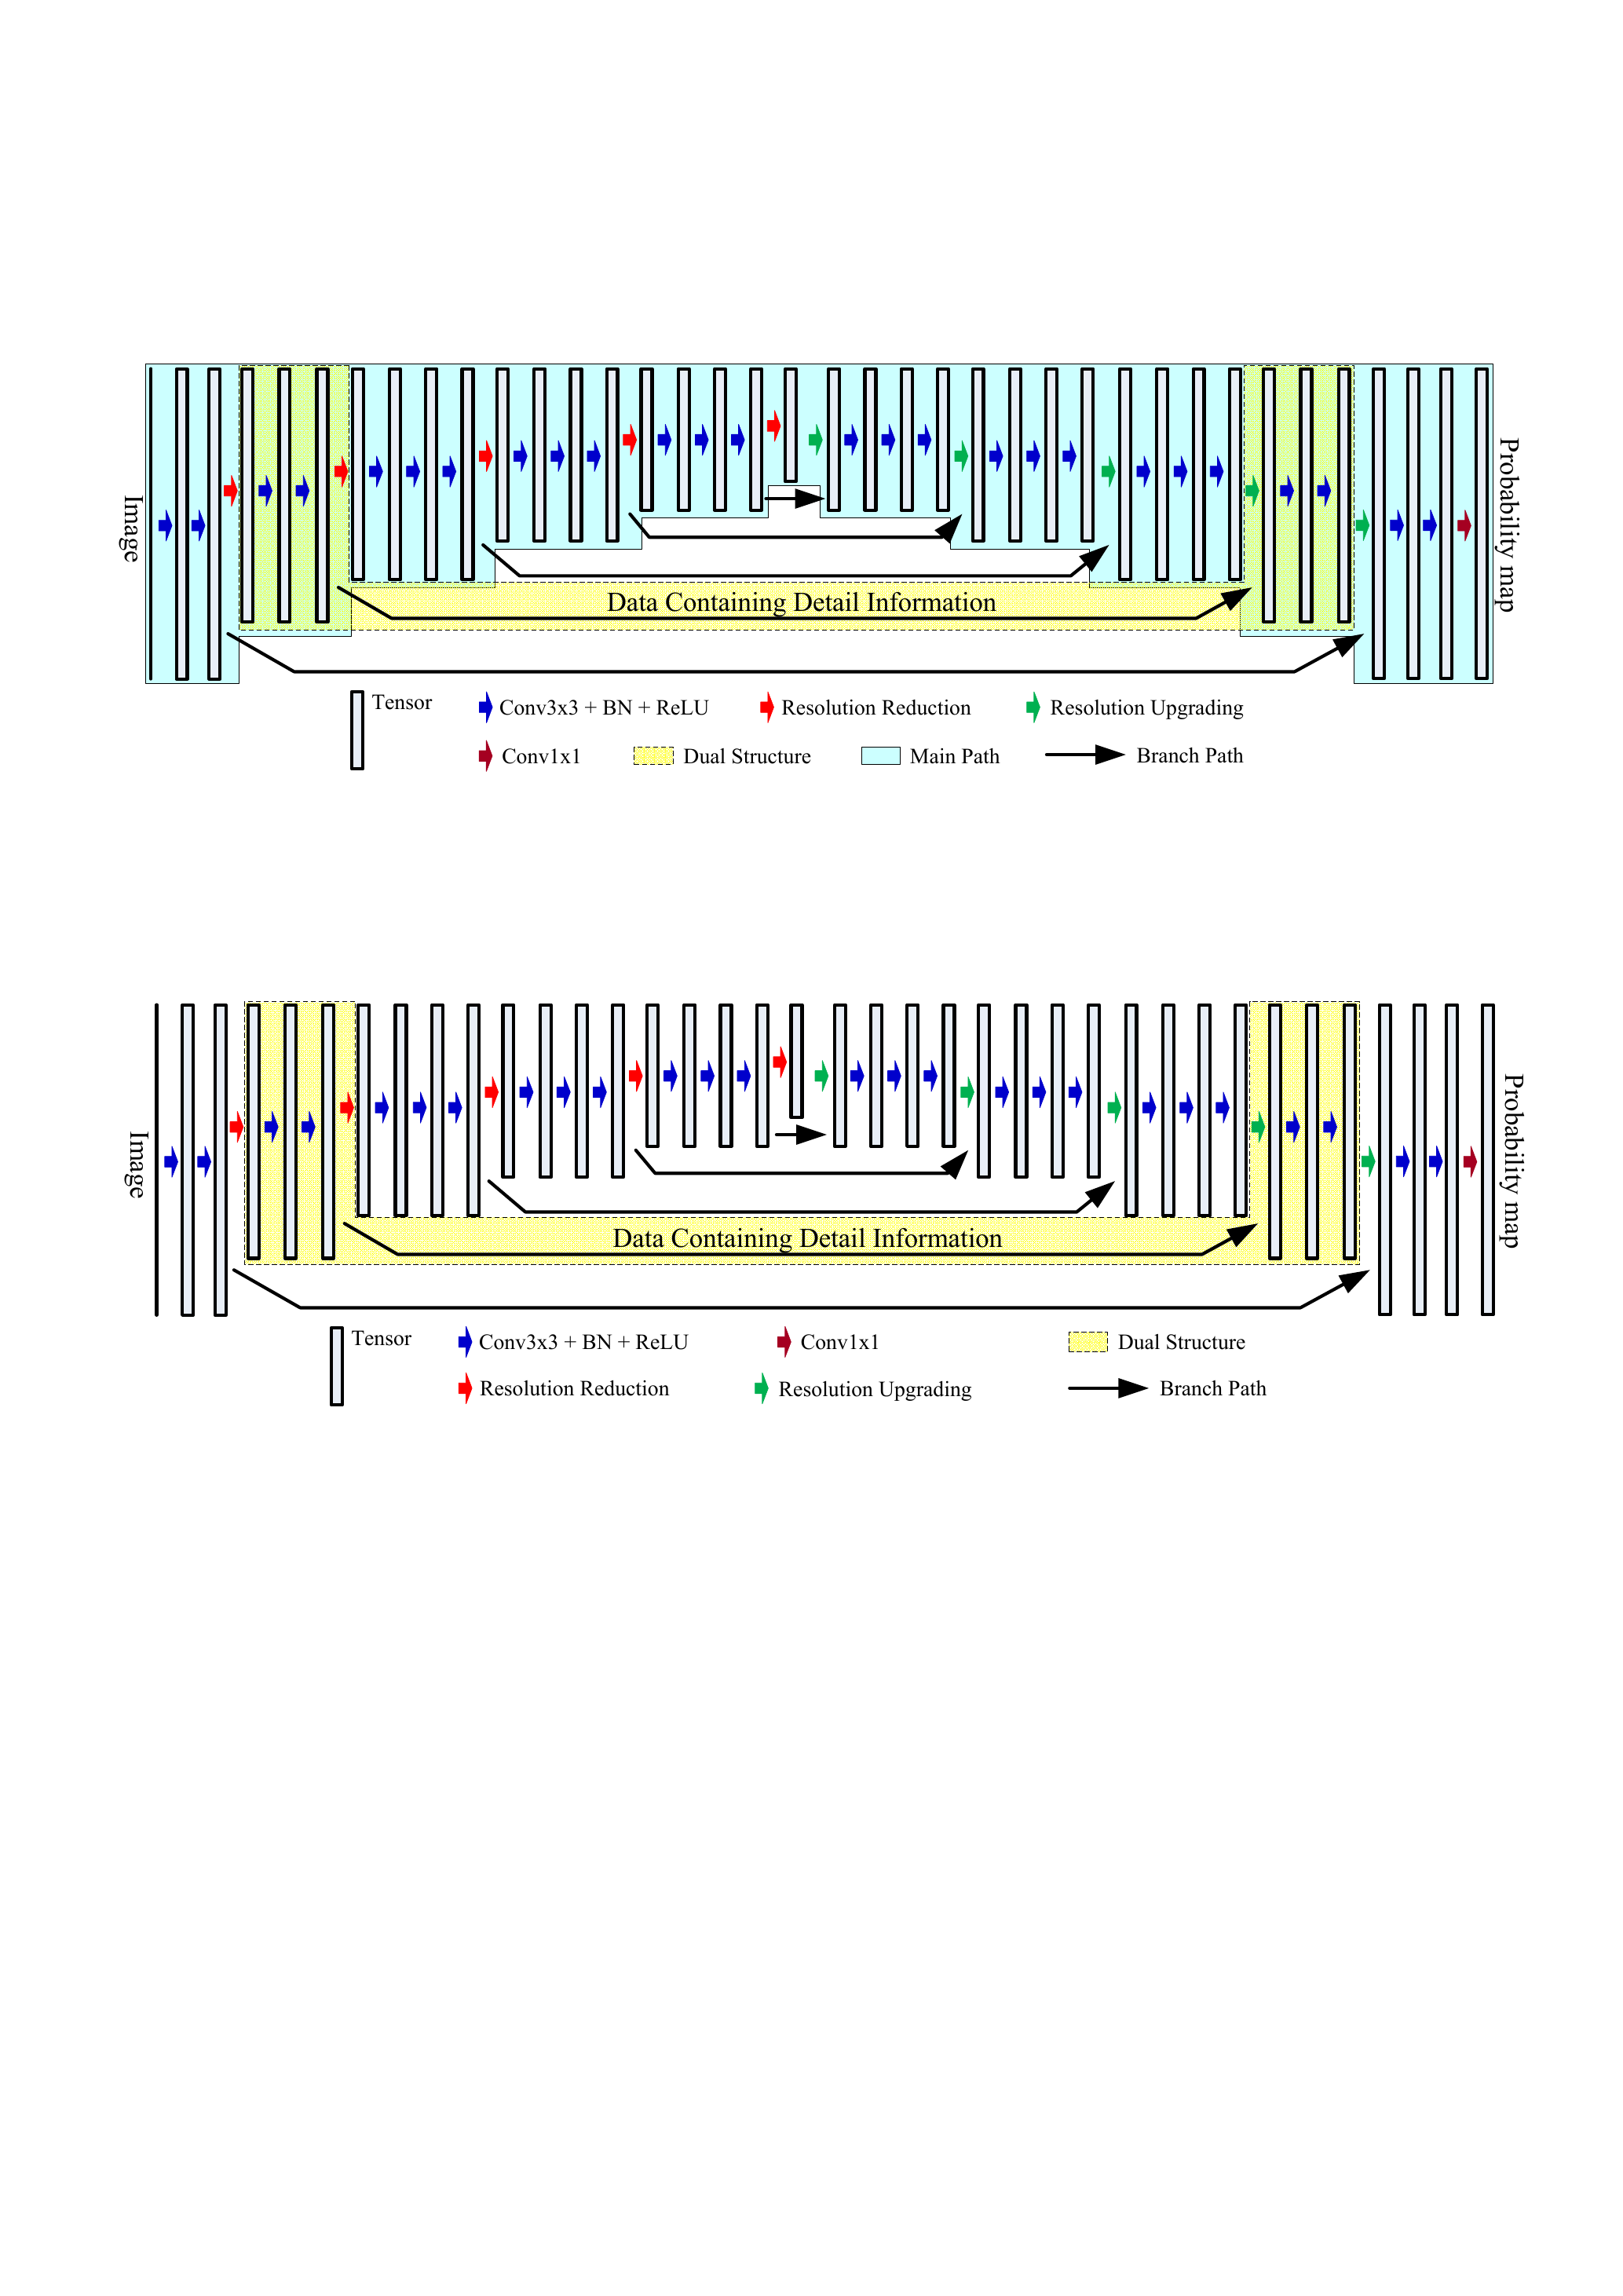}
	\caption{The encoder-decoder architectures.}\label{fig_encoder_decoder}
\end{figure*}
\subsection*{F. The architectures of SegNet and WaveUNets}
SegNet and WaveUNets adopt encoder-decoder architecture, as Fig. \ref{fig_encoder_decoder} shows.
Fig. \ref{fig_dual_structures} shows the down-sampling and up-sampling used in SegNet and WaveUNets.
In the encoder, SegNet down-samples the feature maps using max-pooling, and stores the max-indices.
In its decoder, SegNet recovers the feature map resolution using max-unpooling with the indices,
as Fig. \ref{fig_dual_structure_Pooling_Unpooling} shows.
While max-unpooling only recover very limited details, IDWT can recover most of the data details.
In the encoder, WaveUNets decompose the feature maps into various frequency components, as Fig. \ref{fig_dual_structure_DWT_IDWT} shows.
While the low-frequency components are used to extract high-level features,
the high-frequency components are stored and transmitted to the decoder for resolution restoration with IDWT.

\begin{table}[!t]
	%\scriptsize
	\caption{Deep network configurations.}
	\label{Tab_network_configuration}
	\begin{center}
	\begin{threeparttable}
		\setlength{\tabcolsep}{1.75mm}{
			\begin{tabular}{c||l|r}
				\hline
				\multirow{2}{*}{data size} &    \multicolumn{2}{c}{the number of channels}\\ \cline{2-3}
				                           & \multicolumn{1}{c|}{encoder} & \multicolumn{1}{c}{decoder}\\ \hline
				      $352\times480$       & 3, 64                    &                   64, 64 \\
				      $176\times240$       & 64, 128                  &                  128, 64 \\
				     ~~$88\times120$       & 128, 256, 256            &            256, 256, 128 \\
				       $44\times60$        & 256, 512, 512            &            512, 512, 256 \\
				       $22\times30$        & 512, 512, 512            &            512, 512, 512 \\ \hline
			\end{tabular}}
	\end{threeparttable}
	\end{center}
\end{table}
The encoder of SegNet and WaveUNets consist of 13 convolutional layers
corresponding to the first 13 convolutional layers in the VGG16bn \cite{simonyan2014very}.
Their decoder contains the same number of convolutional layers with the encoder.
Every convolutional layer in the former and the corresponding one in the latter have the same number of channels,
except the first and the last one of the network.
In the encoder and decoder, a Batch Normalization (BN) and Rectified Linear Unit (ReLU) are implemented after every convolution.
A convolutional layer with kernel size of $1\times1$ converts the output of decoder into the predicted segmentation result,
as shown in Fig. \ref{fig_encoder_decoder}.
In Table \ref{Tab_network_configuration}, the first column shows the input size,
though these networks can process images with arbitrary size.
Every number in the table corresponds to a convolutional layer with BN and ReLU.
While the number in the column ``encoder'' is the number of the input channels of the convolution,
the number in the column ``decoder'' is the number of the output channels.

\subsection*{G. The amount of multiply-adds in 2D DWT/IDWT}
Given a 2D tensor $\textbf{X}$ with size of $M\times N$ and channel $C$,
the amount of multiply-adds used in 2D DWT inference is
\begin{align}
\label{eq_no_2D_DWT}
4C\left(M^2N+\dfrac{MN^2}{2} - \dfrac{3MN}{4}\right),
\end{align}
and the amount of multiply-adds used in 2D IDWT inference is
\begin{align}
\label{eq_no_2D_IDWT}
4C\left(MN^2+\dfrac{M^2N}{2} - \dfrac{3MN}{4}\right) + 3,
\end{align}
according to Eqs. (\ref{eq_DWT_2D_M_ll}) - Eqs. (\ref{eq_DWT_2D_M_hh}).

Table \ref{Tab_ratio_wavelet_convolution} presents
the ratios of wavelet related multiply-adds over the total operations for WaveCNets and WaveUNets,
when the input size is $3\times224\times224$.
We only count the amount of multiply-adds in $\text{DWT}_{ll}$ for WaveCNets.
\begin{table}
\scriptsize
\caption{Wavelet related operation ratios.}
\label{Tab_ratio_wavelet_convolution}
\begin{center}
\setlength{\tabcolsep}{0.75mm}{
\begin{tabular}{r||c|cccc|c|c}\hline
\multirow{3}{*}{}	&\multicolumn{6}{c|}{WaveCNet}& {WaveUNet}\\\cline{2-8}
							&VGG & \multicolumn{4}{c|}{ResNet}&DenseNet & VGG\\\cline{2-8}
							&16bn&18&34&50&101&121&16bn\\\hline
non-wavelet ($\times10^9$)&    $15.51$&     $1.82$& $3.67$ &$4.12$&$7.85$ & $2.88$&$30.77$\\\hline
wavelet ($\times10^9$)&    $1.43$&\multicolumn{4}{c|}{$0.22$}&$0.18$&$8.57$\\\hline
ratio ($\%$)   &    $8.44$&     $10.85$&    $5.69$& $5.11$& $2.75$&     $5.82$&$21.78$\\\hline
\end{tabular}}
\end{center}
\end{table}
